# Supplementary material for: Motility-induced buckling and glassy dynamics regulate three-dimensional transitions of bacterial monolayers
Source: arXiv:2003.05618 ancillary file (2020-03-12)
Supplement: Supplementary file 1 [file SI_Bacteria.pdf]

# Motility-induced buckling and glassy dynamics regulate 3D transitions of bacterial monolayers

Sho C. Takatori,[1,2,‡] and Kranthi K. Mandadapu[2,3,†]

[1] Department of Chemical Engineering, University of California, Santa Barbara, CA 93106
[2] Department of Chemical & Biomolecular Engineering, University of California, Berkeley, CA 94720
[3] Chemical Sciences Division, Lawrence Berkeley National Laboratory, CA 94720

This is a supplementary information for the article with the same title.

‡ stakatori@ucsb.edu
† kranthi@berkeley.edu

## TABLE OF CONTENTS

Chapter I. Introduction **2**
1. Experimental observations of bacterial colonies . . . 2
2. Questions . . . 5

Chapter II. Active swarming vs. glassy liquids **7**
1. DF theory for passive colloidal systems . . . 9
2. DF theory for active colloidal systems . . . 10
   2.1 DF theory for active Brownian particles . . . 11
   2.2 Activity and softness . . . 17
3. Swarming and glassy dynamics of active Brownian spherocylinders . . . 18
   3.1 Passive polydisperse spherocylinders . . . 19
   3.2 Active polydisperse spherocylinders . . . 20
   3.3 Swarming behaviors: ABPs vs. Spherocylinders . . . 21
4. DF theory for *P. aeruginosa* colonies . . . 22

Chapter III. Mechanics of bacterial colonies **26**
1. Bacterial colony monolayers as active fluid shells . . . 26
2. Continuum membrane theory . . . 27
   2.1 Differential geometry and kinematics of membranes . . . 27
   2.2 Balance laws for fluid membranes . . . 29
   2.3 Constitutive relations: fluidity, elastic bending and adhesion . . . 31
   2.4 Restrictions to Monge parametrization - small deformations . . . 33
3. Buckling of active bacterial monolayers . . . 35
   3.1 The case of incompressible rotational flow . . . 36
   3.2 The case of imcompressible shear flow . . . 37
   3.3 The case of extensional flow . . . 39
   3.4 The case of nonlinear incompressible squeeze flows . . . 39

3.5 The cases of compressible linear flows . . . . . . . . . . . . . . . . . . . . . . . . . . . 43
4. Molecular simulations to test buckling mechanisms of colonies . . . . . . . . . . . . . . . . . . 47
4.1 Constitutive behavior of 2D polydisperse spherocylinder systems . . . . . . . . . . . 48
4.2 The case of shear flow for passive spherocylinder systems . . . . . . . . . . . . . . . . . 48
4.3 The case of localized shear at an interface for passive spherocylinder systems . . . . 50
5. Role of topological defects in buckling . . . . . . . . . . . . . . . . . . . . . . . . . . . . . . . 51

Chapter IV. Connections to Simulations and Experiments **53**
1. Eigenvalue analysis of spherocylinders under uniform & interfacial shear . . . . . . . . . . 55
2. Eigenvalue analysis of general active colonies . . . . . . . . . . . . . . . . . . . . . . . . . . 55
3. Other experimental observations . . . . . . . . . . . . . . . . . . . . . . . . . . . . . . . . . 59

Chapter V. Supplemental Movies **61**
References . . . . . . . . . . . . . . . . . . . . . . . . . . . . . . . . . . . . . . . . . . . . . . 64

# Chapter I

# INTRODUCTION

## 1. Experimental observations of bacterial colonies

We conduct an under-agar motility assay to analyze the growth of *Pseudomonas aeruginosa* monolayers into three-dimensional (3D) structures. The experimental setup is shown in Fig. 1.1A, using which we track the time trajectory of individual bacteria in the monolayer and one layer above (Fig. 1.1B). Three key experimental observations point towards an interplay between cell density, active motility, and 3D growth of motile bacterial monolayers.

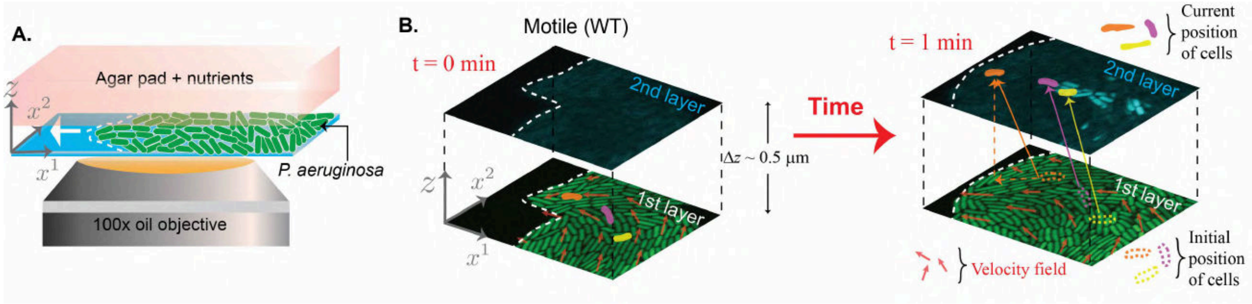


**Figure 1.1:** Motile colonies of *P. aeruginosa* PAO1 transition from a two-dimensional (2D) monolayer into a three-dimensional (3D) architecture. (A) Schematic of under-agar experimental assay for observing confluent bacterial monolayers using confocal microscopy. Time-lapse, z-stack images are taken to observe both first and second bacterial layers. (B) Nucleation events corresponding to 2D to 3D transitions in motile colonies are shown by tracking three bacteria over the course of a minute. Individual bacteria translate in the monolayer by several microns and collide into multiple neighbors before transitioning out of plane. Multiple bacteria appear in the second layer within a minute.

First, wild type colonies exhibit collective swarming motility that is correlated with out-of-plane transitions of individual bacteria from a 2D monolayer into the third dimension. Figure 1.2 is a snapshot of a migrating front of a colony that displays this 2D-to-3D transition; also, see a corresponding SI Movie S1. Complex flows are clearly visible in the colony, and halfway into the video, there is an increase in fluorescence intensity, which indicates that multiple layers of bacteria have formed. Experiments conducted at higher magnification further reveal that these transitions are correlated with unique in-plane flows, as shown in Fig. 1.3 and SI Movies S2 and S3. Highly active complex flows and transition events are especially pronounced at the leading edges of the colony. Given these observations, we hypothesize that in-plane flows are responsible for the out-of-plane transition.

Second, non-motile (pilA mutant) colonies did not exhibit any collective swarms and we did not observe any 3D transitions of bacteria near the leading edges of the colony. Instead, we observe

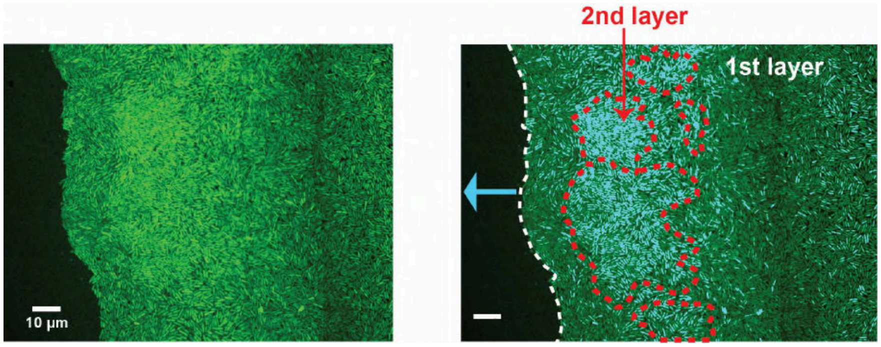


**Figure 1.2:** Left: Snapshot of a confocal image of wild type *P. aeruginosa* colony. Right: The bacteria that have transitioned into a second layer are circled in red dashed lines and pseudo-colored in cyan. See SI Movie S1 for the full video showing the 2D-to-3D transition.

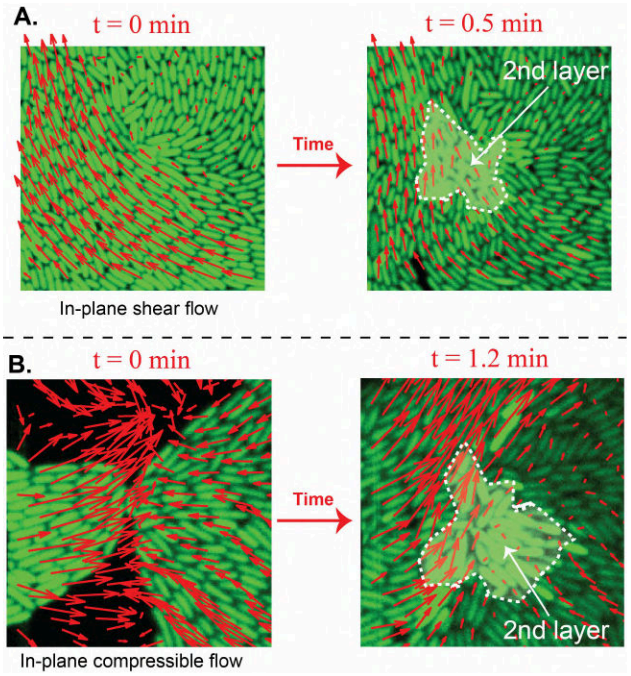


**Figure 1.3:** Confocal images of wild type *P. aeruginosa* colony. (A) Collective swarming of a flock creates an in-plane shear flow that results in out-of-plane transition. (B) Two flocks converging to a single point creates an in-plane compressible flow that results in out-of-plane transition. In both cases, the red arrows are local velocities and white dashed lines denote the bacteria that have displaced out of plane. See SI Movies S2 and S3 for the full video showing the 2D-to-3D transition.

growth into the third dimension only in the colony interiors (Fig. 1.4); also see SI Movies S4 and S5. Nucleation of non-motile bacteria into 3D arises from a known phenomenon of buckling due to cell division and growth-induced stresses [1–7], and occurs on a timescale much larger than the motility-induced transitions that we observe in the wild type strain in the swarming state.

Third and last, colonies prepared at large packing fractions exhibit no collective swarms and the bacteria become kinetically arrested in a glassy-like state; see Fig. 1.5 and SI Movie S7 for a video of a colony in this state. The bacteria are no longer free to translate and rotate as that of a motile colony at low densities, but instead move by distinct, infrequent hopping steps. These 'excitations' do not occur homogeneously across the colony but are focused in specific regions that

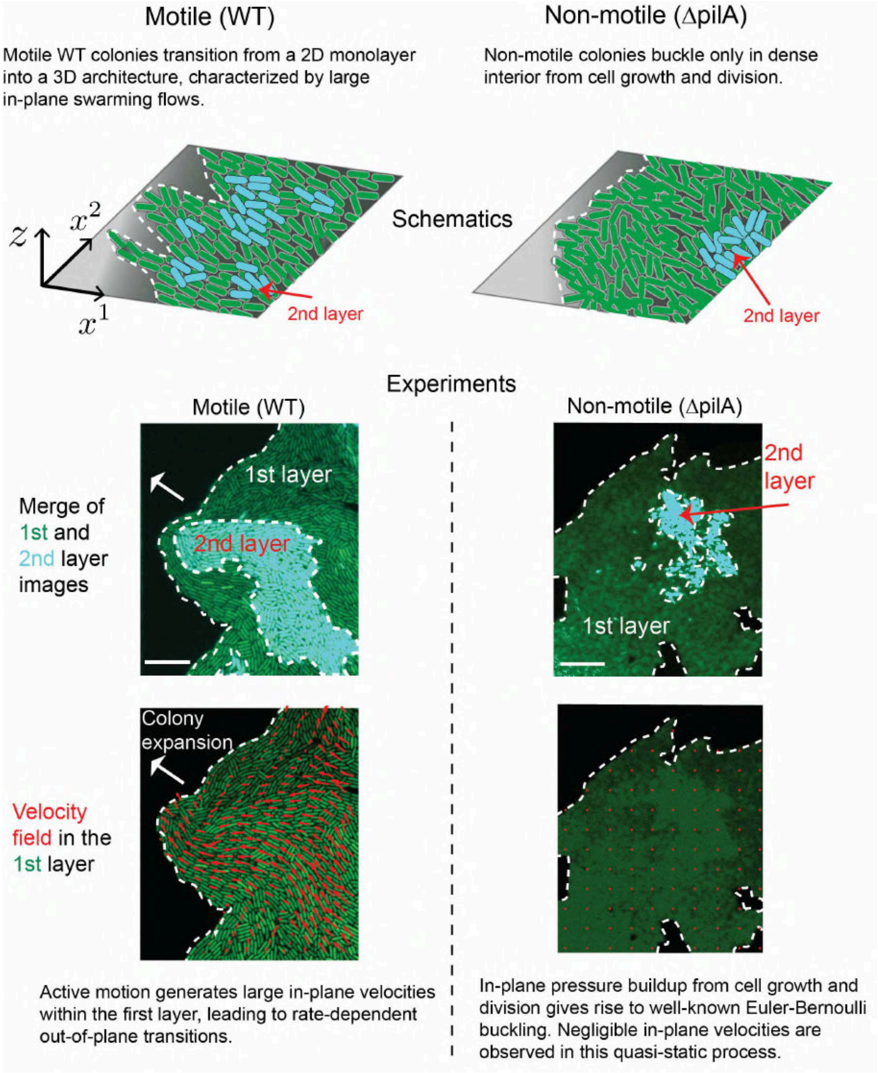


**Figure 1.4:** Top: Schematics of out-of-plane transitions of motile (wild type) and non-motile (ΔpilA) *P. aeruginosa* colonies. Below: Confocal images of motile and non-motile colonies in the first and second layers. Out-of-plane transitions of individual bacteria from 2D monolayers (cyan) is observed for motile (wild type WT, left column) and non-motile (ΔpilA, right column) strains. For motile colonies, these transitions occur in regions of large in-plane collective swarming flows, especially near the colony's leading edges. In contrast, non-motile colonies do not exhibit any flows within the colony, and transitions occur within the interior of the colony where cell density increases slowly via cell growth and division. Snapshots of the experiments show a z-stack superposition of the first layer (in green) and a second layer (pseudo-colored in cyan). Velocity fields within the monolayer (below) are shown with red arrows.

have already experienced an excitation nearby, i.e., these hops are facilitated and heterogeneous. See SI Movie S8 for a contour plot showing the facilitated dynamics within the colony. This glassy-like packing eliminates any flow-induced shear or compressible stresses from being generated within the colony, and the out-of-plane transitions resemble more of the non-motile colonies. Further, we observe individual bacteria popping out of the monolayer over time scales that are characteristic of bacterial growth and division.

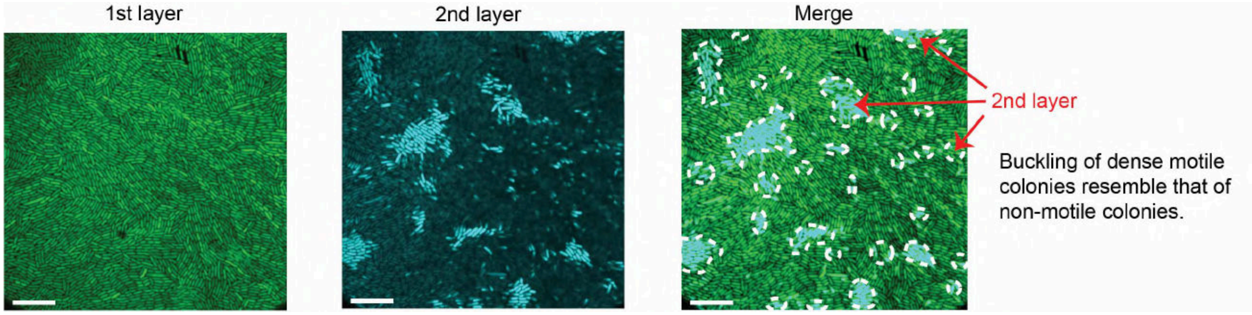


**Figure 1.5:** Snapshots of the first layer (in green), second layer (pseudo-colored in cyan), and merged images of WT colony, at large cell density. Large densities suppress active swarming and the colony enters into a kinetically arrested glassy state. Individual cells can be observed to transition into the second layer from growth and division, away from the leading edges and in the interior (see SI Movie S6). Thus, dense motile colonies and associated transitions from 2D to 3D resemble that of non-motile mutant colonies. All scale bars are 10$\mu$m.

## 2. Questions

Taken together, these observations indicate an interplay between cell density, cell motility, and 2D-to-3D growth of motile bacterial monolayers. Although it is now clear that such an interplay should exist, there are many unanswered fundamental questions:

(i) What are the mechanisms involved in out-of-plane growth of a motile swarming colony;

(ii) How does cell density and motility affect the state of the colony (i.e., swarming vs. glassy); and

(iii) How does the state of the colony govern the 2D-to-3D transitions?

In the remainder of this document, we describe the theories of glassy dynamics and fluid films to fundamentally understand and characterize the dynamical state of bacterial colonies, and provide new mechanisms for out-of-plane colony growth. In Chapter II, we extend the theories of dynamical facilitation to active colloidal glasses. Using molecular dynamics simulations of active Brownian particle models, we elucidate the role of motility on the relaxation of kinetically arrested systems. We ultimately arrive at a corresponding states for active glassy systems and calculate an onset pressure (or density) that delineates the boundary between swarming vs. glassy colonies. In Chapter III, we develop a thin fluid film theory for analyzing out-of-plane motion of active bacterial monolayers in the swarming state to predict the rate-dependent motility-induced buckling instabilities leading to growth in the third dimension. We model the bacterial monolayer as a thin fluid sheet and conduct a stability analysis to predict the onset of 2D-to-3D transition. Importantly, we identify several different mechanisms leading to buckling, all of which are rate and activity dependent. A key destabilizing term in the out-of-plane momentum equation is a viscous-curvature coupling term where in-plane viscous stresses become coupled to out-of-plane motion. We arrive at a universal scaling relation between shear stresses and adhesion that describes the 2D-to-3D transitions. We further extend the analysis to compressible flows, which can also generate out-of-plane motion in a rate dependent manner. In all of the mechanisms we propose, there is a competition between a stabilizing adhesive force and a destabilizing in-plane active force. This differentiates our work from previous studies on buckling instabilities in bacterial colonies primarily mediated by growth/division induced stresses [1–7]. Using molecular simulations, we further test the universal scaling relation between shear stresses and adhesion giving credibility to the mechanisms we propose. In Chapter IV, we apply our theory of thin fluid films to our experimental observations of

*P. aeruginosa* colonies in the swarming state. Our analyses show that these motile bacteria buckle out-of-plane using a combination of different rate-dependent mechanisms. We conclude Chapter IV with additional experiments that demonstrate the importance of extracellular DNA on *P. aeruginosa* swarming motility. Addition of DNaseI, which cleaves DNA strands into fragments, removes any collective swarming patterns and thus eliminates shear stresses from being generated in-plane. Finally, in Chapter V, we list and provide a description of the Supplemental videos associated with this manuscript.

Chapter II

# ACTIVE SWARMING VS. GLASSY LIQUIDS

In this chapter, we develop a theory characterizing the glassy dynamics of motile (or active) bacterial colonies, and the crossover from swarming to glassy states marked by an onset pressure. As mentioned previously in Chapter I, experiments on motile bacterial colonies upon increasing cell density demonstrate a crossover from a state of swarming to a kinetically arrested state where motility is diminished (Fig. 1.5). The colonies at high density exhibit dynamical heterogeneity (Fig. 2.1)—a characteristic signature of glassy dynamics in molecular and colloidal systems [8–12], where there exist distinct mobile and immobile regions when observed in a small window of time $\Delta t$ [10]. Dynamic heterogeneity can also be observed clearly in the individual trajectories of bacteria shown in Fig. 2.2 tracking the magnitude of the displacement of bacteria with respect to an arbitrarily chosen time origin, *i.e.,* $|\mathbf{r}_i(t) - \mathbf{r}_i(0)|$ with $\mathbf{r}_i$ as the position of the bacteria. Figure 2.2 shows that at low densities, bacteria exhibit continuous motion resembling that of a liquid driven by a constant internal force giving rise to its motility. However, at high densities, they exhibit intermittent hopping motion, where the hopping displacements are on the order of the length scale of the individual bacteria and occur on an average time scale $\Delta t$. This time scale $\Delta t$ is typically referred to as the "instanton" time [10], i.e., the time scale in which bacteria move by a bacterial length between two quiescent periods. Such a dramatic change in the time dependent motion of the bacteria is similar to the particle displacements in molecular and colloidal glassy systems [10], and represents another characteristic signature of the emergence of glassy dynamics. Taken together, these observations indicate that motile bacterial monolayers can be considered as active, glassy colloidal systems.

Glassy systems and their dynamics are typically characterized by a relaxation time $\tau$ [10, 13], which quantifies the time scale in which every particle in the system has moved at least by a particle diameter. When a glass forming molecular liquid is cooled from high temperature to low temperature, its relaxation time dependence on temperature exhibits a crossover from being Arrhenius in the liquid state to being super-Arrhenius in the super-cooled state [14–17]. The crossover temperature is typically referred to as an "onset" temperature. The liquid exhibits homogeneous dynamics in the liquid state above the onset temperature, and dynamically heterogeneous behaviors with intermittent hopping motion below the onset temperature. These intermittent motions consequently affect the behaviors of the relaxation time in the supercooled or glassy state and give rise to the super-Arrhenius behaviors [10, 18–21]. In a completely analogous manner, a glass forming colloidal system also exhibits a similar crossover in its relaxation time, however, as a function of pressure $\Pi$, with $\Pi_0$ as the "onset" pressure and with signatures of dynamic heterogeneity in the glassy state above the onset pressure.

The relaxation behaviors of glass forming systems has been a subject of great interest in the last three decades, and there exist different perspectives towards understanding and predicting the emergent properties from microscopic aspects of glassy dynamics [13, 16, 17]. In what follows, we follow the perspective of the Dynamical Facilitation (DF) theory, which places fundamental

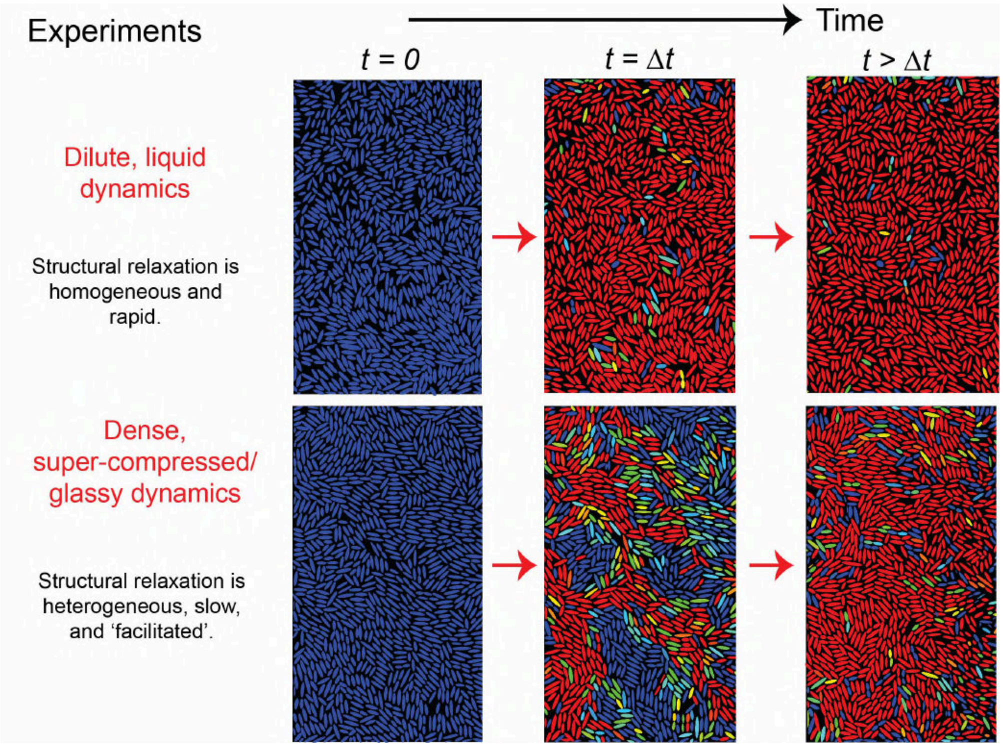


**Figure 2.1:** Snapshots of experiments for dense bacterial colonies, taken at three successive time points. Colors indicate displacement magnitude of each bacterium from its initial position, where blue indicates zero displacement and red indicates displacement more than a body length, $2\mu$m. A dilute colony shows immediate relaxation of the system, where all bacteria have displaced at least a body length in a period of time $\Delta t$ (see Fig. 2 of main text). In contrast, a dense bacterial colony exhibits dynamic heterogeneity, a characteristic signature of glassy dynamics, which results in distinct mobile and immobile regions in time $\Delta t$, as apparent by the strings of red that connect across large length scales.

importance on the dynamics of individual particles and the ensuing dynamical heterogeneity of the glassy state [14, 17, 22]. DF theory is successful in predicting the relaxation time behaviors of molecular liquids as a function of temperature [23, 24], relaxation behaviors of mixtures of glass forming molecular liquids [25], heat capacities of glass forming systems [26], and also the relaxation times of glassy binary hard disk or colloidal systems [27].

In what follows, we first provide a brief description of the DF theory for passive colloidal systems with pressure as the thermodynamic parameter. We extend the DF theory to active colloidal systems in two dimensions, with Active Brownian Particles (ABPs) as the canonical active model. We show that the extended active DF theory predicts the relaxation behaviors of a dense system of ABPs. We then study the effects of the aspect ratio of the particles and polydispersity on relaxation behaviors, by considering spherocylinders as approximate representations of the bacterial colonies. Finally, we analyze the relaxation time in experiments of bacterial monolayers, and find the extended DF theory to be consistent with the dependence of relaxation time as a function of cell density.

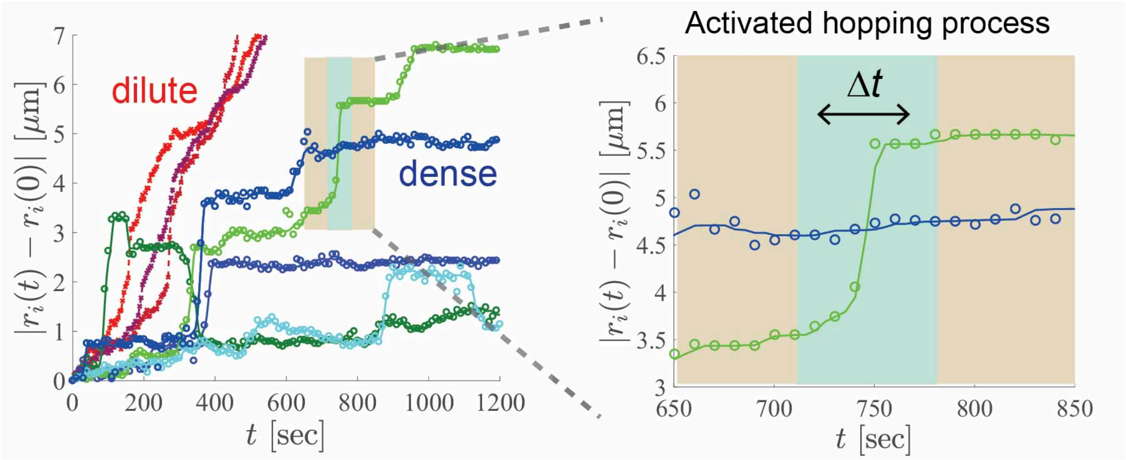


**Figure 2.2:** Absolute values of particle displacement, $|\mathbf{r}_i(t) - \mathbf{r}_i(0)|$, corresponding to trajectories of several cells in both dilute and dense *P. aeuroginosa* colonies. A magnified view of the trajectory is shown where a hopping event, similar to activated hopping events in molecular and colloidal glassy systems is observed, thus exhibiting another characteristic signature of glassy dynamics.

# 1. DF theory for passive colloidal systems

We begin by a brief description of the DF theory for colloidal systems. We refer the reader to references [10] and [27] for a detailed development of the theory for molecular liquids and colloidal systems, respectively. The theory is originally developed for molecular liquids as a function of changing temperature [10, 14, 28], but has been extended recently to systems with pressure (or density) as the governing parameter [27]. In what follows, we discuss the theory as applicable to colloidal systems with relevance to bacterial colonies, where changing density or pressure is typically the relevant thermodynamic parameter. As mentioned before, DF theory fundamentally takes into account aspects of dynamical heterogeneity, by means of “excitations” or “soft-spots”, which encompass mobile regions observed in a window of instanton time $\Delta t$. In the perspective of DF theory, the crossover from liquid to a super-cooled or super-compressed liquid is accompanied by the emergence of the excitations (or soft-spots). These excitations then facilitate the motion of nearby regions in a hierarchical manner, leading to a super-Arrhenius “parabolic” form for the relaxation time as a function of inverse temperature for molecular liquids, or pressure for colloidal systems.

DF theory entails studying the concentration of excitations $C_a(\Pi; t_{\text{obs}})$, which is defined as the number of particles that displace by at least an amount $a$ in an observation time window $t_{\text{obs}}$ at a given pressure $\Pi$, i.e.,

$$C_a(\Pi; t_{\text{obs}}) = \frac{1}{N} \sum_{i=1}^{N} \Theta\left(|\mathbf{r}_i(t_{\text{obs}}) - \mathbf{r}_i(0)| - a\right), \tag{2.1}$$

where $\Theta$ is a Heaviside step function and $\mathbf{r}_i(t)$ is the position vector of an individual particle [10, 27]. The size of the displacement $a$ is typically less than or equal to the size of the particle $\sigma$. At sufficiently high pressures or densities, the concentration $C_a(\Pi; t_{\text{obs}})$ scales linearly with $t_{\text{obs}}$ when $t_{\text{obs}} \gg \Delta t$, where $\Delta t$ is the instanton time, and is given by

$$C_a(\Pi; t_{\text{obs}}) \sim t_{\text{obs}} c_a(\Pi), \tag{2.2}$$

and $c_a(\Pi)$ denotes the rate of particle displacements. The rate $c_a(\Pi)$ reduces exponentially with

pressure, giving rise to an ideal gas of excitations above an onset pressure $\Pi_0$:

$$c_a(\Pi) \sim \exp(-\kappa_a(\Pi - \Pi_0)), \tag{2.3}$$

where $\kappa_a$ denotes the energy scale corresponding to the emergence of excitations of size $a$. This then leads to excitations separated by a length scale

$$\ell_a \sim c_a^{-1/d_f}. \tag{2.4}$$

where $d_f$ is the fractal dimension given by $d_f = 1.9$ for two dimensional systems [10]. Furthermore, the energy scale $\kappa_a$ is observed to depend logarithmically on the particle displacement, *i.e.,*

$$\kappa_a - \kappa_\sigma = \gamma\kappa_\sigma \ln(a/\sigma), \tag{2.5}$$

where $\gamma$ is a system dependent proportionality constant.

The kinetics of the excitations is facilitated, where motion in one region leads to motion in its vicinity, i.e., motion begets motion [10]. In this case, the relaxation time of the system, defined as the time required for almost all particles to move a displacement of particle size $\sigma$, is governed by the time scale connecting excitations separated by the equilibrium length scale $\ell_\sigma$. Inspired by the lattice models with kinetic constraints, such as the East model [29–34], the energy barrier associated with connecting excitations of size $\sigma$ is given by

$$\kappa_{\ell_\sigma} - \kappa_\sigma = \gamma\kappa_\sigma \ln(\ell_\sigma/\sigma) = \frac{\gamma\kappa_\sigma^2}{d_f}(\Pi - \Pi_0), \tag{2.6}$$

where the second equality is obtained by using (2.4) and (2.3). Using transition state theory and (2.6), the relaxation time for the system is obtained as

$$\tau(\Pi) \sim \exp([\kappa(\Pi - \Pi_0)]^2). \tag{2.7}$$

thus yielding the super-Arrhenius "parabolic law" for the logarithm of the relaxation time above the onset pressure $\Pi_0$, where $\kappa = \sqrt{\frac{\gamma\kappa_\sigma^2}{d_f}}$ is a system dependent energy scale.

## 2. DF theory for active colloidal systems

As mentioned before, DF theory was established originally for thermal fluids [10, 14, 28], and has been extended to equilibrium hard colloids with pressure as the control parameter instead of inverse temperature [27]. However, it is not apriori clear whether the DF theory can be extended to active matter systems. Motivated by the recent developments in active matter [35–39] and the concept of mechanical pressure for active systems [40–45], we extend the DF theory by supposing that the active pressure is the relevant controlling variable in understanding glassy dynamics. We demonstrate below through molecular simulations that such an ansatz provides a reasonable description of glassy dynamics inherent to active colloidal suspensions. Although we take the perspective of DF theory, note that others have taken alternative approaches such as extensions of the random first-order transition (RFOT) theory [46], and it will be interesting to compare these different perspectives in future work.

To begin, recall that dynamical heterogeneity is observed in our experiments on motile bacterial colonies at high densities (see Fig. 2.1 and Fig. 2 of the main text). To characterize dynamic heterogeneity and to extend the applicability of DF theory for bacterial monolayers, we start

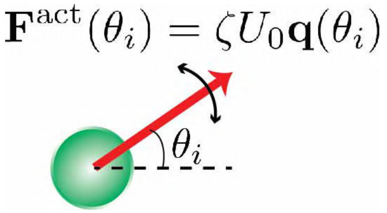


**Figure 2.3:** Schematics of an ABP with applied active forces along its orientation.

with a simplistic molecular model containing bi-disperse hard disks based on the active Brownian particle (ABP) models, a paradigmatic model commonly studied in the emergent field of active matter [35–40]. We further extend the analysis to rod-shaped spherocylinders with polydispersity resembling the realistic distributions inherent to colonies of *P. aeruginosa*, and find that there exists no qualitative difference between the spherocylindrical and the bi-disperse hard disk systems. Unlike experiments on the real colonies, molecular simulations enable careful control over packing fraction $\phi$ and activity parameter, and thus are well-suited to test and extend the applicability of DF theory for active colloidal systems.

## 2.1 DF theory for active Brownian particles

In this section, we consider the canonical model of ABPs, a paradigmatic model for studying active systems, where there exist self-propusive forces in the direction of motion of the particle [37, 40]. An ABP is defined by a position $\mathbf{r}_i$ and an angular coordinate $\theta_i$ defining the orientation of the particle with respect to a fixed axis (see Fig. 2.3). The particle is subjected to an active force $\mathbf{F}^{\mathrm{act}}(\theta_i)$ along its orientation $\theta_i$ in addition to the interaction forces between the particles as shown in Fig. 2.3. Such a model with self-propulsive force along the orientation is an appropriate starting point for bacterial monolayers of *P. aeruginosa*, where there exists a motility inducing (or an active) force along the orientation of the bacteria created by the extension and retraction of the pili [47–50].

The dynamics of the ABPs are governed by the $N$-particle Langevin equations,

$$\zeta \frac{d\mathbf{r}_i}{dt} = \mathbf{F}^{\mathrm{act}}(\theta_i) + \sum_{j \neq i} \mathbf{F}^{\mathrm{P}}_{ij}, \tag{2.8}$$

$$\frac{d\theta_i}{dt} = \sqrt{\frac{2}{\tau_{\mathrm{R}}}} \Lambda_{\mathrm{R}}, \tag{2.9}$$

where $\zeta$ is the hydrodynamic drag coefficient. Here, $\mathbf{F}^{\mathrm{act}}(\theta_i) \equiv \zeta U_0 \mathbf{q}_i(\theta_i)$ is the self-propulsive force with $U_0$ being the motility speed, $\mathbf{q}_i$ is the unit vector specifying the particle's orientation where $\mathbf{q}_i = (\cos\theta_i, \sin\theta_i)$ in 2D, and $\mathbf{F}^{\mathrm{P}}_{ij}$ is the interaction force between particles $i$ and $j$. Further, $\tau_{\mathrm{R}}$ is the reorientation time of the swimmer such that the rotational diffusivity $D_{\mathrm{R}} = 1/\tau_{\mathrm{R}}$, and the reorientation dynamics occur as a continuous random process with $\Lambda_{\mathrm{R}}$ being the Gaussian white noise. We note that, in general, the rotational diffusion need not necessarily be thermal in origin (for example, bacteria can use flagella to reorient using non-thermal mechanisms), and thus $\tau_{\mathrm{R}}$ may be entirely decoupled from all other system parameters unlike other active matter models [51]. We also neglect translational Brownian motion in (2.8).

The parameters we vary are the area fraction $\phi = n\pi\sigma^2$ with $n$ as the number density, and an activity parameter given by the Péclet ($Pe$) number

$$Pe = \frac{U_0 \tau_{\mathrm{R}}}{\sigma}, \tag{2.10}$$

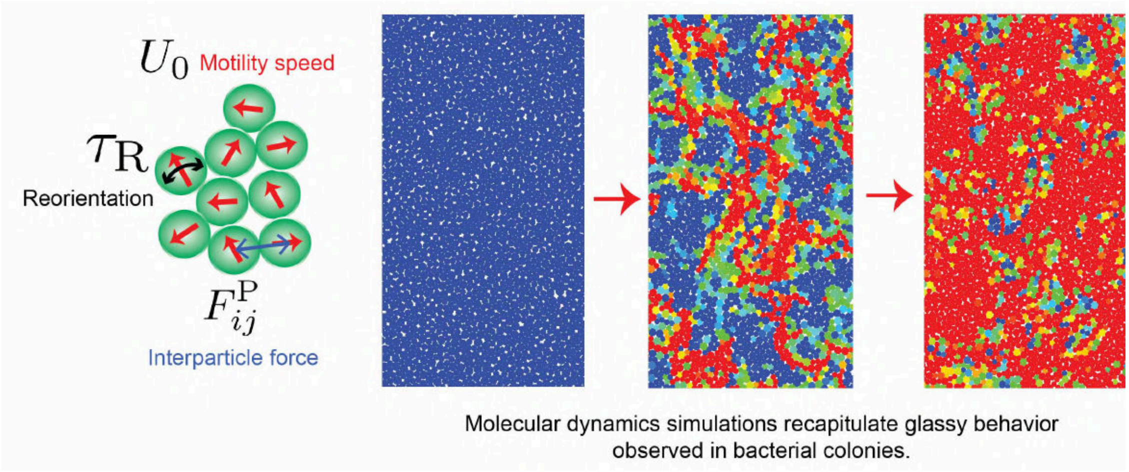


**Figure 2.4:** Left: A schematic showing the molecular model and key parameters in our molecular dynamics (MD) simulations, where we use an ABP model with motility speed $U_0$, reorientation time $\tau_R$, bidispersity ratio of 1.4. Right: Snapshots of simulations at three successive time steps for a dense system exhibiting glassy dynamics. MD simulations of ABPs at high densities recapitulate dynamic heterogeneity characteristic to experiments on bacterial colonies (see Fig. 2.1).

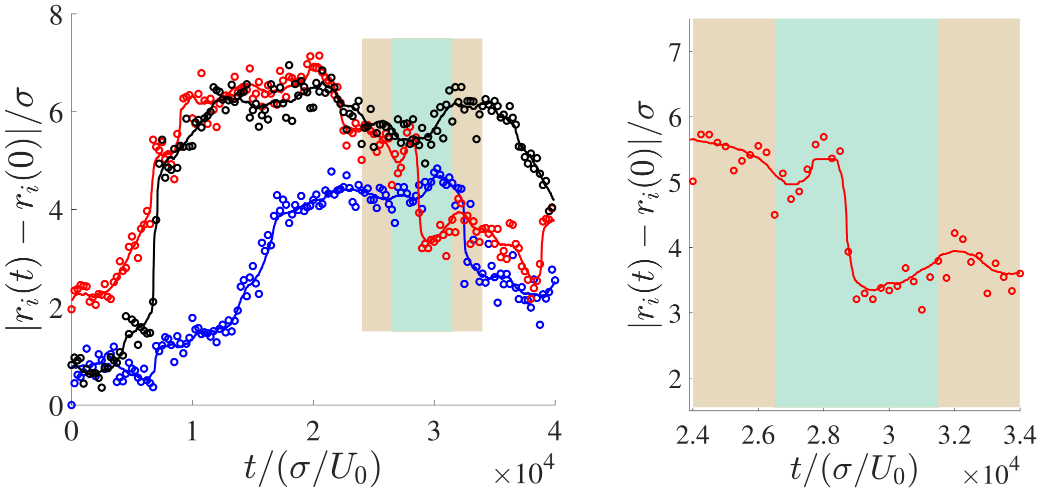


**Figure 2.5:** Absolute values of particle displacement, $|\mathbf{r}_i(t) - \mathbf{r}_i(0)|$, corresponding to trajectories of three different particles in a dense bidisperse active system at an area fraction $\phi = 0.83$. A magnified view of the trajectory is shown where a hopping event, similar to activated hopping events in passive molecular and colloidal glassy systems, is observed.

a non-dimensional number defined by the ratio of the intrinsic run length of the active particle $U_0\tau_R$ over its size $\sigma$. The activity parameter can also be expressed as $Pe = U_0/(D_R\sigma)$ denoting the ratio of translational convection over the rotational diffusion, and can be further rewritten as $Pe = \tau_R/(\sigma/U_0)$ denoting the ratio of the time scale associated with rotational diffusion and the time scale associated with traversing a particle diameter under the self-propulsive force. To avoid interference by crystallization, we use a binary mixture of small and large particles with diameters $\sigma$ and $\sigma_1$, and mole fractions $(1-\chi) = 2/3$ and $\chi = 1/3$, respectively, prepared at an area fraction

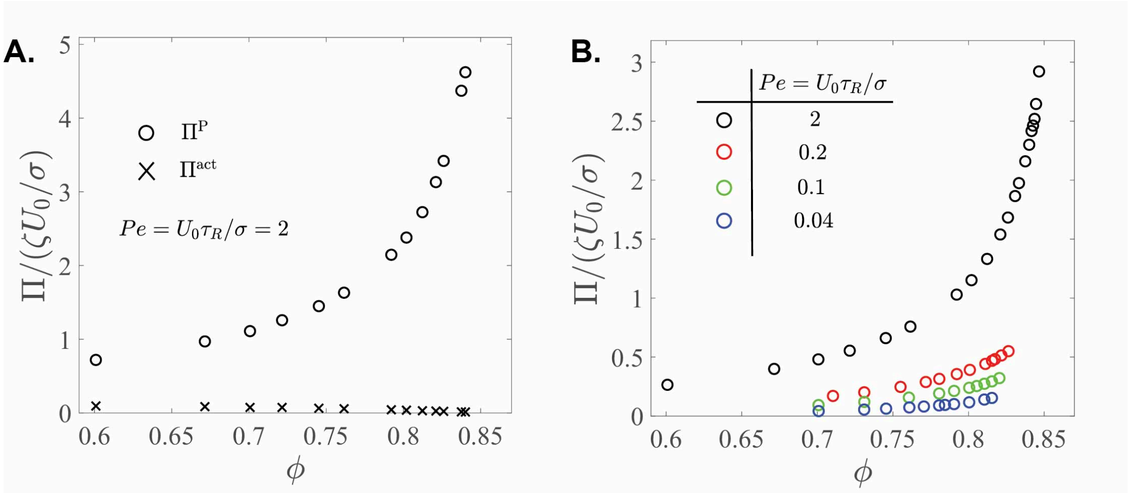


**Figure 2.6:** (A) Contribution to pressure from the interaction and active forces as a function of area fraction, $\phi$, for a fixed activity $Pe = 2$. For dense active systems considered, pressure contributions from active forces are negligible compared to those arising from interaction forces. (B) Pressure as a function of area fraction, $\phi$, for four different values of activity, $U_0\tau_R/\sigma$. The pressure vs. area fraction relationships are used to characterize the onset of glassy dynamics in our simulations.

$\phi = N\pi((1-\chi)\sigma^2 + \chi\sigma_1^2)/A$, with size ratio of $\sigma_1/\sigma = 1.4$ [27]. We vary the area fraction $\phi$ to be in the range from 0.70 to 0.845, and $Pe$ from 0.04 to 2. The ABPs are considered to be hard disks, where the potential is singular and non-zero only at contact. In this case, we use a modified potential-free algorithm [52], in which overlaps from convective and Brownian steps are separated along the line of centres of the two particles to yield an equivalent force until they are no longer in contact.

Figure 2.4 shows dynamical heterogeneous behaviors in our ABP model systems, at high area fractions $\phi$, that are qualitatively similar to those observed in the motile bacterial colonies at high densities (shown in Fig. 2.1). Further, Fig. 2.5 shows the trajectories of the individual particles at high fractions where there exist intermittent hopping motions on a length scale of the order of the particle diameter. Taken together, these observations indicate that the ABP models are reasonable representations of realistic bacterial colonies in their glassy states, and therefore could be utilized to develop a systematic extension of the DF theory to active glassy systems.

For the system of binary mixture of ABPs, we begin the analysis of glassy dynamics by examining the pressure ($\Pi$) vs. area fraction ($\phi$) relation. Pressure can be defined as the negative trace of the stress tensor $\boldsymbol{\sigma}$ [40, 45] given by

$$\boldsymbol{\sigma} = \boldsymbol{\sigma}^{\mathrm{P}} + \boldsymbol{\sigma}^{\mathrm{act}}, \tag{2.11}$$

where, $\boldsymbol{\sigma}^{\mathrm{P}}$ is the standard Irving-Kirkwood expression for the stress tensor arising from interaction forces $\mathbf{F}_{ij}^{\mathrm{P}}$

$$\boldsymbol{\sigma}^{\mathrm{P}} = -\frac{1}{A}\Big\langle \sum_i \sum_{j>i} \mathbf{r}_{ij} \otimes \mathbf{F}_{ij}^{\mathrm{P}} \Big\rangle, \tag{2.12}$$

with $A$ being the area of the system and $\mathbf{r}_{ij}$ the interparticle distance. The active stress for a system of ABPs is given by

$$\boldsymbol{\sigma}^{\mathrm{act}} = -\frac{1}{A}\Big\langle \sum_i \mathbf{r}_i \otimes \mathbf{F}^{\mathrm{act}}(\theta_i) \Big\rangle, \tag{2.13}$$

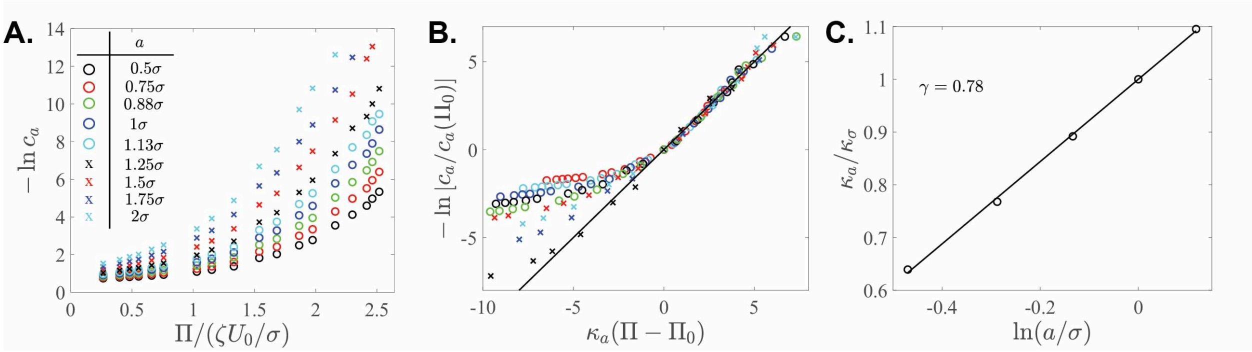


**Figure 2.7:** (A) Concentration of excitations for various displacements $a$ when $Pe = (U_0\tau_{\mathrm{R}})/\sigma = 1$. (B) Collapse of the concentrations for various displacements using (2.14) and (2.15). Legends are the same for (A) and (B). (C) Logarithmic scaling of the energy scale $\kappa_a$ following (2.15). This analysis yields the parameters $\kappa_a$ and $\gamma$ in the active DF theory for $Pe = (U_0\tau_{\mathrm{R}})/\sigma = 1$.

and can be added to the overall stress only in the absence of any inhomogeneous flows [45], which is applicable for our system of ABPs with no alignment interactions. Figure 2.6A shows the pressure as a function of area fraction for a given value of activity. It can be seen that the contributions from the active stress are negligible compared to the stresses from interactions at high densities. This is in contrast to systems at very low densities, where the pressure can be dominated by contributions from active forces [40]. Figure 2.6B shows pressure $\Pi(\phi)$ as a function of $\phi$ for various activities $Pe$.

We now study the extensions of the DF theory by an analysis of the concentration of excitations as a function of pressure $\Pi$ for a non-zero $Pe$. For all the systems considered, our molecular simulations show that the excitations are localized at high area fractions or high pressures. Figure 2.7A shows the concentration of excitations $c_a(\Pi; Pe)$[1] defined from (2.1) and (2.2) for various particle displacements of size $a$, and $Pe = 1$. As can be seen in Fig. 2.7B, the concentration $c_a(\Pi; Pe)$ follows an exponential dependence with the pressure $\Pi$ above an onset pressure $\Pi_0$, similar to that of the non-active systems [27]. The energy scale $\kappa_a$ again follows a logarithmic dependence on the size of the displacement $a$ as seen in Fig. 2.7C. We find the same observations hold when we repeat the analysis for various activities $Pe$. Importantly, we see that the activity $Pe$ modifies both the onset pressure $\Pi_0(Pe)$ and the energy scale for the emergence of excitations $\kappa_a(Pe)$ as demonstrated from the collapse of data in Fig. 2.8. This leads to the following generalized relation for the concentration of excitations:

$$c_a(\Pi; Pe) \sim \exp\Big( -\kappa_a(Pe)[\Pi - \Pi_0(Pe))]\Big). \tag{2.14}$$

[1]A key concept in dynamical facilitation is the identification of spatially localized excitations, or soft spots, within a material that engender structural relaxation. For a simulation at a given area fraction, the first step is to obtain the trajectories of each particle, $|\Delta\mathbf{r}_i(t)| = |\mathbf{r}_i(t) - \mathbf{r}_i(0)|$, where $\mathbf{r}_i(t)$ is the position of particle $i$ at time $t$. Note that the displacement is relative to some initial time $t = 0$, which remains fixed (as opposed to a moving window difference, $|\mathbf{r}_i(t) - \mathbf{r}_i(t-1)|$). Usually, when the area fraction is high, the concentration of excitations are calculated not by the raw displacements but using displacements that are either time averaged over a small period of time $\delta t \ll \Delta t$, or finding the inherent states corresponding to the lowest energy at the time point of the trajectory [10]. This identifies non-trivial displacements indicating significant changes in the inherent structures, and not the vibrations or noise present in the system. In the case of our active systems, both in molecular simulations and experiments on bacterial colonies, we remove the small, rapid fluctuations by coarse-graining over a small time interval using a low-pass filter to eliminate high-frequency particle motion.

This demonstrates that the emergence of excitations can be understood with two activity dependent parameters: the energy scale $\kappa(Pe)$ and the onset pressure $\Pi_0(Pe)$. Note that the onset pressure increases as $Pe$ increases indicating that glassy dynamics begins at much higher area fractions for increasing activity. Furthermore, the energy scale $\kappa_a$ again depends logarithmically on the size of the particle displacement $a$ given by

$$\kappa_a(Pe) - \kappa_\sigma(Pe) = \gamma(Pe)\kappa_\sigma(Pe)\ln\left(\frac{a}{\sigma}\right), \tag{2.15}$$

as in the case of passive glassy systems, however, with $\gamma$ depending on activity $Pe$. In summary, the analysis indicates that hierarchical dynamics exists even in active glassy systems, and can be analyzed on a similar footing as the passive glassy systems.

The exponential dependence of the concentration of excitations of size $a$ in (2.14) leads to a mean separation distance

$$\ell_a(\Pi; Pe) \sim c_a^{(-1/d_f)}. \tag{2.16}$$

At this stage, we assume that even in the presence of non-zero activity ($Pe \neq 0$), the system in the glassy state is sufficiently close to equilibrium[2]. In this case, the relaxation time of the system, i.e., the time scale for every particle to move a particle size $\sigma$, can be obtained by finding the energy barrier required to connect excitations separated by the length scale $\ell_\sigma(\Pi; Pe)$ given by

$$\kappa_{\ell_\sigma} - \kappa_\sigma = \gamma\kappa_\sigma \ln(\ell/\sigma) = \Big(\gamma(Pe)[\kappa_\sigma(Pe)]^2/d_f\Big)(\Pi - \Pi_0(Pe)). \tag{2.17}$$

[2]We note that a rigorous justification of the assumption of equilibrium in calculating the time scale $\tau$ with an energy barrier and modified pressure $\Pi$ is required for the active systems with non-conservative forces at the microscale. In this work, we postulate such a scenario, and it is only aposteriori supported by the predictions of the relaxation time for non-zero activity. The rigorous first principles justification of the form of equilibrium assumption that the time scale $\tau \propto \exp([\Pi - \Pi_0]E_\mathrm{b})$, where $E_\mathrm{b}$ is an energy barrier, will be left to future work.

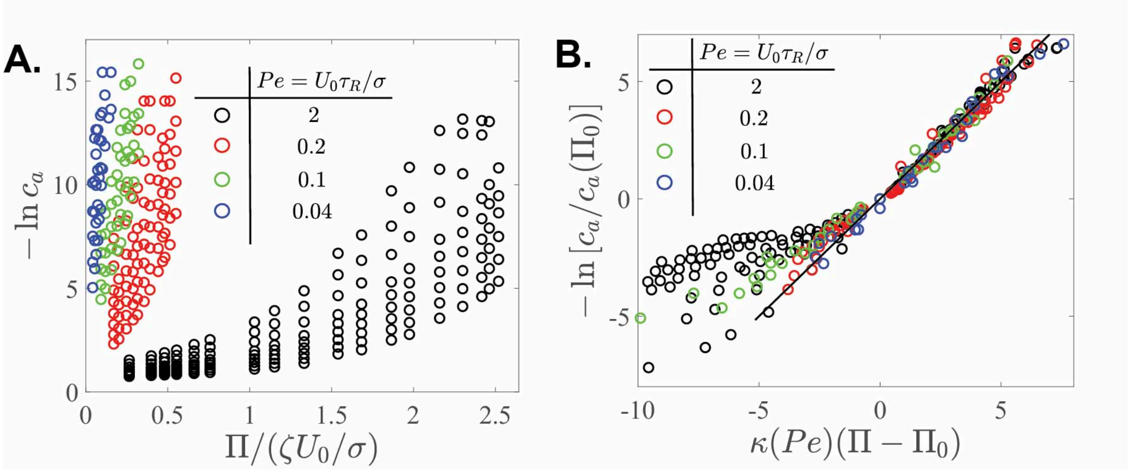


**Figure 2.8:** (A) Concentration of excitations for various $Pe$ and displacement size $a$, which yields the parameters $\kappa$ and $\gamma$ for each activity. (B) Collapse of the concentration of excitations for various activities and displacements using (2.14), shows the remarkable generality of the exponential behavior of the concentration of excitations. To obtain this collapse, 70 independent MD realizations were conducted to sweep across four activities and a wide range of densities.

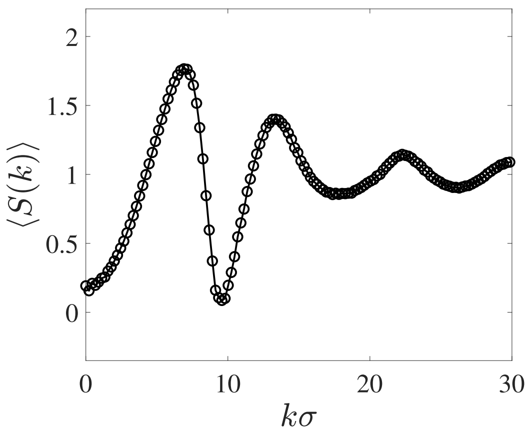


**Figure 2.9:** Static structure factor for $Pe = U_0\tau_R/\sigma = 2$ near the onset pressure. The wave vector corresponding to the first peak is used in the calculation of the dynamic structure factor $F_s(\mathbf{k}, t)$ in (2.21).

With the assumption that active glassy states at high densities are still close to equilibrium in the arrested state, application of the transition state theory yields the relaxation time at high fractions to be

$$\tau(\Pi; Pe) \sim \exp\left(\left[\kappa(Pe)[\Pi - \Pi_0(Pe)]\right]^2\right), \tag{2.18}$$

where $\kappa(Pe) = \sqrt{\frac{\gamma(Pe)}{d_f}}\kappa_\sigma(Pe)$. Equation (2.18) says that active glassy systems still obey the same parabolic law that is used to describe the relaxation behaviors of non-active systems. If this is the case, then the active glassy systems behave in a qualitatively similar manner as the equilibrium super-compressed glassy systems [27]. The only difference appears to be that activity modifies the onset pressure $\Pi_0(Pe)$, the energy scale $\kappa(Pe)$, and $\gamma(Pe)$. Taken together, extensions of the DF theory to the case of active systems yield the relaxation time of the system to be

$$\ln\left(\frac{\tau_\sigma}{\tau_0}\right) = [\kappa(\Pi - \Pi_0)]^2 + E_a(\Pi - \Pi_0), \text{ if } \Pi > \Pi_0 \tag{2.19}$$

$$= E_a(\Pi - \Pi_0), \qquad \text{if } \Pi > \Pi_0 \tag{2.20}$$

where $\tau_0$ is the relaxation time at the onset pressure.

To verify the predictions from Eqs. (2.19)-(2.20), we estimate the relaxation times of the system for various area fractions and activities using the time decay of the density correlations [14] given by

$$F_s(\mathbf{k}, t) = \frac{1}{N}\left\langle \sum_{i=1}^{N} \exp(\mathrm{i}\mathbf{k} \cdot [\mathbf{r}_i(t) - \mathbf{r}_i(0)])\right\rangle. \tag{2.21}$$

Here, $\mathbf{k}$ is the wave-vector corresponding to the peak of the structure factor [53] (see Fig. 2.9), and $\langle\cdot\rangle$ denotes an ensemble average. Note that active forces may result in mean rigid-body translations, which we subtract from the displacements when calculating $F_s(\mathbf{k}, t)$. Figure 2.10A shows $F_s(\mathbf{k}, t)$ for various fractions $\phi$, and therefore various pressures $\Pi$, for a given activity $Pe$. It shows that the long time decay of the correlation functions change from being exponential at low fractions to stretched exponential at high fractions, resembling the dynamical correlation functions that are similar to standard glassy systems. Furthermore, assuming that the relaxation time $\tau$ is given by the decay of the correlation function $F_s(\mathbf{k}, t)$ to one-tenth of its initial value, we find from Fig. 2.10B that

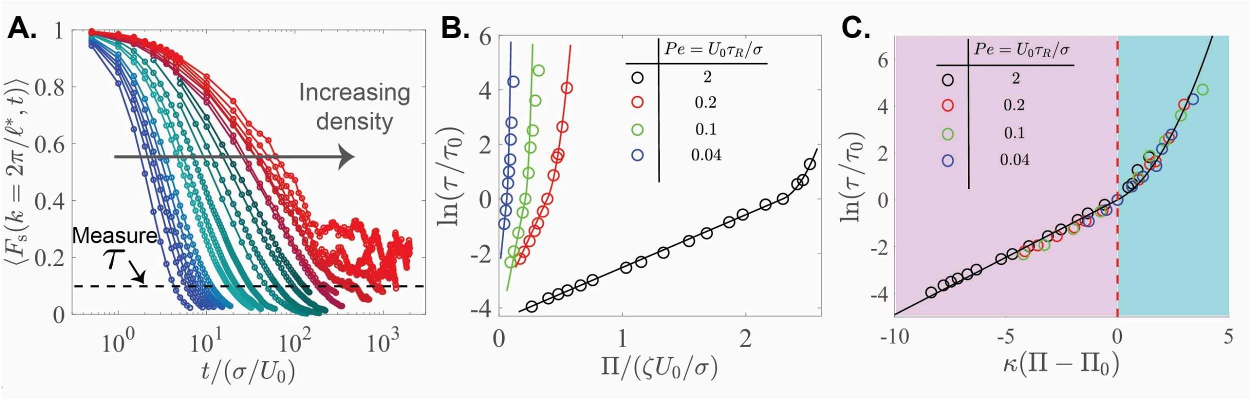


**Figure 2.10:** (A) Dynamic structure factor, $F_s(k = 2\pi/\ell^*, t)$, for activity $Pe = U_0\tau_{\mathrm{R}}/\sigma = 2$. Different colors correspond to simulations at varying densities, and $\ell^*$ is the length associated with the first peak of the static structure factor. (B) Relaxation times as a function of mechanical pressure $\Pi$, for various values of activity $Pe = 0.04, 0.1, 0.2$, and 2, show crossover from Arrhenius-like behaviors to super-Arrhenius behaviors at high densities, similar to the behaviors characteristic of molecular and colloidal glassy systems. (C) All data collapse universally onto the parabolic law, $\kappa^2(\Pi - \Pi_0)^2$, as predicted by the DF theory (2.19). The solid line corresponds to the relaxation time formula given by (2.19) and (2.20). The onset relaxation time $\tau_0$, energy barrier $\kappa$, and onset pressure $\Pi_0$ are all functions of $Pe$.

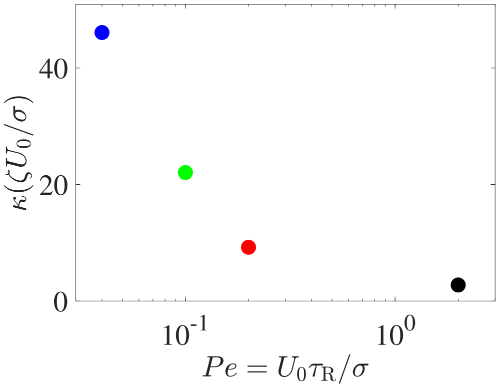


**Figure 2.11:** Energy scale $\kappa$ decreases with activity $Pe$.

the logarithm of the relaxation times show again a remarkable crossover from linear dependence on $\Pi$ at low pressures to a non-linear dependence above the onset pressure. Figure 2.10C shows that the parabolic form for the relaxation time in (2.19) is in excellent agreement with the relaxation times obtained from $F_s(\mathbf{k}, t)$ above the onset pressure $\Pi_0(Pe)$, for various $Pe$, thus demonstrating the universal features of glassy dynamics at all activities. These results indicate that the extended DF theory provides a useful perspective to describe the onset and further relaxation behaviors of glassy dynamics in active systems.

## 2.2 *Activity and softness*

Two important concepts emerge from extending DF theory to active glassy systems. First, as mentioned before, the crossover into glassy behavior is pushed up to larger pressures (or densities) with

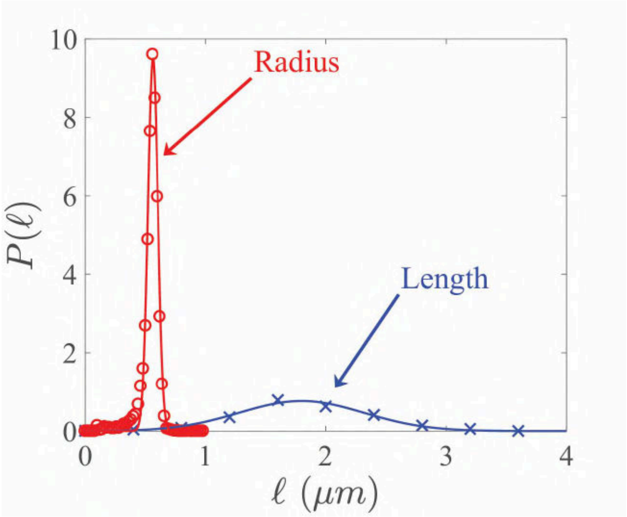


**Figure 2.12:** Probability distribution of the width and length of individual bacteria, obtained from cell segmentation of colonies.

increasing motility. These generic observations were discussed via MD simulations in earlier works [53–55], but with no theoretical interpretation. Secondly, the material parameter $\kappa$ corresponding to an excitation of size $\sigma$ can be physically interpreted as a local energy barrier to displace a particle volume of void (an excitation); it points to local 'softness' within the heterogeneous material, although a fundamental connection of $\kappa$ to a bulk material property such as elastic bulk modulus or shear modulus has not yet been established in the context of DF theory. Figure 2.11 shows $\kappa$ decreasing as a function of $Pe$ indicating that the material 'softens' and relaxes more quickly with increasing activity. This is reminiscent of non-Newtonian fluids that have elastic and viscous moduli that depend on imposed external shear rate [56–58].

# 3. Swarming and glassy dynamics of active Brownian spherocylinders

The ABP systems studied in the previous section constitute an important model for developing and testing the extensions of DF theory to active glassy systems. However, the bacterial colonies are not hard disks as in the case of ABPs; they have an average aspect ratio larger than one, and are polydisperse in nature (Fig. 2.12). Thus, understanding glassy dynamics in polydisperse systems that resemble bacteria is an important step towards interpreting the glassy behaviors of bacterial colonies. To this end, we construct a new particulate system consisting of active Brownian spherocylinders (Fig. 2.13), that resemble bacterial monolayers observed in our experiments. In particular, we consider systems made up of polydisperse spherocylinders, with polydispersity as that of *P. aeruginosa* colonies in Fig. 2.12. We then study the glassy dynamics of passive and active polydisperse spherocylinders and show that there exists an onset pressure above which the relaxation behaviors again follow the "parabolic" form similar to the case of ABPs, thus showing that the DF theory can be used to analyze scenarios close to dense bacterial colonies.

## 3.1 Passive polydisperse spherocylinders

We begin by analyzing the glassy dynamics of passive Brownian spherocylinder systems. The spherocylinders are created by a rigid assembly of 9 overlapping spherical particles along their line of centers. The particles interact via a Weeks-Chandler-Andersen (WCA) potential [59], in which a Lennard-Jones (LJ) potential is shifted upwards, truncated at the potential minimum of $2^{1/6}\sigma$ (such that the potential is purely repulsive), and assigned a well depth of $\epsilon$. The particles in a single spherocylinder are rigidly constrained to lie along the line of centers at their fixed positions.

The motion of spherocylinder systems are governed by the Langevin equations corresponding to the center particle

$$\mathbf{0} = -\zeta \mathbf{U}_i + \mathbf{F}_i^{\mathrm{B}} + \mathbf{F}_i^{\mathrm{P}} \tag{2.22}$$

$$\mathbf{0} = -\zeta_{\mathrm{R}} \mathbf{\Omega}_i + \mathbf{L}_i^{\mathrm{B}}, \tag{2.23}$$

where $\mathbf{U}_i = \dfrac{d\mathbf{x}_i}{dt}$ with $\mathbf{x}_i$ being the position of the center particle of the spherocylinder, $\mathbf{\Omega}_i = \dfrac{d\theta_i}{dt}$ is the angular velocity of the spherocylinder about its center, $\zeta$ and $\zeta_{\mathrm{R}}$ are the translational and rotational drag coeffiецeints, $\mathbf{F}_i^{\mathrm{P}}$ is the interparticle force between the particles, and $\mathbf{F}_i^{\mathrm{B}}$ and $\mathbf{L}_i^{\mathrm{B}}$ are the Brownian translational force and rotational torque, respectively. Translational Brownian forces satisfy the fluctuation-dissipation relation $\langle \mathbf{F}_i^{\mathrm{B}} \rangle = \mathbf{0}$ and $\langle \mathbf{F}_i^{\mathrm{B}}(0)\mathbf{F}_i^{\mathrm{B}}(t) \rangle = 2k_{\mathrm{B}}T\zeta\delta(t)\mathbf{I}$, where $k_{\mathrm{B}}$ is Boltzmann's constant. Similarly, rotational torque has the statistics $\langle \mathbf{L}_i^{\mathrm{B}} \rangle = \mathbf{0}$ and $\langle \mathbf{L}_i^{\mathrm{B}}(0)\mathbf{L}_i^{\mathrm{B}}(t) \rangle = 2k_{\mathrm{B}}T\zeta_{\mathrm{R}}\delta(t)\mathbf{I}$. The rigid bodies reorient due to both rotational noise, and also from interparticle interactions that can rotate the rigid body about its center. Rotations due to interparticle interactions are handled naturally from WCA interactions of each constituent particle with all particles not part of its own rigid body and internal constraining forces that keep the rigid body intact. All molecular simulations with spherocylinders are performed using the open source HOOMD-blue software [60, 61], where the spherocylinder particles use the rigid constraint functionality as explained in Ref. [62].[3]

The spherocylinders have width $\sigma$ and mean side length $\ell_0 = 3\sigma$ (corresponding to the center-to-center distance of the first and last particles of the spherocylinder). Polydispersity is implemented in our simulations by normally distributing the particle length between seven discrete sizes chosen from the set

$$\{\ell_0, \ell_0 + 0.75\sigma, \ell_0 + 1.2\sigma, \ell_0 + 2.0\sigma, \ell_0 - 0.75\sigma, \ell_0 - 1.2\sigma, \ell_0 - 2.0\sigma\} \tag{2.24}$$

with a standard deviation of 25% of the mean length. This polydispersity is inspired from the experimental analysis of bacterial colonies as shown in Fig 2.12.

Given the average aspect ratio of spherocylinders to be four, it is important to consider and verify whether the orientational relaxation behaviors differ or decouple with respect to the translational behaviors at high densities. Such an analysis was performed for anisotropic particles [63], where it was shown that the rotational and translational particle rearrangements have glassy behaviors of their own. To this end, following earlier works in [64], we calculate the dynamic version of the angular structure factor defined by the time correlation function

$$L_n(\theta = 2\pi/n, t) = \frac{1}{N} \Big\langle \sum_{j=1}^{N} \cos \Big[ n \left( \theta_j(t) - \theta_j(0) \right) \Big] \Big\rangle, \tag{2.25}$$

[3] Note that bacterial division is not modeled in this work in regards to the phenomena of motility induced buckling phenomena or glassy phenomena because of the large separation of timescales between motility ($\sim 20-35\mu$m/min) and division rate ($\sim 1-2$ divisions/hr). For glass and rheology simulations, the particles are confined between two parallel walls separated by one bead diameter, allowing them to translate in 2D without escaping out of plane.

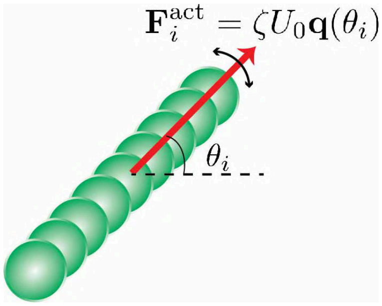


**Figure 2.13:** Schematic of a spherocylinder active particle with an active force along its orientation. The active force is zero in the case of passive spherocylinder systems.

where $n$ is a positive integer and $\theta_j$ is the orientation of the spherocylinder as shown in Fig 2.13. The decay of $L_n(\theta = 2\pi/n, t)$ indicates timescales in which every particle has reoriented at least an angle $2\pi/n$. In what follows, we chose $n = 5$ in our molecular simulations at high densities. However, we note that the qualitative nature of the relaxation behaviors for different $n$ are similar, while the onset pressure for glassy rotational behaviors is the same for different $n$. Further, in calculating $L_n(\theta = 2\pi/n, t)$, we subtract the mean rigid-body rotations from the angular displacements.

Figures 2.14A and 2.14B show the angular and translational dynamic structure factors for passive 2D suspensions of polydisperse spherocylinders at varying densities. Defining the angular relaxation time as the timescale for which $L_{n=5}$ decays to a value 0.1, Fig. 2.14C shows the rotational and translational relaxation times as a function of varying pressures $\Pi$.[4] The onset pressure $\Pi_0$ again corresponds to the pressure at which the relaxation functions deviate from Arrhenius-like form and follow super-Arrhenius-like behaviors. As shown in Fig. 2.14C, we find that the same onset pressure and the energy scale $\kappa$ describe the onset and relaxation times of rotational and translational glassy behaviors consistent with the passive DF theory. This indicates that the rotational and translational behaviors are coupled in polydisperse passive spherocylinders, thus making their behaviors similar to a binary hard disk glassy system [27]. Hence, DF theory developed for hard disk systems consisting of symmetry particles can be applied to understand the behaviors of passive polydisperse spherocylinder systems.

### 3.2 Active polydisperse spherocylinders

We now extend the analysis described in the previous section to the case of active polydisperse spherocylinders. In this case, the particles are subjected to active forces in the direction of the orientation of the bacteria as shown in Fig. 2.13. The equations of motion of active spherocylinders are given by

$$\mathbf{0} = -\zeta \mathbf{U}_i + \mathbf{F}_i^{\mathrm{B}} + \mathbf{F}_i^{\mathrm{P}} + \mathbf{F}_i^{\mathrm{act}}(\theta_i) \tag{2.27}$$

$$\mathbf{0} = -\zeta_{\mathrm{R}} \boldsymbol{\Omega}_i + \mathbf{L}_i^{\mathrm{B}}. \tag{2.28}$$

[4] The pressure in the spherocylinder system is obtained as the negative trace of the stress tensor given by

$$\boldsymbol{\sigma} = -nk_{\mathrm{B}}T\mathbf{I} - \frac{1}{A}\left(\left\langle \sum_i \sum_{j>i} \mathbf{r}_{ij} \otimes \mathbf{F}_{ij}^{\mathrm{P}} \right\rangle + \left\langle \sum_k \mathbf{r}_k \otimes \mathbf{F}_k \right\rangle\right), \tag{2.26}$$

where $A$ is the area of the simulation box, $\mathbf{F}_{ij}^{\mathrm{P}}$ is the pair-wise interparticle force between all particles and $\mathbf{F}_k$ are forces due to rigid-body constraints on all particles.

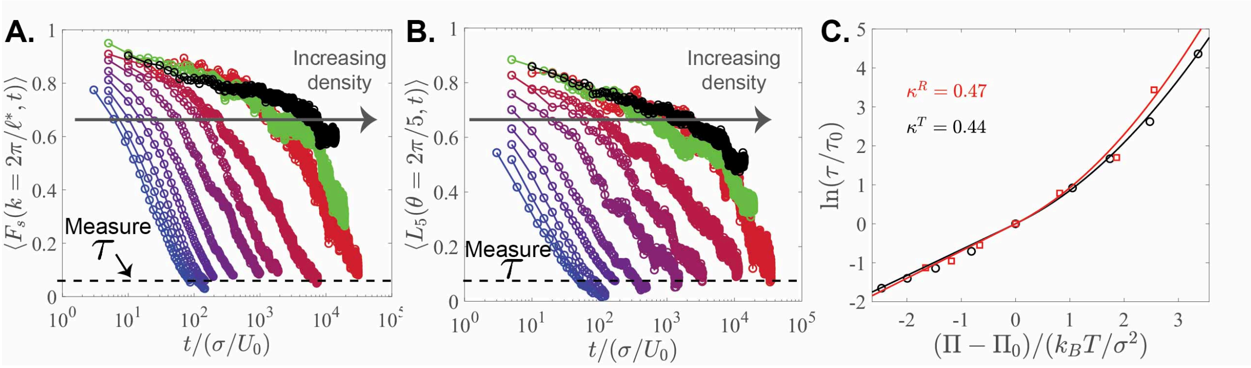


**Figure 2.14:** (A) Dynamic structure factor, $F_s(k = 2\pi/\ell^*, t)$, and (B) angular dynamic structure factor, $L_5(\theta = 2\pi/5, t)$, as a function of time for a passive 2D suspension of polydisperse spherocylinders. Different colors correspond to simulations at varying densities, and $\ell^*$ is the length associated with the first peak of the static structure factor. (C) Relaxation time calculated from translational and angular dynamic structure factors shows Arrhenius and super-Arrhenius crossover behaviors with respect to pressure $\Pi$.

The active force is implemented by imposing an external body force of constant magnitude along the semi-major body axis of the spherocylinder. Given an orientation of a spherocylinder, $\mathbf{q}(\theta_i)$, the active force is defined as $\mathbf{F}_i^{\text{act}}(\theta_i) = \zeta U_0 \mathbf{q}(\theta_i)$, where $U_0$ is the magnitude of the active velocity (see Fig. 2.13). For simplicity, we did not include translational Brownian motion in the active spherocylinder simulations. Therefore, the particles translate due to the active force and reorient due to rotational noise $\mathbf{L}_i^{\text{B}}$. In our simulations, we vary the Péclet number $Pe = U_0\tau_{\text{R}}/\sigma$ (as previously defined) and the density of particles. As before, all pair and wall interactions are modeled with a WCA potential [59] with a well depth of $\epsilon$. For active spherocylinder simulations, the parameter $\epsilon$ is adjusted with activity $Pe$ such that the nondimensional number $F^{\text{act}}\sigma/\epsilon = 1$ remains fixed. This ensures that the particles remain hard and stiff at larger activities; otherwise, an increase of $F^{\text{act}}\sigma/\epsilon$ causes the effective particle size to decrease, where each collision gives rise to increasingly large overlaps for increasing $Pe$ [65]. All of our simulations are performing using a system of $N = 64 \times 64$ particles, and adjusting the box size to achieve the target area density.

Figure 2.15 shows the dynamic translational and rotational structure factors for active spherocylinder systems as a function of density. Figure 2.15C shows the orientational and relaxation times as a function of the pressure $\Pi$ for two different $Pe$. In summary, we find that the active spherocylinder system exhibits crossover between the Arrhenius and super-Arrhenius behaviors around an onset density as in the case of passive systems.

### 3.3 Swarming behaviors: ABPs vs. Spherocylinders

As can be seen from the relaxation behaviors described in previous sections, the onset pressure indicates the state of the active systems consisting of ABPs and active spherocylinders. For packing fractions below the onset pressure the suspensions exist in an active liquid state, and increasing densities beyond the onset pressure results in the active glassy regime. However, there exist significant and important differences in the nature of the active liquid state between the ABPs and active spherocylinders. As can be seen in Fig. 2.16A, the ABP system consisting of hard disks does not exhibit any swarming behaviors of bacterial colonies. In contrast, systems of active spherocylinders exhibit significant swarming (Fig. 2.16B) as found in the real bacterial colonies. This is simply due to the fact that there exist no flocking or swarming behaviors in a homogeneous system devoid of any aligning interactions [45], which is the case for ABPs. However, in the case of spherocylinders,

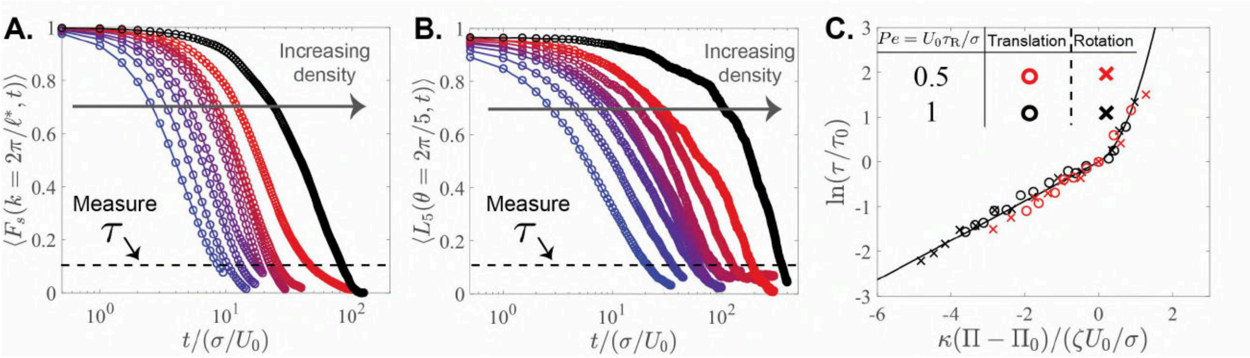


**Figure 2.15:** (A) Dynamic structure factor, $F_s(k = 2\pi/\ell^*, t)$, and (B) angular dynamic structure factor, $L_5(\theta = 2\pi/5, t)$, as a function of time for an active 2D suspension of polydisperse spherocylinders at $Pe = 0.5$. Different colors indicate simulations conducted at varying densities, and $\ell^*$ is the length associated with the first peak of the static structure factor. (C) Translational relaxation time (circles) and angular relaxation time (crosses) calculated from the dynamic structure factors in (A) and (B), for two values of activity $Pe = 0.5$ (red) and $Pe = 1$ (black). The mechanical pressure is scaled with the energy scale: $\kappa^{\mathrm{T}} = 0.20, \kappa^{\mathrm{R}} = 0.15$ for $Pe = 0.5$, and $\kappa^{\mathrm{T}} = 0.24, \kappa^{\mathrm{R}} = 0.30$ for $Pe = 1$.

the inter-spherocylinder interactions mediated by the WCA potential provides overall alignment interactions, thus resulting in flocking. This important difference makes spherocylinder systems ideal for testing the motility induced buckling mechanisms that will be discussed in the following Chapter III.

## 4. DF theory for *P. aeruginosa* colonies

We now discuss the applicability of DF theory to our experiments on *P. aeruginosa* colonies. To this end, time lapse confocal microscopy is conducted at single-cell resolution to obtain displacements and flow fields of the colonies (see SI Movie S7 for representative images). We then obtain dis-

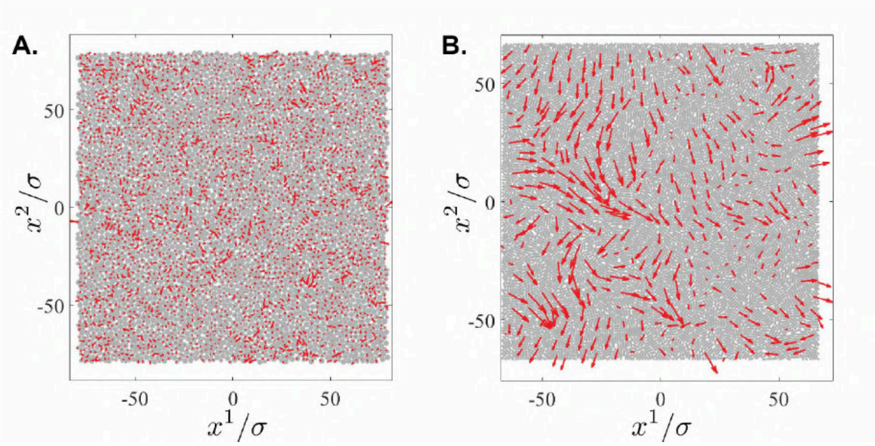


**Figure 2.16:** Nature of swarming behaviors in (A) ABP and (B) spherocylinderical systems. The particles are rendered in gray, while the red arrows correspond to the local velocity vectors. Collective swarms are apparent for active spherocylinders but not for ABPs.

placements of individual bacteria by using an open-source particle-tracking software, SuperSegger [66]. A typical trajectory analysis can be seen in SI Movie S8. By tracking single-cell trajectories, we can compute with high accuracy the density and the dynamic structure factor of the colony (Fig. 2.19A) for varying density. Figure 2.19B shows that the relaxation time of the colony increases when increasing the density of the colony. Note that the relaxation times in experiments is given by the timescale corresponding to the decay of the correlation function $F_s(\mathbf{k}, t)$ to $1/e$ of its initial value.

To test the applicability of the DF theory as extended in (2.20) to bacterial colonies, we need a measurement of the mechanical pressure and not the colony density. Because a direct measurement of the mechanical pressure of bacterial colonies is experimentally challenging, we calculate the cell densities and use a modified equation of state[5] for ellipses to obtain the corresponding pressures [67]. It is known that free-volume theory yields the pressure near close packing to be of the form

$$\Pi = nk_{\mathrm{B}}T\Big(\frac{6}{1-\phi/\phi_{\mathrm{J}}}\Big), \tag{2.29}$$

where $\phi_{\mathrm{J}}$ is the jamming density [67]. To address twitching bacteria where there is no thermal energy $k_{\mathrm{B}}T$, we replace the ideal gas pressure $nk_{\mathrm{B}}T$ with the pressure scale $n\zeta U_0\sigma$, inspired by recent works on active systems [68], which leads to the following modified equation of state

$$\Pi = n\zeta U_0\sigma\Big(\frac{6}{1-\phi/\phi_{\mathrm{J}}}\Big). \tag{2.30}$$

Based upon analysis of MD simulations of active polydisperse spherocylinder systems, we obtain proficient fitting with the parameter $\phi_J = 0.94$ as shown in Fig.2.17. We use this modified equation of state to convert bacterial cell densities to mechanical pressures in our experiments.

Figure 2.19C shows experimental relaxation times of bacterial colonies as a function of pressure using the modified $\Pi(\phi)$ relation in (2.30). We then obtain the energy scale $\kappa_\sigma$, liquid activation energy $E_a$ and the onset pressure $\Pi_0$ by fitting the functional forms in (2.20) and with the experimental relaxation times in Fig. 2.19C. We note that there exist reasonably large errors associated with indirect calculation of the pressure due to the inherent fluctuations in cell density arising from cell division (largest relaxation times were of the order of time of cell division, $\sim 50-70$ min). However, inspections of the bacterial colonies at various densities vividly show swarming and glassy behaviors at pressures (or densities) below the obtained onset pressure (or onset density). This indicates that the onset pressure obtained by fitting the relaxation times is a reasonable estimate of the crossover from swarming to glassy state. Despite many approximations relating to the pressure-density relations, all of the observations, including dynamical heterogeneity, clear indications of facilitated excitations, and the fit of the relaxation time data reveal that the extended DF theory is useful for interpreting the state of the bacterial colony.

[5] Since we do not have a direct way of measuring the pressures in bacterial systems due to both experimental limitations and cell division, we use a modified equation of state as described in (2.30) to be able to apply the DF theory to relaxation times obtained for bacterial colonies in experimental systems. In this case, we are inspired by the work of A. Donev and co-workers who performed an extensive analysis of the equation of state for ellipses [67]. In particular, it is found that (2.29) obtained from free-volume theory provides excellent predictions for pressures close to jamming points, while scaled particle theory yields accurate predictions at lower packing fractions. However, the same work also shows that (2.29) provides a reasonable approximation even at lower packing fractions. Therefore, in our comparison of the DF theory for experiments, we use the modified version of (2.29) as given in (2.30). This approximation appears to be reasonable from our analysis of the $\Pi(\phi)$ vs. $\phi$ curves for active spherocylinders, as shown in Fig. 2.17. Furthermore, these severely crude approximations still appear to enable the expected relaxation times from the theory to agree with the measured times as we will see below.

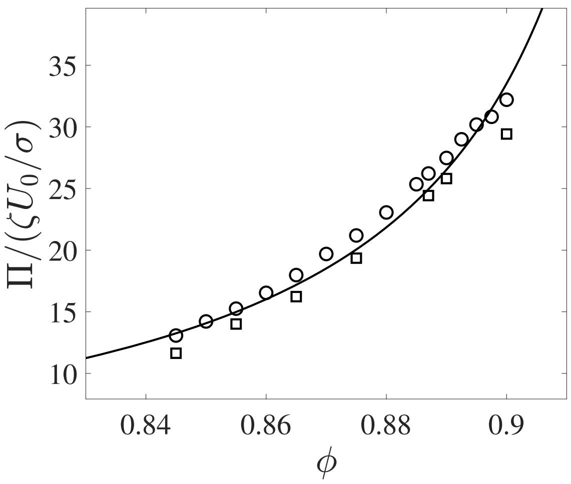


**Figure 2.17:** Mechanical pressure as a function of area fraction calculated via (2.26) in MD simulations of active polydisperse spherocylinders for $Pe = 1$ (circles) and $Pe = 10$ (squares). The solid curve is the modified free-volume relation in (2.30) with $\phi_J = 0.94$. This is used to convert bacterial densities in experiments to corresponding mechanical pressures.

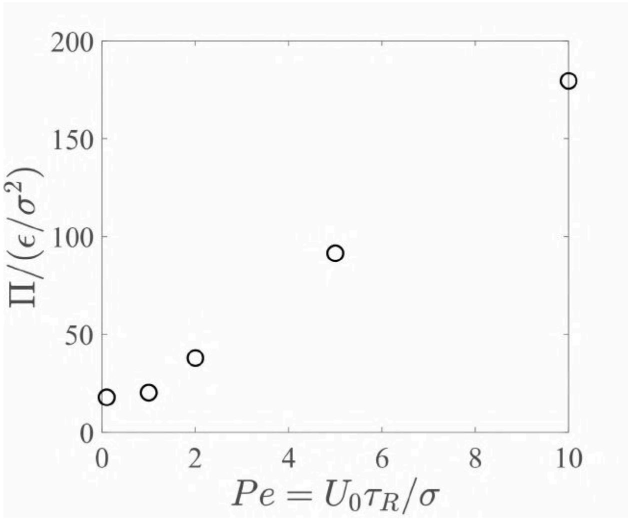


**Figure 2.18:** Pressure calculated via (2.26) in MD simulations of active polydisperse spherocylinders with $\phi = 0.87$ for different $Pe = U_0\tau_R/\sigma$. Here, the pressure is scaled with the absolute simulation units $\epsilon/\sigma^2$, where $\epsilon$ is the interparticle WCA pair potential energy scale.

In summary, results from molecular simulations and experiments demonstrate that DF theory and its extensions enable quantitative prediction of the state of the bacterial colony. Figures 3B and 3C of the main text show a dynamical state diagram that determines the state of the colony (swarming vs glassy) as a function of motility strength and cell density. The crossover pressure (or density), referred as the onset pressure, demarcates the onset between swarming and glassy states and plays a significant role in regulating the mechanism by which bacterial monolayers buckle out of plane, which we proceed to analyze in Chapter III.

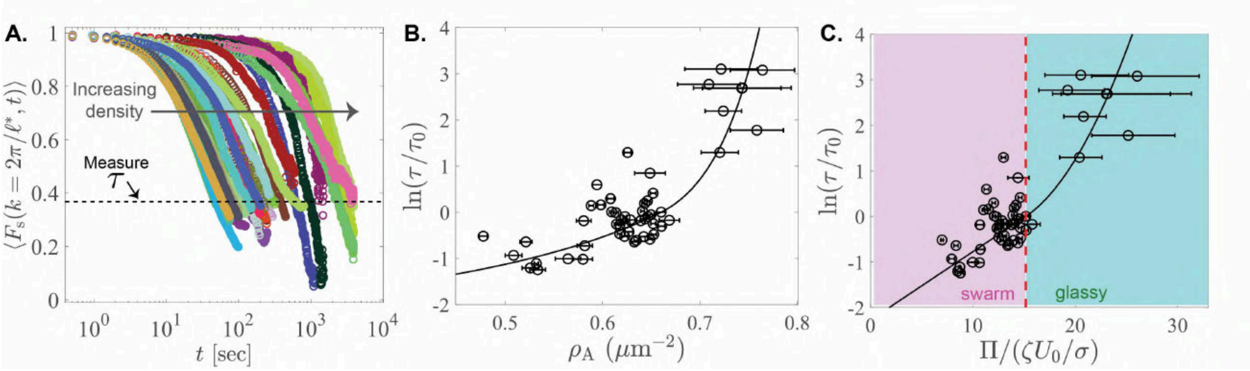


**Figure 2.19:** (A) Dynamic structure factor of *P. aeruginosa* colonies, $F_s(k = 2\pi/\ell^*, t)$, across a range of densities. (B) Relaxation times as a function of cell density; the solid curve is our prediction from our extended DF theory, where (2.30) was used to convert between cell density and pressure. (C) Relaxation times as a function of pressure using the relation (2.30) that converts cell density to pressure. The onset density or the onset pressure demarcates the swarming and glassy states of the colony.

## Chapter III

# MECHANICS OF BACTERIAL COLONIES

We have thus far focused on the behavior of dense bacterial colonies where glassy-like signatures are observed. We now turn our attention to more dilute colonies where collective swarms are present, which may result in buckling. As described in Chapter I, wild type colonies exhibit 2D-to-3D transitions of individual bacteria at the migrating front correlated with collective swarming motility. Non-motile species or colonies at high density do not show any swarming behaviors, and transitions into the third dimension occur in the colony interiors. As mentioned before, transitions in non-motile or dense colonies arise from growth induced stresses that lead to buckling [1–7], which occur on a time scale much larger than the motility-dependent transitions below the onset density of glassy dynamics. In this chapter, we develop a 2D fluid film theory to model active bacterial monolayers in the swarming state, and predict the motility-induced buckling mechanisms leading to 3D transitions.

## 1. Bacterial colony monolayers as active fluid shells

In this section, we analyze the out-of-plane motion of the bacterial monolayers as a fluid membrane. As can be seen from both experiments and particularly the simulations, the active swarming state of the bacterial colony below the onset pressure (or onset density) is reminiscent of a two-dimensional fluid, where the in-plane flows are generated by the inherent motile or self-propelling nature of bacteria. In deed, these types of flows have been previously observed in other bacterial colonies such as *Bacillus subtilis* [69]. Such flows were analyzed theoretically using two-dimensional incompressible Navier-Stokes equations in conjunction with an active velocity functional that models the collective swarming nature of the colony [69]. The encompassing continuum theory in the plane of the bacteria reproduced many of the experimental features, including turbulence-like phenomena of the colonies at the meso-scale [69–71].

The aforementioned studies show that dense bacterial colonies can be modeled as 2D incompressible Newtonian fluids with in-plane velocity gradients, and therefore viscous shear stresses. It is possible that an in-plane non-zero shear stress in a membrane leads to out-of-plane buckling. This can be understood by analyzing the following simple scenario. Consider the case of velocity gradient in the plane of the membrane corresponding to a pure Couette flow with a non-zero shear rate $\dot{\gamma}$. In this case, the 2D velocity gradient in the Cartesian coordinate system is given by

$$\boldsymbol{\nabla}\mathbf{v} = [0, \dot{\gamma}; 0, 0], \tag{3.1}$$

which has two eigenvalues given by $+\dot{\gamma}$ and $-\dot{\gamma}$, thus containing an eigenvector along which there exists pure compression. If the system is incompressible, this compression can then lead to an out-of-plane deformation of the membrane in the direction of the eigenvector, leading to buckling of the membrane. As mentioned before, an active swarming state of the colony exhibits behaviors

reminiscent of a Newtonian fluid with inhomogeneous flows, and therefore can sustain shear gradients. In such a case, there exist compressive stresses corresponding to negative eigenvalues of the strain rates, which may cause buckling of the bacterial colony thereby leading to out-of-plane growth of the colony.

Detailed analysis of the coupling between in-plane velocity gradients and out-of-plane deformations, and the ensuing rate-dependent or motility-induced buckling instabilities, requires a theoretical framework corresponding to fluid membranes (or shells) capable of out-of-plane deformations. Such couplings are very common in related problems in biology, especially in the field of biological membranes, which behave as a Newtonian fluid in the plane and resist elastically out-of-plane [72]. Inspired by the continuum theories used to analyze arbitrarily curved and deforming lipid membranes [73–79], we propose a novel theoretical framework for analyzing the in-plane and out-of-plane behaviors of bacterial colonies.

# 2. Continuum membrane theory

As mentioned before, we assume that the bacterial colonies are sufficiently dense in their swarming state such that they behave as a continuum two-dimensional fluid. We analyze the motion of the colony by considering the surface connecting the mid-points of the bacterial monolayer as shown in Fig. 3.1. The coupling between in-plane flows and out-of-plane deformations of the monolayer can be studied using the well known Kirchhoff-Love shell theory [80], and requires the general framework of differential geometry. In what follows, we consider the theoretical formalism outlined in Sahu et. al. [74] for lipid membranes in the differential geometric setting, and derive the balance laws governing the motion of the monolayer. We note that the analysis of bacterial colonies as a continuum is valid only for studying the onset of motility-induced buckling. The concept of a continuum is broken as one or more of the bacteria detach from the first monolayer and enter into the second layer.

## *2.1 Differential geometry and kinematics of membranes*

To begin, the reader is assumed to possess knowledge of differential geometry [81, 82], and Einstein's summation convention standard in continuum mechanics. Moreover, we only describe those parts of the theory of arbitrarily deforming membranes that are of use in the current work. For a detailed description containing a general theoretical development concerning irreversible thermodynamics and mechanics of arbitrarily curved and deforming surfaces, see [74].

Let the mid-plane of the bacterial monolayer at any time be represented by a position vector $\mathbf{x}(\theta^\alpha, t)$, where $\theta^\alpha$ is a parametric representation of the surface. Given the position of the surface

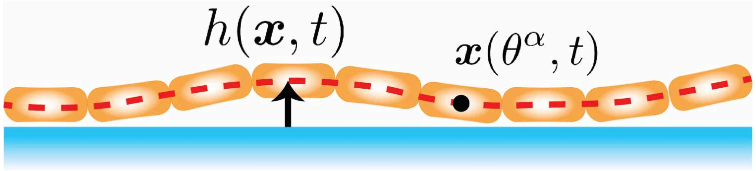


**Figure 3.1:** A schematic of the bacterial monolayer and the substrate (blue). Also, shown is a representation of the surface $\mathbf{x}(\theta^\alpha, t)$ (red dashed line) representing the mid-points of the bacterial monolayer and a height fluctuation with respect to the substrate. Single bacteria can overcome adhesion forces with the substrate and grow into a second layer.

$\mathbf{x}$, the tangent vectors to the surface at any point are given by

$$\mathbf{a}_\alpha = \mathbf{x}_{,\alpha}, \quad \alpha \in \{1, 2\}, \tag{3.2}$$

where $(\cdot)_{,\alpha}$ denotes the partial derivative with respect to $\theta^\alpha$, *i.e.,* $\frac{\partial(\cdot)}{\partial\theta^\alpha}$. The normal to the surface at any point is $\mathbf{n} := \mathbf{a}_1 \times \mathbf{a}_2/|\mathbf{a}_1 \times \mathbf{a}_2|$, which together with the tangent vectors $\mathbf{a}_\alpha$ forms a natural basis $\{\mathbf{a}_1, \mathbf{a}_2, \mathbf{n}\}$ to express any vector on the surface.

The tangent vectors make up the metric tensor components $a_{\alpha\beta} = \mathbf{a}_\alpha \cdot \mathbf{a}_\beta$. The contravariant metric components are given by $a^{\alpha\beta} = (a_{\alpha\beta})^{-1}$. The contravariant basis vectors $\mathbf{a}^\alpha$ can be obtained by raising the indices with the contravariant metric components as $\mathbf{a}^\alpha = a^{\alpha\beta}\mathbf{a}_\beta$. Any vector $\mathbf{w}$ on the surface can be described in the basis $\{\mathbf{a}_1, \mathbf{a}_2, \mathbf{n}\}$ or $\{\mathbf{a}^1, \mathbf{a}^2, \mathbf{n}\}$ as

$$\mathbf{w} = w^\alpha \mathbf{a}_\alpha + w\mathbf{n} = w_\alpha \mathbf{a}^\alpha + w\mathbf{n}, \tag{3.3}$$

where $w^\alpha$ or $(w_\alpha)$ are the contra-variant (or co-variant) components along the corresponding tangent vectors related by

$$\begin{aligned} w^\alpha &= a^{\alpha\beta} w_\beta, \\ w_\alpha &= a_{\alpha\beta} w^\beta, \end{aligned} \tag{3.4}$$

and $w$ is the component in the normal direction. We note that, the metric components $a^{\alpha\beta}$ and $a_{\alpha\beta}$ can be used to raise or lower the indices of the components of vectors and tensors. The covariant derivatives of the co-variant and contravariant vector components $w_\lambda$ and $w^\lambda$ are

$$w_{\lambda;\alpha} = w_{\lambda,\alpha} - \Gamma^\mu_{\lambda\alpha} w_\mu \tag{3.5}$$

and

$$w^\lambda_{;\alpha} = w^\lambda_{\alpha} + \Gamma^\lambda_{\mu\alpha} w_\mu, \tag{3.6}$$

where $\Gamma^\alpha_{\lambda\mu}$ are Christoffel symbols of the second kind given by

$$\Gamma^\alpha_{\lambda\mu} = \frac{1}{2} a^{\alpha\delta}(a_{\delta\lambda,\mu} + a_{\delta\mu,\lambda} - a_{\lambda\mu,\delta}). \tag{3.7}$$

To describe the deformation of the interface, one also needs the curvature tensor components defined as $b_{\alpha\beta} = \mathbf{n} \cdot \mathbf{x}_{,\alpha\beta}$. The metric components and curvature components together define the mean curvature $H$ and the Gaussian curvature $K$ as

$$H = \frac{1}{2} a^{\alpha\beta} b_{\alpha\beta} \tag{3.8}$$

and

$$K = \frac{1}{2} \epsilon^{\alpha\beta} \epsilon^{\lambda\mu} b_{\alpha\lambda} b_{\beta\mu}, \tag{3.9}$$

where $\epsilon^{\alpha\beta}$ is the permutation tensor with components

$$\epsilon^{11} = \epsilon^{22} = 0, \quad \epsilon^{12} = -\epsilon^{21} = \frac{1}{\sqrt{\det(a_{\alpha\beta})}}, \tag{3.10}$$

and $\det(\cdot)$ denotes the determinant of the corresponding tensor $(\cdot)$.

In what follows, we describe the dynamics of the surface. The velocity $\mathbf{v}$ of any point on the surface is given by

$$\mathbf{v} = \frac{d\mathbf{x}}{dt} = \dot{\mathbf{x}} = v^\alpha a_\alpha + v\mathbf{n}, \tag{3.11}$$

where $v^\alpha$ are the contravariant components along the tangent basis and $v = \mathbf{v} \cdot \mathbf{n}$ is the component in the normal direction. In (3.11), $\frac{d}{dt}(\cdot)$ denotes the material time derivative given by

$$\frac{d}{dt}(\cdot) := \frac{\partial}{\partial t}(\cdot) + v^\alpha (\cdot)_{,\alpha}, \tag{3.12}$$

and $\dot{(\cdot)}$ denotes a short hand notation for the material time derivative. The material time derivative of the metric tensor components correspond to the velocity gradients on arbitrary surfaces:

$$\dot{a}_{\alpha\beta} = v_{\beta;\alpha} + v_{\alpha;\beta} - 2v b_{\alpha\beta}, \tag{3.13}$$

which will be useful in defining the in-plane Newtonian-fluid behaviors, relating in-plane shear stresses and velocity gradients.

Let us also introduce the Jacobian $J$ that describes the areal dilation or contraction of the membrane as

$$J = \frac{\mathrm{d}a}{\mathrm{d}A}, \tag{3.14}$$

where $\mathrm{d}a$ and $\mathrm{d}A$ are the current and referential area of the surface. Given the metric $a_{\alpha\beta}$ and its time derivative in (3.13), the time derivative of the Jacobian can be obtained as

$$\frac{\dot{J}}{J} = \frac{1}{2} a^{\alpha\beta} \dot{a}_{\alpha\beta} = v^\alpha_{;\alpha} - 2vH. \tag{3.15}$$

If the material is incompressible, $J = 1$ everywhere and its time derivative is zero.

## 2.2 Balance laws for fluid membranes

We now describe the balance laws governing the motion of the surface. We provide only the local form of the balance laws for mass, and linear momentum. For obtaining the local forms from the global form of the balance laws, see [74].

Given a mass density $\rho(\mathbf{x}, t)$, the local form of the mass balance is given by

$$\dot{\rho} + \left(v^\alpha_{;\alpha} - 2vH\right)\rho = 0. \tag{3.16}$$

For an incompressible fluid, the mass balance reduces to

$$v^\alpha_{;\alpha} - 2vH = 0. \tag{3.17}$$

The momentum balance for any curved surface can be written as

$$\mathbf{T}^\alpha_{;\alpha} + \rho \mathbf{b} = \rho \dot{\mathbf{v}}, \tag{3.18}$$

where $\mathbf{b}$ is the body force. $\mathbf{T}^\alpha$ are the stress vectors and are related to traction vector (or force per unit length) $\mathbf{t}(\mathbf{x}_b, t; \boldsymbol{\nu})$ on a line boundary of the surface with outward normal $\boldsymbol{\nu}$ by

$$\mathbf{t}(\mathbf{x}, t; \boldsymbol{\nu}) = \mathbf{T}^\alpha \nu_\alpha, \tag{3.19}$$

where $\nu_\alpha$ are the components of the outward normal to the line boundary. Without loss of generality, the traction vectors $\mathbf{T}^\alpha$ can be decomposed into

$$\mathbf{T}^\alpha = N^{\alpha\beta} \mathbf{a}_\beta + S^\alpha \mathbf{n}, \tag{3.20}$$

where $N^{\alpha\beta}$ and $S^{\alpha}$ are the components of the traction vector in basis $\{\mathbf{a}_1, \mathbf{a}_2, \mathbf{n}\}$. Given (3.20) and (3.19), the total traction can be rewritten as

$$\mathbf{t} = \mathbf{T}^T \boldsymbol{\nu}, \tag{3.21}$$

where $\mathbf{T}$ is the total stress tensor given by

$$\mathbf{T} = N^{\alpha\beta}\mathbf{a}_\alpha \otimes \mathbf{a}_\beta + S^\alpha \mathbf{a}_\alpha \otimes \mathbf{n}. \tag{3.22}$$

In an analogous manner to the traction analysis, the total moment on a line boundary can be written as $\mathbf{M} = \boldsymbol{\mu}^T\boldsymbol{\nu}$, with $\boldsymbol{\mu}$ being the moment tensor represented in the component form as

$$\mu = -M^{\alpha\beta}\mathbf{a}_\alpha \otimes \mathbf{a}_\beta.\text{[1]} \tag{3.23}$$

In this case, the balance of angular momentum dictates that

$$\begin{aligned} \sigma^{\alpha\beta} &:= N^{\alpha\beta} - b^\beta_\mu M^{\mu\alpha} \quad \text{is symmetric} \\ S^\alpha &= -M^{\beta\alpha}_{;\beta}, \end{aligned} \tag{3.24}$$

where $b^\beta_\mu = b^{\beta\gamma}a_{\gamma\mu}$.

The balance of momentum (3.18) can now be written in component form along the tangent vectors and the normal direction as

$$\rho b^\alpha + N^{\lambda\alpha}_{;\lambda} - S^\lambda b^\alpha_\lambda = \rho\dot{\mathbf{v}}\cdot\mathbf{a}^\alpha \tag{3.25}$$

and

$$\rho b_{\mathrm{n}} + N^{\alpha\beta}b_{\alpha\beta} + S^\alpha_{;\alpha} = \rho\dot{\mathbf{v}}\cdot\mathbf{n}, \tag{3.26}$$

respectively, where $b^\alpha = \mathbf{b}\cdot\mathbf{a}^\alpha$ and $b_{\mathrm{n}} = \mathbf{b}\cdot\mathbf{n}$ are the components of the body force in the tangential and the normal directions. Equations (3.25) and (3.26) correspond to the in-plane and out-of-plane equations of motion of the surface, respectively.

In the ensuing analysis, we assume that inertial forces in and out-of-plane are negligible compared to the viscous forces in the plane of the surface and the drag forces imposed by the solvent and the substrate around the bacteria. In this case, the balance equations (3.25) and (3.26) can be reduced to

$$\rho b^\alpha + N^{\lambda\alpha}_{;\lambda} - S^\lambda b^\alpha_\lambda = 0, \tag{3.27}$$

and

$$\rho b_{\mathrm{n}} + N^{\alpha\beta}b_{\alpha\beta} + S^\alpha_{;\alpha} = 0. \tag{3.28}$$

[1] Note that we recapitulate here the full theory developed for lipid bilayers, which resit bending elastically resulting in bending moments due to changes in curvature. However, such moments may not be relevant to understanding out-of-plane deformations of bacterial monolayers, as they lack bending resistance and the main governing force that resists the height fluctuations are primarily due to adhesion. Even then, the consequences of balance of angular momentum imposing the symmetry of the stresses $\sigma^{\alpha\beta}$ still remain true.

### *2.3 Constitutive relations: fluidity, elastic bending and adhesion*

We now propose constitutive behaviors that connect the stresses and moments to the kinematic variables. We provide a brief overview of the constitutive relations governing the surface, and we refer the reader again to [74] for a full description of the derivations inspired by the framework of irreversible (or non-equilibrium) thermodynamics. To that end, we define a Helmholtz free energy (per unit mass) $\psi$ that depends on the metric and curvature tensor components $a^{\alpha\beta}$ and $b^{\alpha\beta}$, i.e.,

$$\psi = \psi(a_{\alpha\beta}, b_{\alpha\beta}, T).^{2} \tag{3.29}$$

Given (3.29), the over all stresses and the moments can be derived to be of the form

$$\sigma^{\alpha\beta} = \rho\left(\frac{\partial\psi}{\partial a_{\alpha\beta}} + \frac{\partial\psi}{\partial a_{\beta\alpha}}\right) + \pi^{\alpha\beta} \tag{3.30}$$

and

$$M^{\alpha\beta} = \frac{\rho}{2}\left(\frac{\partial\psi}{\partial b_{\alpha\beta}} + \frac{\partial\psi}{\partial b_{\beta\alpha}}\right), \tag{3.31}$$

see [74]. In (3.30), $\pi^{\alpha\beta}$ denote the viscous stresses in the plane of the membrane and are related to the in-plane velocity gradients through $\dot{a}_{\alpha\beta}$ as

$$\begin{aligned} \pi^{\alpha\beta} = &= \eta\, a^{\alpha\gamma} a^{\beta\mu} \dot{a}_{\gamma\mu} + \xi\, a^{\alpha\beta} a^{\gamma\mu} \dot{a}_{\gamma\mu} \\ &= \eta\, a^{\alpha\gamma} a^{\beta\mu} \dot{a}_{\gamma\mu} + \xi\, a^{\alpha\beta}\big(2v^{\mu}_{;\mu} - 4vH\big), \end{aligned} \tag{3.32}$$

where $\eta$ and $\xi$ are the shear and bulk viscosities, respectively. If the in-plane fluid behavior is assumed to be incompressible, the last term on the right-hand side of $(3.32)_2$ is zero due to (3.17). In cases where the in-plane fluid behavior is non-Newtonian, the constitutive equation for the viscous stress should include a dependence of the shear strain rate $\dot{\gamma}$ in the shear viscosity, i.e., $\eta(\dot{\gamma})$.

We now evaluate the stresses and moments for a surface whose in-plane behavior is that of an incompressible Newtonian fluid, and which resists bending elastically. To this end, the form of Helmholtz energy that describes such a behavior is the Helfrich energy (as applicable for lipid membranes in general) supplemented with an area constraint. In this case, the free energy of the system is given by

$$\begin{aligned} \int \rho\psi(a_{\alpha\beta}, b_{\alpha\beta}, T)\mathrm{d}a &= \int (k_{\mathrm{b}}H^2 + k_{\mathrm{g}}K)\mathrm{d}a + \int \lambda(J-1)\mathrm{d}A \\ &= \int (k_{\mathrm{b}}H^2 + k_{\mathrm{g}}K)\mathrm{d}a + \int \lambda\frac{(J-1)}{J}\mathrm{d}a, \end{aligned} \tag{3.33}$$

where $\lambda(\mathbf{x}, t)$ is the Lagrange multiplier that maintains the constraint $J = 1$.

For the free energy of the form given in (3.33), using (3.30) and (3.31) the in-plane stresses and moments can be obtained as

$$\sigma^{\alpha\beta} = \lambda a^{\alpha\beta} + k_{\mathrm{b}}H^2 a^{\alpha\beta} - 2k_{\mathrm{b}}H b^{\alpha\beta} - k_{\mathrm{g}}K a^{\alpha\beta} + \pi^{\alpha\beta} \tag{3.34}$$

and

$$M^{\alpha\beta} = k_{\mathrm{b}}H a^{\alpha\beta} + k_{\mathrm{g}}(2H a^{\alpha\beta} - b^{\alpha\beta}). \tag{3.35}$$

[2] Note that the dependence of the behavior of bacterial colonies on temperature is irrelevant to our problem.

It can be readily seen from (3.34) and (3.35) that for a system with no bending rigidity in relevance to bacterial monolayers, the in-plane stresses reduce to that of a Newtonian fluid and the moments are zero.

Bacterial systems interact primarily via adhesion with the substrate, and bacteria must overcome adhesion forces to be able to grow into the second layer. Therefore, it is important to account for adhesion interaction forces, which usually enter as the body forces in the surface equations since they do not contribute to the internal energy of the monolayer. Assuming that the adhesion energy is of the form

$$F_{\mathrm{ad}} = \frac{1}{2} E_{\mathrm{ad}} \left[\mathbf{x}(\theta^\alpha, t) - \mathbf{x}_s) \cdot (\mathbf{x}(\theta^\alpha, t) - \mathbf{x}_s)\right], \tag{3.36}$$

with $\mathbf{x}_s$ being the substrate position constrained to be fixed everywhere, and $E_{\mathrm{ad}}$ the adhesion modulus indicating the strength of the interactions, the body force on the surface is given by

$$\rho \mathbf{b} = -\frac{\delta F_{\mathrm{ad}}}{\delta \mathbf{x}}, \tag{3.37}$$

where the right-hand side of (3.37) is the variational derivative.

With (3.34) and (3.35), the equations of motion for the surface along the tangential and normal directions (3.27) and (3.28), are reduced to

$$\underbrace{\lambda^{;\alpha}}_{\text{tension gradients}} + \underbrace{\pi^{\beta\alpha}_{;\beta}}_{\text{viscous gradients}} + \rho b^\alpha = 0, \tag{3.38}$$

and

$$\underbrace{\rho b_{\mathrm{n}}}_{\text{cell-substrate adhesion}} + \underbrace{2\lambda H}_{\text{tension-curvature coupling}} + \underbrace{\pi^{\alpha\beta} b_{\alpha\beta}}_{\text{viscous-curvature coupling}} \underbrace{-k_{\mathrm{b}}\Delta H - 2k_{\mathrm{b}} H(H^2 - K)}_{\text{bending}} = 0, \tag{3.39}$$

respectively, where the operator $\Delta(\cdot) := (\cdot)_{;\beta\alpha} a^{\alpha\beta}$ is the surface Laplacian. The in-plane equations in (3.38) correspond to the Stokes equations on arbitrarily curved surfaces, which balance the surface tension (or negative surface pressure) and viscous stress gradients. The equation along the normal (3.39) is an extension of the usual Young-Laplace equation for surfaces, taking into account additional forces from adhesion, bending and viscous-curvature coupling. The term $\pi^{\alpha\beta} b_{\alpha\beta}$ corresponds to the viscous-curvature coupling forces and present non-trivial coupling between viscous flows in the surface and out-of-plane deformation, particularly to cases such as active systems, which sustain velocity gradients and therefore viscous stresses. The coupling between curvature and viscous forces can also be seen explicitly from the in-plane viscous stress gradients $\pi^{\beta\alpha}_{;\beta}$ and the viscous-curvature coupling terms $\pi^{\alpha\beta} b_{\alpha\beta}$ given by

$$\pi^{\beta\alpha}_{;\beta} = 2\eta[d^{\beta\alpha}_{;\beta} - v_{,\beta} b^{\beta\alpha} - 2vH_{,\beta} a^{\beta\alpha}] + \xi a^{\beta\alpha}(v^{\mu}_{;\mu} - 2vH)_{;\beta}, \tag{3.40}$$

and

$$\pi^{\alpha\beta} b_{\alpha\beta} = 2\eta[b^{\alpha\beta} d_{\alpha\beta} - v(4H^2 - 2K) + 2\xi H(v^{\mu}_{;\mu} - 2vH), \tag{3.41}$$

where

$$d^{\alpha\beta} = \frac{1}{2}(v^{\alpha;\beta} + v^{\beta;\alpha}) \tag{3.42}$$

is the symmetric part of the in-plane velocity gradients in curvilinear coordinate system.

## 2.4 Restrictions to Monge parametrization - small deformations

In what follows, we analyze the system of equations to small deformations about the monolayer to predict the buckling of bacterial monolayers leading to their out-of-plane growth. To this end, we introduce the Monge parametrization given by

$$\mathbf{x} = x^1\mathbf{e}_1 + x^2\mathbf{e}_2 + h(x^1, x^2, t)\mathbf{e}_3 \tag{3.43}$$

where $\mathbf{e}_1$, $\mathbf{e}_2$ and $\mathbf{e}_3$ are the unit vectors in the cartesian coordinate system. Here, $h(x^1, x^2, t)$ is height of the bacterial monolayer for small deformations (see Figure 3.2). Such a mapping preserves one-to-one mapping with the initial surface.

We restrict the analysis to the case of small deformations, where any $O(h^2)$ terms are negligible. The tangential basis vectors are

$$\mathbf{a}_\alpha = \mathbf{e}_\alpha + h_{,\alpha}\mathbf{e}_3. \tag{3.44}$$

The normal is

$$\mathbf{n} \approx \mathbf{e}_3 - h_{,1}\mathbf{e}_1 - h_{,2}\mathbf{e}_2 + O(h^2). \tag{3.45}$$

The metric and curvature tensor components are given by

$$a_{\alpha\beta} \approx \delta_{\alpha\beta} + O(h^2), \tag{3.46}$$

and

$$b_{\alpha\beta} \approx h_{,\alpha\beta} + O(h^2), \tag{3.47}$$

respectively. The mean curvature is

$$H = \frac{1}{2}a^{\alpha\beta}b_{\alpha\beta} = \frac{1}{2}h_{,\alpha\alpha} + O(h^2), \tag{3.48}$$

and the Gaussian curvature is

$$K \approx 0 + O(h^2). \tag{3.49}$$

Moreover, all the Christoffel symbols that provide the co-variant derivatives are all of $O(h^2)$, and therefore do not contribute to the terms in the equations.

The velocity of any point on the surface in the Monge representation (3.43) is given by

$$\begin{aligned}\mathbf{v} = \dot{\mathbf{x}} &= \dot{x}^1\mathbf{e}_1 + \dot{x}^2\mathbf{e}_2 + h_{,1}\dot{x}^1\mathbf{e}_3 + h_{,2}\dot{x}^2\mathbf{e}_3 + h_{,t}\mathbf{e}_3\\ &= \dot{x}^1(\mathbf{e}_1 + h_{,1}\mathbf{e}_3) + \dot{x}^2(\mathbf{e}_2 + h_{,2}\mathbf{e}_3) + h_{,t}\mathbf{e}_3\\ &= v^\alpha\mathbf{a}_\alpha + v\mathbf{n},\end{aligned} \tag{3.50}$$

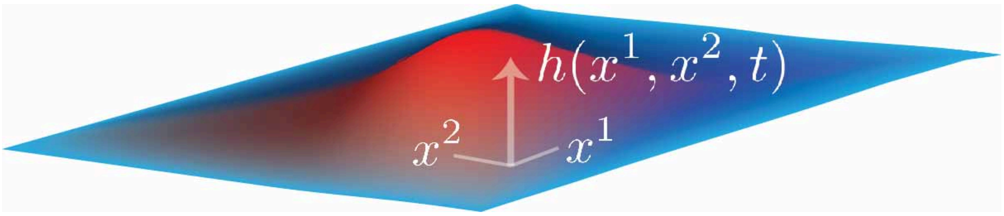


**Figure 3.2:** A schematic of the height field $h(x^1, x^2, t)$ of the bacterial monolayer under small deformations.

where use is made of the tangent vectors from (3.46). One can identify the time derivatives of the $x^1$ and $x^2$ positions as velocities along the tangents in the Eulerian representation, i.e., $v^\alpha(x^1, x^2)$. Furthermore, the normal component of the velocity is given by

$$v = \mathbf{v} \cdot \mathbf{n} = h_{,t}, \tag{3.51}$$

which is simply the change in height with respect to time. The velocities $v^\alpha$ and the height field $h$ remain as unknowns to be solved from the equations of motion.

For the case of an incompressible fluid under small deformations, the in-plane viscous gradients (3.40) and viscous-curvature coupling terms (3.41) reduce to

$$\pi^{\beta\alpha}_{;\beta} = \eta \Delta v^\alpha, \tag{3.52}$$

and

$$\pi^{\alpha\beta} b_{\alpha\beta} = \eta(v^{\alpha,\beta} + v^{\beta,\alpha}) h_{,\alpha\beta}, \tag{3.53}$$

respectively. The adhesion forces for small deformations only involves height field and is given by

$$F_{\mathrm{ad}} = \frac{1}{2} E_{\mathrm{ad}} (h - h_0)^2 \tag{3.54}$$

where $h_0$ is the substrate height and is taken to be zero, *i.e.,* the substrate is in the $x - y$ plane. In this case, the body forces only involve the normal component given by

$$\rho b_{\mathrm{n}} = -E_{\mathrm{ad}} h. \tag{3.55}$$

For an incompressible system undergoing small deformations $h$ that can also sustain arbitrary in-plane velocities $v^\alpha$, the equations of motion, using all the above definitions and simplifications corresponding to the Monge representation, can be reduced to

$$v^\alpha_{,\alpha} = 0, \tag{3.56}$$

$$\lambda^{,\alpha} + \eta \Delta v^\alpha = 0, \tag{3.57}$$

and

$$\lambda \nabla^2 h + \eta(v^{\alpha,\beta} + v^{\beta,\alpha}) h_{,\alpha\beta} - \frac{1}{2} k_{\mathrm{b}} \nabla^2 \nabla^2 h - E_{\mathrm{ad}} h = \zeta_{\mathrm{B}} \frac{\partial h}{\partial t} \tag{3.58}$$

Equations (3.56) and (3.57) simply correspond to the incompressible Navier-Stokes equations in the Stokes approximation, where $\lambda$ is the Lagrange multiplier which enforces the incompressibility condition. As such, the value of tension therefore can depend on the nature of the flows involved in the bacterial colony. Equation (3.58) corresponds to the out-of-plane deformation and contains competitions between surface tension, viscous, bending and adhesion forces. Note that we added a simple form of the bulk drag term in the normal direction. Such a drag term serves to identify the fastest growing modes of deformation that could lead to instabilities. As such, this term does not alter the physics between the competing forces of tension, adhesion, viscous and bending forces.

The equations (3.56), (3.57) and (3.58) also demonstrate that the in-plane equations governing the spatial velocity distributions decouple from the normal equation, and therefore can be solved independently from the out-of-plane equation. However, the equation along the normal shows the influence of in-plane velocity gradients in the out-of-plane deformations by the viscous-curvature coupling term. The decoupling of in-plane velocity from the height field in the in-plane equations, but its influence on the height field, allows us to consider special cases of flows and demonstrate the novel instabilities that can arise from activity inherent in motile bacterial colonies.

# 3. Buckling of active bacterial monolayers

Observations of bacterial monolayers suggest that there exist sustained motility driven (active) flows and corresponding gradients. As mentioned in Section 1, a simple case of an active flow resulting in a constant velocity gradient in the monolayer can lead to a buckling of the monolayer, due to compression along one of its eigenvectors. This active flow driven buckling mechanism can enable bacteria overcome adhesion forces in the monolayer providing an onset for the growth of the bacteria into a second layer. In what follows, we identify such a possibility by considering special cases of linear and non-linear flows including Couette, squeeze, and compressible flows. We demonstrate that these special cases of flows lead to buckling instabilities of the bacterial monolayers nucleating growth in the third dimension.

To investigate the instabilities, we consider linear perturbations to the fields in the equations (3.56), (3.57) and (3.58) and perform linear stability analysis. It appears, as we will show later, that the behavior of bacterial monolayers modeled either as a collection of spherical particles or a polydisperse liquid crystal-like molecules is that of a non-Newtonian fluid. Using molecular simulations, we shall also demonstrate in the subsequent sections that the non-Newtonian behavior is that of a power-law fluid [83]. For the case of small height deformations, the general stress-strain rate relations for an incompressible power-law fluid can be written as

$$\pi^{\alpha\beta} = \eta_0[v^{\alpha,\beta} + v^{\beta,\alpha}]^n, \tag{3.59}$$

where $\eta_0$ is a proportionality constant and $n$ is the exponent. In this case, the viscous in-plane behaviors of the monolayer should be linearized for performing the linear stability analysis. To this end, let $v^\alpha = v_0^\alpha + \epsilon\tilde{v}^\alpha$, where $v_0^\alpha$ is a reference velocity and $\tilde{v}^\alpha$ is a perturbation with $\epsilon$ being a small parameter. The linearized viscous stresses can be written as

$$\pi^{\alpha\beta} = \pi_0^{\alpha\beta} + \epsilon\big[n\eta_0(v_0^{\alpha,\beta} + v_0^{\beta,\alpha})^{n-1}(\tilde{v}^{\alpha,\beta} + \tilde{v}^{\beta,\alpha})\big], \tag{3.60}$$

where

$$\pi_0^{\alpha\beta} = \eta_0[v_0^{\alpha,\beta} + v_0^{\beta,\alpha}]^n \tag{3.61}$$

are the viscous stresses with respect to the reference velocity $v_0^\alpha$. The linearized form of the viscous-curvature coupling terms in the limit of small deformations are given by

$$\pi^{\alpha\beta}b_{\alpha\beta} = \pi_0^{\alpha\beta}h_{,\alpha\beta} + O(\epsilon h), \tag{3.62}$$

where the last term on the right-hand side of (3.62) is negligible due to small height and velocity perturbations.

Given the linearized form of the viscous stresses and the coupling terms, the equation of motion of the monolayer along the normal direction (3.58) will be modified accordingly as

$$\zeta_{\mathrm{B}}\frac{\partial h}{\partial t} = \lambda\nabla^2 h + \pi_0^{\alpha\beta}h_{,\alpha\beta} - \frac{1}{2}k_{\mathrm{b}}\nabla^2\nabla^2 h - E_{\mathrm{ad}}h. \tag{3.63}$$

The in-plane equations of motion remain unchanged.

To perform the stability analysis, consider the height field in terms of its normal modes

$$h(x^1, x^2, t) = \sum_{\mathbf{k}} h_{\mathbf{k}}\exp(ik_\alpha x^\alpha + \omega t), \tag{3.64}$$

where $\mathbf{k} = k_1\mathbf{e}_1 + k_2\mathbf{e}_2 = k^\alpha\mathbf{e}_\alpha$ is the wave-vector, $h_{\mathbf{k}}$ is the amplitude, and $\omega$ is the frequency. As can be seen in (3.64), positive values of $\omega$ lead to an unbounded growth of the height field.

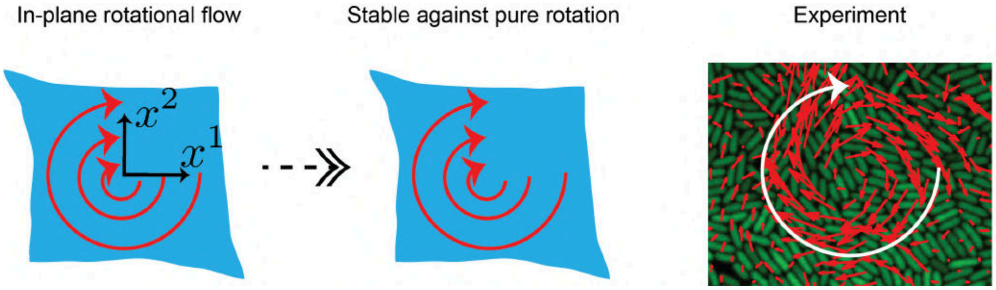


**Figure 3.3:** A schematic representation of the rotational flow field. The right figure shows the presence of rotational flow field in a bacterial monolayer.

Equation (3.63) in terms of the height field normal modes is given by

$$\begin{aligned}\sum_{\mathbf{k}} \zeta_{\mathrm{B}} \omega h_{\mathbf{k}} \exp(ik_\alpha x^\alpha + \omega t) = \sum_{\mathbf{k}} [-E_{\mathrm{ad}} - \lambda k^2 - \frac{1}{2} k_{\mathrm{b}} k^4] h_{\mathbf{k}} \exp(ik_\alpha x^\alpha + \omega t) \\ - \sum_{\mathbf{k}} \pi_0^{\alpha\beta} k_\alpha k_\beta h_{\mathbf{k}} \exp(ik_\alpha x^\alpha + \omega t),\end{aligned} \tag{3.65}$$

where $k^2 = k_\alpha k_\alpha = k_1^2 + k_2^2$ and $\pi_0^{\alpha\beta}$ is given by (3.61).

As mentioned before, since the height field does not perturb the in-plane equations for the velocity and the $\lambda$ fields, in what follows we will consider special in-plane flow cases and demonstrate the emergence of the instabilities. The special cases include linear rotational, shear and extensional flows, non-linear squeeze flows and compressible flows. A natural bacterial swarm, of course, consists of all types of flows ranging from simple shear flows to complex squeeze flows. However, all the special linear cases we consider provide analytical formulae for the onset of buckling instability of the monolayer, which not only provide simple physical interpretations but are also amenable to testing from molecular simulations mimicking the bacterial swarm. Furthermore, the velocity gradients in general can be described by a linear combination of fluid flows corresponding to that of shear, rotational, extensional and compressible flows. To see this, in two-dimensions, the velocity gradient is a $2 \times 2$ tensor and the following form a basis for any $2 \times 2$ tensor:

$$\boldsymbol{d}^1 = \begin{pmatrix} 0 & 1 \\ -1 & 0 \end{pmatrix}, \quad \boldsymbol{d}^2 = \begin{pmatrix} 0 & 1 \\ 0 & 0 \end{pmatrix}, \quad \boldsymbol{d}^3 = \begin{pmatrix} 1 & 0 \\ 0 & -1 \end{pmatrix}, \quad \boldsymbol{d}^4 = \begin{pmatrix} 1 & 0 \\ 0 & 1 \end{pmatrix}, \tag{3.66}$$

where $\boldsymbol{d}^1$, $\boldsymbol{d}^2$, $\boldsymbol{d}^3$, and $\boldsymbol{d}^4$ correspond to rotational, shear, extensional and compressible flows and are valid solutions to in-plane equations. As linear flows in (3.66) form a basis set for all fluid behaviors in two dimensions, we perform linear stability analysis for such a set of flows. All of the basis tensors except $\boldsymbol{d}^4$ enforce incompressibility. In what follows, we begin our analysis with those of uniform incompressible flows ($\boldsymbol{d}^1$, $\boldsymbol{d}^2$, and $\boldsymbol{d}^3$), and end with uniform compressible flows ($\boldsymbol{d}^4$).

## *3.1 The case of incompressible rotational flow*

We consider the stability analysis for the case of uniform pure rotational flow ($\boldsymbol{d}^1$) at a resting tension of $\lambda = 0$. In this case, the velocity profile compatible with $\boldsymbol{d}^1$ is given by

$$v^1 = \dot{\gamma} x^2, \qquad v^2 = -\dot{\gamma} x^1; \tag{3.67}$$

see Fig 3.3 for a schematic of the flow. The viscous stresses in a non-Newtonian fluid described by (3.61) for a pure rotational flow are given by

$$\pi_0^{\alpha\beta} = \eta_0(v^{\alpha,\beta} + v^{\beta,\alpha})^n = 0. \tag{3.68}$$

Multiplying (3.65) by $\exp(-ik'_\alpha x^\alpha - \omega t)$ and integrating over all two-dimensional space $(x^1, x^2)$ leads to the dispersion relation

$$\zeta_B\omega(\mathbf{k}) = -\frac{1}{2}k_b k^4 - E_{ad} < 0. \tag{3.69}$$

Since the frequency $\omega < 0$ for all wave-vectors $\mathbf{k}$, none of the modes are unstable which can lead to buckling of the monolayer. Therefore the monolayer is always stable for cases of pure rotational flows.

## *3.2 The case of imcompressible shear flow*

We now consider the case of a uniform shear flow again at zero base tension, where the velocities compatible with $\boldsymbol{d}^2$ are given by

$$v^1 = \dot{\gamma}x^2, \qquad v^2 = 0. \tag{3.70}$$

Corrsponding viscous stresses are

$$\pi_0^{11} = 0, \quad \pi_0^{12} = \eta_0\dot{\gamma}^n, \quad \pi_0^{21} = \eta_0\dot{\gamma}^n, \quad \pi_0^{22} = 0. \tag{3.71}$$

Again multiplying (3.65) by $\exp(-ik'_\alpha x^\alpha - \omega t)$ and integrating over $x^1$ and $x^2$ yields the dispersion relation

$$\zeta_B\omega(\mathbf{k}) = -\frac{1}{2}k_b k^4 - E_{ad} - 2\eta_0\dot{\gamma}^n k_1 k_2. \tag{3.72}$$

Equation (3.72) shows that in the absence of adhesion (i.e., $E_{ad} = 0$), we may have unstable modes in those quadrants of the $k_1, k_2$ plane that satisfy $k_1 k_2 < 0$. In the absence of bending forces ($k_b = 0$), we find that instabilities arise again when $k_1 k_2 < 0$ and the limits of stability ($\omega > 0$) are governed by the condition:

$$k_1 k_2 = -\frac{E_{ad}}{2\eta_0\dot{\gamma}^n}. \tag{3.73}$$

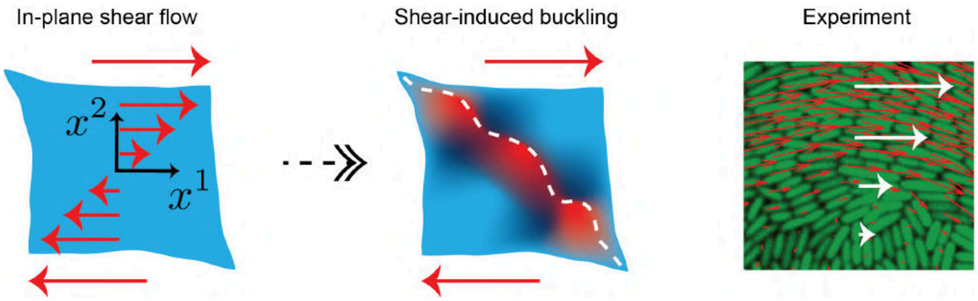


**Figure 3.4:** A schematic representation of the simple shear flow field and the deformation field in the bacterial monolayer. Also shown is the presence of shear flows in bacterial colonies.

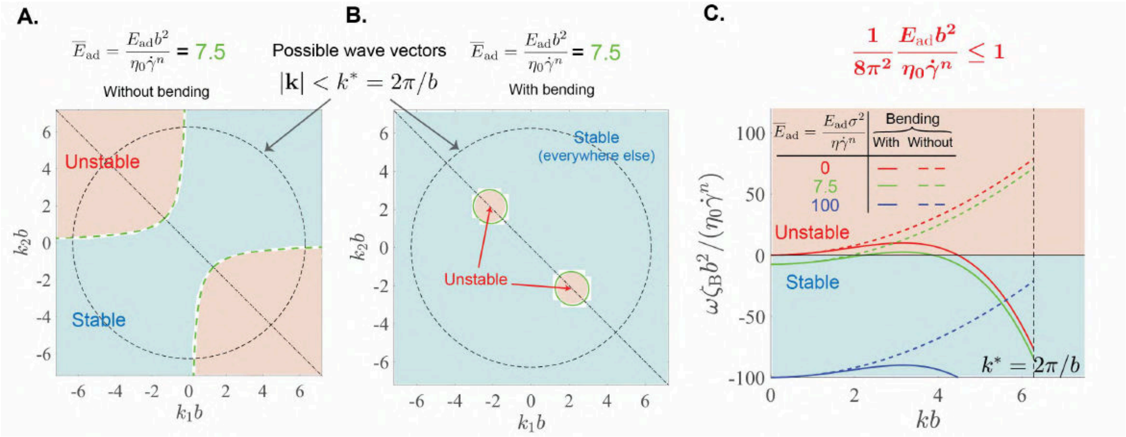


**Figure 3.5:** Stability analysis for a simple shear flow. Left: Stability diagram in the full $k_1 - k_2$ plane with the onset of instability demarcated by a dashed green line, for the case without bending and a fixed non-dimensional adhesion $\overline{E}_{\rm ad} = 7.5$. The dashed black circle indicates the maximum possible wave vector in our system, $k^* = 2\pi/b$, where $b$ is the bacterial length. Center: Stability diagram in the full $k_1 - k_2$ plane with the onset of instability demarcated by a dashed green line, for the case with bending and a fixed non-dimensional adhesion $\overline{E}_{\rm ad} = 7.5$. Right: Stability diagram showing the growth rate of unstable modes as a function of wave vector along the compressional axis, $k_1 = -k_2 = k$, for various cell-substrate adhesion $E_{\rm ad}$ and shearing rates $\dot{\gamma}$, in the presence (solid curves) and absence (dashed curves) of bending. Here, $\omega(k) > 0$ indicate unstable regions. We anticipate that bending plays a negligible role compared to cell-substrate adhesion for bacterial colonies. In the absence of bending, the dispersion relation increases monotonically with $k$, and $\omega(k)$ is maximum at the largest wave vector, $k^* = 2\pi/b$, where $b$ is the bacterial length. This indicates that buckling events from in-plane shearing flows occur at the level of individual bacteria.

Therefore, the relevant length scale at which instability begins to occur, in the presence of adhesion and no bending, is given by

$$\ell \sim \sqrt{\frac{1}{k_1 k_2}} \sim \sqrt{\frac{2\eta_0\dot{\gamma}^n}{E_{\rm ad}}}. \tag{3.74}$$

As adhesion increases, the length scale decreases, indicating that the system is more stable against low frequency perturbations. As adhesion decreases, the length scale increases and the system is unstable against all modes including small wave vectors.

Figure 3.5 shows the dispersion curves for various values of adhesion and bending modulus. When adhesion strength $\overline{E}_{\rm ad} = \frac{E_{\rm ad}b^2}{\eta_0\dot{\gamma}^n}$ is high with $b$ the average bacterial length, there exist no positive values of $\omega$ for all wave vectors, which can lead to the growth of an instability with and without bending. However, for zero to low enough adhesion strength, there exist non-zero growth modes leading to buckling. In the absence of bending, the growth rate is $\zeta_{\rm B}\omega = -2\eta_0\dot{\gamma}^n k_1 k_2 - E_{\rm ad}$, which increases monotonically with the wave vector. Therefore, the fastest growing mode is the largest possible wave-vector, or wave-lengths corresponding to the size of individual bacteria. Such a wave-vector in a bacterial colony corresponds to the length scale $b$ of an individual cell, $k^* = 2\pi/b \approx 2\pi/(0.5\mu m)$, for bacterial colonies of *P. aeruginosa*. The critical boundary of instability can be obtained by setting $k_1^* = -k_2^* = 2\pi/b$ in (3.73) leading to

$$k_1^* k_2^* = \frac{E_{\rm ad}}{2\eta_0\dot{\gamma}^n} \approx \left(\frac{2\pi}{b}\right)^2. \tag{3.75}$$

Therefore, we expect the boundary of instability to lie along a linear ratio of adhesion to shear rate, *i.e.*,

$$\frac{1}{8\pi^2}\frac{E_{\rm ad}b^2}{\eta_0\dot{\gamma}^n} \leq 1. \tag{3.76}$$

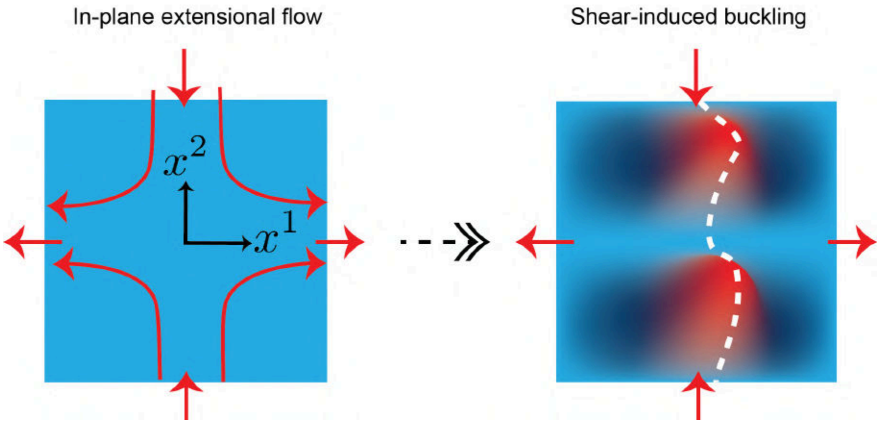


**Figure 3.6:** A schematic representation of the extensional flow field and the deformation field in the monolayer.

## 3.3 The case of extensional flow

We now consider the case of a uniform extensional flow ($\boldsymbol{d}^3$ in (3.66)) with corresponding velocity components given by

$$v^1 = \dot{\gamma}x^1, \qquad v^2 = -\dot{\gamma}x^2; \tag{3.77}$$

see Fig 3.6 for a schematic of extensional flow. In this case, the fluid is drawn along the $x^2$-axis and is pushed out along the $x^1$-axis. We again consider the base tension $\lambda_0 = 0$. The viscous stresses are

$$\pi_0^{11} = \eta_0\dot{\gamma}^n, \quad \pi_0^{12} = 0, \quad \pi_0^{21} = 0, \quad \pi_0^{22} = -\eta_0\dot{\gamma}^n. \tag{3.78}$$

The dispersion relation for the extensional flow can be obtained as

$$\zeta_{\mathrm{B}}\omega(\mathbf{k}) = -\frac{1}{2}k_{\mathrm{b}}k^4 - E_{\mathrm{ad}} - \eta_0\dot{\gamma}^n(k_1^2 - k_2^2). \tag{3.79}$$

Equations (3.79) and (3.72) can be transformed into one another by a change of variables with $k_1$ and $k_2$ in (3.72) being replaced by $\frac{1}{\sqrt{2}}(k_1+k_2)$ and $\frac{1}{\sqrt{2}}(k_1-k_2)$, respectively. Therefore, dispersion curves for extensional flow can be obtained by a simple transformation of those corresponding to shear shown in Fig. 3.5. Experimentally, extensional flows can be realized when different motile flocks of bacteria collide into each other and disperse outward, and we would anticipate membrane instabilities along the compressional axis if the shear rate is large enough. An extreme version of the extensional flow in a narrow width leads to the case of squeeze flow, which will be considered in the following section.

## 3.4 The case of nonlinear incompressible squeeze flows

Until now, we considered only special cases involving linear flows where the velocity gradients are uniform in space. We have also neglected the effects of in-plane tension on the stability of the monolayer. In what follows we consider the case of nonlinear flows, and in particular squeeze flows. The squeeze flows arise when two motile flocks of bacteria of length scale $L$, collide with each other but can only disperse outward from a narrow constriction with a characteristic size $2\delta \ll L$ (see

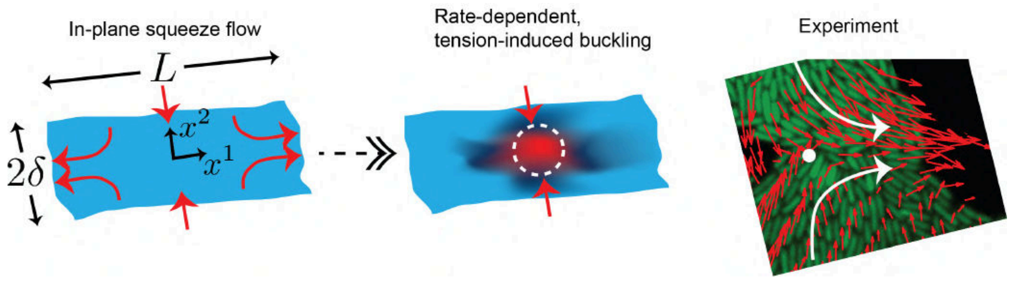


**Figure 3.7:** A schematic representation of squeeze flow and the deformation field in the bacterial monolayer. Also shown on the right is a plausible scenario of a squeeze flow in bacterial colonies.

Fig. 3.7). Such a situation may occur not only in the bulk of swarming bacterial colonies but also at T-junctions as shown in Fig. 3.8. This case also shows an instance in which motility-induced tension plays a dominant role in leading to an instability of the monolayer. The viscous stresses for a Newtonian fluid is given by choosing the exponent $n = 1$ in (3.59), with $\eta_0$ now being the shear viscosity.

The instabilities arising from squeeze flows can be analyzed using the theories of lubrication [84] by realizing that the gap ratio $\epsilon = \delta/L \ll 1$. Here, we consider our in-plane fluid equations and the viscous behaviors to be that of a Newtonian fluid, instead of the power-law behavior considered for linear flows in the previous sections. We note that such a simplification is amenable to realizing again analytical solutions for the velocity profiles and tension in lubricating flows, in contrast to those of a non-Newtonian fluid which leads to partial differential equations that are unnecessarily cumbersome to solve for. Moreover, as we will see, this specialization to Newtonian fluids is sufficient to understand the role of non-linear and spatially inhomogeneous flows leading to instabilities arising specifically from motility-induced tension gradients.

To begin the lubrication analysis, suppose that we have a fluid monolayer inside a narrow gap of width $2\delta$ and length $L$ as shown in Fig. 3.7. Let us consider the velocity of the fluid at the top and the bottom of a gap to satisfy

$$v^1(x^1, x^2 = \delta) = 0, \quad v^2(x^1, x^2 = \delta) = -U, \tag{3.80}$$
$$v^1(x^1, x^2 = -\delta) = 0, \quad v^2(x^1, x^2 = -\delta) = U, \tag{3.81}$$

corresponding to a situation of two opposing flocks of bacteria arriving at velocity $U$ in the thin gap $2\delta$. In the lubrication approximation, the following non-dimensional quantities are useful to

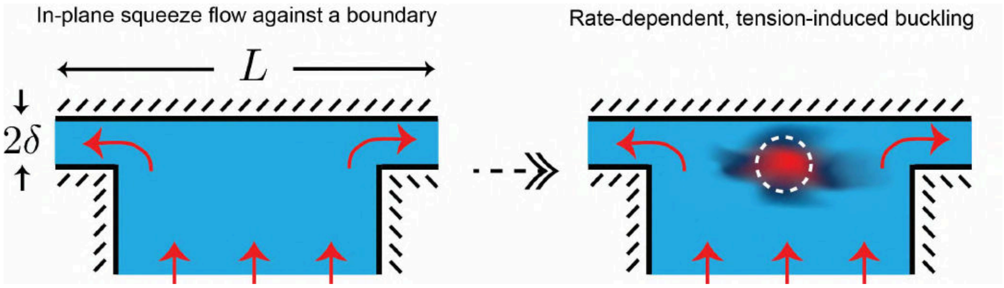


**Figure 3.8:** A schematic representation of squeeze flow against a boundary and the deformation field in the bacterial monolayer.

understand the variations in the relevant field variables:

$$\hat{x}^1 = \frac{x}{L}, \quad \hat{x}^2 = \frac{x^2}{\delta} = \frac{x^2}{\epsilon L}; \quad \hat{v}^2 = \frac{v^2}{U}; \quad \hat{v}^1 = \frac{v^1}{V}; \quad \hat{\lambda} = \frac{\lambda}{\Lambda}. \tag{3.82}$$

Using the dimensionless quantities in (3.82), the in-plane balance equations (3.56) and (3.57) can now be non-dimensionalized.

First, the mass balance yields

$$\left(\frac{V\epsilon}{U}\right)\frac{\partial \hat{v}^1}{\partial \hat{x}^1} + \frac{\partial \hat{v}^2}{\partial \hat{x}^2} = 0, \tag{3.83}$$

which dictates that the characteristic velocity $V$ in the $x^1$-direction should obey $V = \frac{U}{\epsilon}$ for the flow profile to be compatible with the velocity boundary conditions (3.80) and to not violate the mass balance. This then leads to a modified mass balance equation given by

$$\frac{\partial \hat{v}^1}{\partial \hat{x}^1} + \frac{\partial \hat{v}^2}{\partial \hat{x}^2} = 0. \tag{3.84}$$

Next, the non-dimensionalization of the in-plane momentum equation in the $x^1$-direction using (3.82) and $U = V\epsilon$ yields

$$0 = \left(\frac{\Lambda\delta^2}{L\eta_0 V}\right)\frac{\partial \hat{\lambda}}{\partial \hat{x}^1} + \epsilon^2 \frac{\partial^2 \hat{v}^1}{\partial (x^1)^2} + \frac{\partial^2 \hat{v}^1}{\partial (x^2)^2}, \tag{3.85}$$

which indicates that the characteristic in-plane tension $\Lambda$ should scale as

$$\Lambda = \frac{\eta_0 V L}{\delta^2} \tag{3.86}$$

to find a variation in the tension along the $x^1$-direction that balances the viscous stresses. This also indicates that the gradients of $v^1$ in the $x^1$-axis are smaller than the gradients in the $x^2$-direction in the lubrication approximation $\epsilon \ll 1$. With these simplifications, (3.85) reduces to

$$0 = \frac{\partial \hat{\lambda}}{\partial \hat{x}^1} + \frac{\partial^2 \hat{v}^1}{\partial (x^2)^2}. \tag{3.87}$$

Again using $V = \frac{U}{\epsilon}$ and (3.82), non-dimensionalization of (3.57) in the $x^2$-direction leads to

$$0 = \left(\frac{\eta_0 V}{L^2}\right)\left[\frac{\partial \hat{\lambda}}{\partial \hat{x}^2} + \epsilon^4 \frac{\partial^2 \hat{v}^2}{\partial (x^1)^2} + \epsilon^3 \frac{\partial^2 \hat{v}^2}{\partial (x^2)^2}\right], \tag{3.88}$$

and for $\epsilon \ll 1$ reduces to

$$0 = \frac{\partial \hat{\lambda}}{\partial \hat{x}^2}. \tag{3.89}$$

Equation (3.89) indicates that tension $\lambda$ is uniform along the $x^2$ axis, and any gradients in $\lambda$ exist only along the longer $x^1$ direction.

The governing equations for the velocity and tension in the lubrication approximation are given in (3.84), (3.87) and (3.89). These are subjected to no-slip boundary conditions for the velocity in

(3.80) and the tension is assumed to be zero at the two exits of the constriction located at $x^1 = \pm L$. These equations can be solved with standard techniques in lubrication analysis [84] yielding the velocity and tension profiles to be

$$v^1(x^1, x^2, t) = \frac{3}{2}\dot{\gamma}x^1 \left[1 - \left(\frac{x^2}{\delta}\right)^2\right], \tag{3.90}$$

$$v^2(x^1, x^2, t) = -\frac{3}{2}\dot{\gamma}\delta \left[\frac{x^2}{\delta} - \frac{1}{3}\left(\frac{x^2}{\delta}\right)^3\right], \tag{3.91}$$

$$\lambda(x^1, x^2, t) = -\frac{3}{2}\eta_0\dot{\gamma}\left(\frac{L}{\delta}\right)^2 \left[1 - \left(\frac{x^1}{L}\right)^2\right], \tag{3.92}$$

where $\dot{\gamma} = U/\delta$ is a measure of the squeezing strain rate.

As can be seen from (3.90), the velocity profile along the $x^1$-direction is that of a tension-driven parabolic flow. Equation (3.92) indicates that the tension is negative and attains a minimum at the center of the gap. This negative tension is dependent on the rate $\dot{\gamma}$ at which the flow is squeezed through the narrow constriction, and can induce a buckling instability of the monolayer by overcoming the adhesion forces. This possibility is explored below.

Substituting the solutions (3.90)-(3.92) into the out-of-plane equations (3.65) and performing the linear stability analysis as before in the cases of linear flows, we obtain the growth rate for instability for the squeeze flow to be

$$\zeta_{\mathrm{B}}\omega(\mathbf{k}) = \frac{\eta_0\dot{\gamma}}{2}\left[\left(\frac{L}{\delta}\right)^2 (k_1^2 + k_2^2) - (k_1^2 - k_2^2)\right] - \frac{1}{2}k_{\mathrm{b}}k^4 - E_{\mathrm{ad}}. \tag{3.93}$$

The first and the second terms on the right of (3.93) arise from the negative tension and the viscous stresses, and the third and fourth terms are the standard bending and adhesion terms that appear in all of the linear cases studied before. The bending and adhesion terms again act as stabilizing terms, while the tension and viscous terms tend to destabilize the membrane. In the squeeze flow, the negative tension appears to be a stronger de-stabilizing term compared to the viscous stresses, due to the large aspect ratio $(L/\delta)$ of the constriction. Therefore, the stability of the system depends solely on the competition between a destabilizing tension term, and the stabilizing bending and adhesion terms.

Figure 3.9 shows the dispersion curves for squeeze flow. It appears that for all values of adhesion forces $\overline{E}_{\mathrm{ad}}$ considered, there is always an instability with and without bending at high wave-vectors in the case of squeeze flows. This behavior is qualitatively different when compared to that of the pure shear flow (Fig. 3.5) where high values of adhesion ($\overline{E}_{\mathrm{ad}}$=100) lead to a stable monolayer. Therefore, squeeze flows arising in a narrow gap can overcome adhesion forces easier in comparison to shearing flows. As can be seen in Figure 3.9, the maximum growth rate again increases with the wave vector, indicating that the instability again occurs at the length scale of the size of single bacteria, similar to the case of buckling events in linear flows. In the absence of bending, the characteristic wave vector is one that balances tension and adhesion terms leading to

$$k_1^* = 2\pi/b \sim \left[\frac{2E_{\mathrm{ad}}}{\eta_0\dot{\gamma}}\left(\frac{\delta}{L}\right)^2\right]^{1/2}, \tag{3.94}$$

which leads to the following condition for instability:

$$\frac{1}{2\pi^2}\frac{E_{\mathrm{ad}}}{\eta_0\dot{\gamma}}\left(\frac{\delta}{L}\right)^2 \leq 1. \tag{3.95}$$

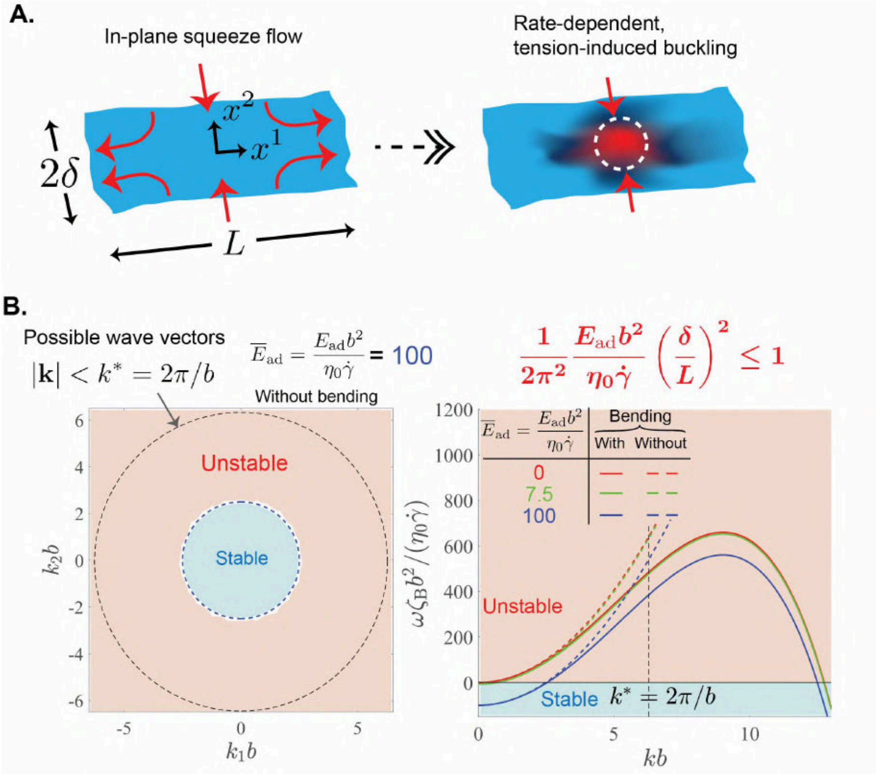


**Figure 3.9:** (A) Schematic of in-plane incompressible squeeze flow arising from flocks of bacteria of length $L$ moving towards each other but can only disperese over a length scale $\delta \ll L$. The red region indicates a stagnation point, leading to a build up of compression, which leads to buckling by tension-curvature coupling term $\lambda \nabla^2 h$ in the momentum balance. (B) Left: Stability diagram in the $k_1 - k_2$ plane with the onset of instability demarcated by a dashed blue line, for the case without bending and a fixed non-dimensional adhesion. $\overline{E}_{\rm ad} = 100$. Right: Stability diagram for the case of squeeze flow, which leads to a maximum growth rate $\omega$ at $k^* = 2\pi/b$ in the absence of bending, thus leading to buckling again at the level of individual bacteria.

In summary, comparing (3.95) and (3.76) indicates that due to the aspect ratio $\delta/L \ll 1$ buckling instabilities may occur even at larger adhesive forces for squeeze flows when compared to the case of shear or extensional flow induced instabilities.

## *3.5 The cases of compressible linear flows*

Previously, we analyzed only incompressible flows, where shearing and non-uniform pressure forces lead to buckling instabilities. In this section, we describe instabilities resulting from compressible linear flows. Here again, we assume the fluid's constitutive behavior to be Newtonian, instead of a non-Newtonian power-law fluid. Such a choice again allows for simple analytical solutions demonstrating the non-trivial role of compressible flows and bulk viscosity. In this case, the relation between the viscous stresses and in-plane velocity gradients is given by (3.32). Following the derivations in Section 2.4 in the Monge representation for small deformations of the monolayer, the viscous stresses reduce to

$$\pi^{\alpha\beta} = \eta_0 (v^{\alpha,\beta} + v^{\beta,\alpha}) + 2\xi v^{\mu}_{,\mu} \delta^{\alpha\beta}, \tag{3.96}$$

where $\xi$ and $\eta_0$ are the bulk and shear viscosities.

Next, the equations of motion for a compressible system in the Monge representation can be

obtained from (3.16), (3.38) and (3.39), which lead to the mass balance

$$\frac{\partial \rho}{\partial t} + \rho_{,\alpha} v^{\alpha} + \rho\big(v^{\alpha}_{,\alpha}\big) = 0, \tag{3.97}$$

the in-plane equations of motion

$$\lambda^{,\alpha} + (2\xi + \eta_0) v^{\mu,\mu\alpha} + \eta_0 \Delta v^{\alpha} = 0, \tag{3.98}$$

and the out-of-plane equation

$$[\lambda + (2\xi + \eta_0)(v^{\alpha,\alpha})]\nabla^2 h + \eta_0 (v^{\alpha,\beta} + v^{\beta,\alpha}) h_{,\alpha\beta} - \frac{1}{2} k_{\mathrm{b}} \nabla^2 \nabla^2 h - E_{\mathrm{ad}} h = \zeta_{\mathrm{B}} \frac{\partial h}{\partial t}, \tag{3.99}$$

where use is made of (3.96). In the case of compressible flow, the tension $\lambda = -\Pi(\rho, Pe)$ is a function of the density $\rho$ and activity $Pe$, with $\Pi$ being the pressure given by the relation (2.30). An increase in density or importantly activity results in an increase in the pressure, thereby reducing tension to significantly negative values, which can then lead to buckling. In what follows, we perform instability analysis for non-zero base tension and its role in buckling instabilities. This is an extension of the previous analysis of in-compressible flows where the base tension was assumed to be zero.

As can be seen from (3.98) and (3.99), the in-plane equations are decoupled from the height fluctuations showing, as in the case of incompressible fluid flows, that the in-plane flows can be solved independent of the shape of the monolayer. This again allows us to consider special cases of compressible flows that satisfy both in-plane equations of motion and demonstrate the buckling instabilities. To analyze the instabilities, let $v^{\alpha}_0$, $\rho_0$ and $\lambda_0$ be the solutions of the mass balance (3.97) and in-plane equations (3.98). Then the out-of-plane equation becomes

$$[\lambda_0 + (2\xi + \eta_0)(v_0^{\alpha,\alpha})]\nabla^2 h + \eta_0 (v_0^{\alpha,\beta} + v_0^{\beta,\alpha}) h_{,\alpha\beta} - \frac{1}{2} k_{\mathrm{b}} \nabla^2 \nabla^2 h - E_{\mathrm{ad}} h = \zeta_{\mathrm{B}} \frac{\partial h}{\partial t}. \tag{3.100}$$

Comparing (3.100) and (3.63), we can see that there exists two additional contributions in the destabilization of the membrane corresponding to the rate of area changes arising from the divergence of the velocity vector and a non-zero base tension/pressure.

In what follows, we demonstrate buckling instabilities by considering special cases of uniform linear compressible flows corresponding to a velocity gradient of the type

$$\boldsymbol{d} = \begin{pmatrix} \nu_1 & 0 \\ 0 & \nu_2 \end{pmatrix}, \tag{3.101}$$

where $\nu_1$ and $\nu_2$ are constant values. Note that $\nu_1$ and $\nu_2$ are also the eigenvalues of the velocity gradient and correspond to compression or extension when $\nu_1 + \nu_2 \neq 0$. The choice of velocity gradient in (3.101) is a solution of the in-plane equations of motion along with a spatially uniform density and tension. This can be seen by substituting (3.101) into (3.97) and (3.98) leading to

$$\frac{\partial \rho_0}{\partial t} + \rho_0(\nu_1 + \nu_2) = 0, \tag{3.102}$$

and

$$\lambda_0^{;\alpha} = 0, \tag{3.103}$$

assuming a spatially uniform density distribution. Equation (3.103) dictates that tension must be uniform in space, and (3.102) indicates density grows exponentially with time whenever $\nu_1 + \nu_2 < 0$. The growth in density leads to an increase in the pressure or a reduction in the tension $\lambda_0 =$

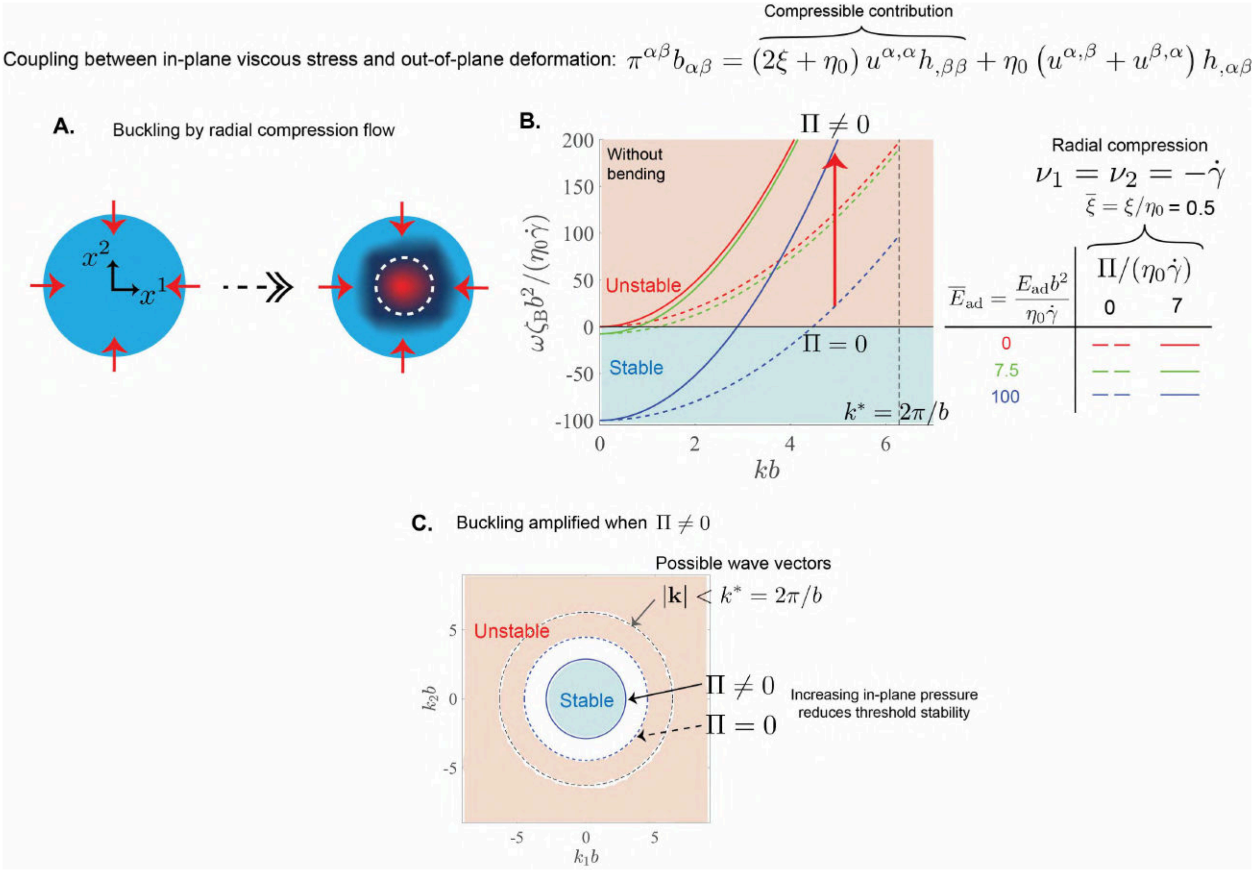


**Figure 3.10:** Left: A schematic of inward (compressible) radial flow arising from flocks of bacteria moving towards a single point. Right: Dispersion curves for compressible squeeze flow showing growth rate as a function of wave vector along the compressional axis of flow (with no bending). Stability diagram for a range of cell-substrate adhesion and different base pressures. Non-zero bulk modulus generates a larger growth rate of unstable modes, and fluid compressibility generally has a destabilizing effect. Bottom: Stability diagram in the $k_1 - k_2$ plane with the onset of instability demarcated by the dashed lines, for the case of $\xi/\eta_0 = 0.5$. The dashed black circle indicates the maximum possible wave vector, $k^* = 2\pi/b$, where $b$ is the bacterial length.

$-\Pi(\rho_0, Pe)$ for a given activity. Furthermore, the velocity gradient in (3.101) encompasses all of the uniform linear incompressible flows $\boldsymbol{d}^1$, $\boldsymbol{d}^2$ and $\boldsymbol{d}^3$ in (3.66) as special cases (by considering the eigenvalues $\nu_1 = -\nu_2 = \dot{\gamma}$, where $\dot{\gamma}$ is arbitrary).

For the choice of velocity gradient in (3.101), the linear stability analysis can again be performed by considering the height fluctuations in terms of normal modes (3.64), which leads to the dispersion relation

$$\zeta_B \omega(\mathbf{k}) = -\frac{1}{2} k_b k^4 - E_{ad} - \Big[ -\Pi(\rho_0, Pe) + (2\xi + 2\eta_0)\nu_1 + (2\xi + \eta_0)\nu_2 \Big] k_1^2 - \Big[ -\Pi(\rho_0, Pe) + (2\xi + \eta_0)\nu_1 + (2\xi + 2\eta_0)\nu_2 \Big] k_2^2, \tag{3.104}$$

expressed in terms of pressure $\Pi$ and the eigenvalues $\nu_1$ and $\nu_2$. In the absence of bending it can be seen from (3.104) that positive growth rates can occur whenever

$$-\Pi(\rho_0, Pe) + (2\xi + 2\eta_0)\nu_1 + (2\xi + \eta_0)\nu_2 < 0, \tag{3.105}$$

or

$$-\Pi(\rho_0, Pe) + (2\xi + \eta_0)\nu_1 + (2\xi + 2\eta_0)\nu_2 < 0. \tag{3.106}$$

Equations (3.105) and (3.106) demonstrate the minimum conditions for $\nu_1$ and $\nu_2$ for plausible buckling. In what follows we consider two special cases corresponding to radially symmetric compression and extensile flows, and discuss the dispersion curves and the buckling instability mechanisms.

### The case of $\nu_1 = \nu_2 = -\dot{\gamma}$ ($\dot{\gamma} > 0$) corresponding to radial compression

Figure 3.10 shows a schematic of buckling induced from radial compressible flow. In this case, the dispersion relation (3.104) in the absence of bending reduces to

$$\zeta_{\mathrm{B}}\omega(\mathbf{k}) = -E_{\mathrm{ad}} + \Big[\Pi(\rho_0, Pe) + (4\xi + 3\eta_0)\dot{\gamma}\Big](k_1^2 + k_2^2). \tag{3.107}$$

Figure 3.10B shows the dispersion curves corresponding to (3.107) for different base pressures and adhesion strengths for $\bar{\xi} = \xi/\eta_0 = 0.5$. These curves show that the growth rate increases monotonically as a function of the wave-vector, indicating that buckling again occurs at the maximum wave-vector in the system corresponding to the length scale of the individual bacteria. Furthermore, increasing the base pressure $\Pi$ amplifies the buckling instability and allows the monolayer to buckle at higher adhesion strengths. Figure 3.10C shows the stability diagram in the $k_1 - k_2$ plane indicating all possible wave-vectors leading to buckling instability, and that buckling occurs isotropically in space. Since the maximum growth rate corresponds to the case of $k_1^2 + k_2^2 = (2\pi/b)^2)$ as indicated from the stability diagrams in Fig. 3.10(B) and (C), we can find the adhesion strength below which buckling leads to growth in the third dimension from the condition $\zeta_B\omega(2\pi/b) \geq 0$ yielding

$$\frac{E_{\mathrm{ad}} b^2}{4\pi^2} \leq \Big[\Pi(\rho_0, Pe) + (4\xi + 3\eta_0)\dot{\gamma}\Big]. \tag{3.108}$$

### The case of $\nu_1 = \nu_2 = \dot{\gamma}$ ( $\dot{\gamma} > 0$) corresponding to radial extensile flow

We now consider a special case of buckling under radial extensile flow. Such a scenario is typically counterintuitive as extensile flow tends to stabilize a flock. In this case, the dispersion relation (3.104) in the absence of bending reduces to

$$\zeta_{\mathrm{B}}\omega(\mathbf{k}) = -E_{\mathrm{ad}} + \Big[\Pi(\rho_0, Pe) - (4\xi + 3\eta_0)\dot{\gamma}\Big](k_1^2 + k_2^2). \tag{3.109}$$

The minimal condition for buckling can be obtained (3.109) as

$$\Pi(\rho_0, Pe) > (4\xi + 3\eta_0)\dot{\gamma}. \tag{3.110}$$

Figure 3.11B shows the dispersion curves for different base pressures and adhesion strengths, which show that for negligible base pressures, extensile flows stabilize the monolayer from buckling. However, when $\Pi$ increases, which is typically the case for active systems or colonies at high activity $Pe$ (Fig 2.18), there exist positive growth rates that lead to buckling. Here as well, the growth rates increase monotonically with the wave-vector indicating that buckling occurs at the length scale of the individual bacteria. Figure 3.11C shows the stability diagram in the $k_1 - k_2$ diagram demonstrating that buckling occurs isotropically as expected for symmetric extensile flows. In this case, the condition for which buckling occurs can be obtained by substituting $k^2 = k_1^2 + k_2^2 = (2\pi/b)^2$ and considering a positive growth rate evaluated at the bacterial length scale yielding

$$\frac{E_{\mathrm{ad}} b^2}{4\pi^2} \leq \Big[\Pi(\rho_0, Pe) - (4\xi + 3\eta_0)\dot{\gamma}\Big]. \tag{3.111}$$

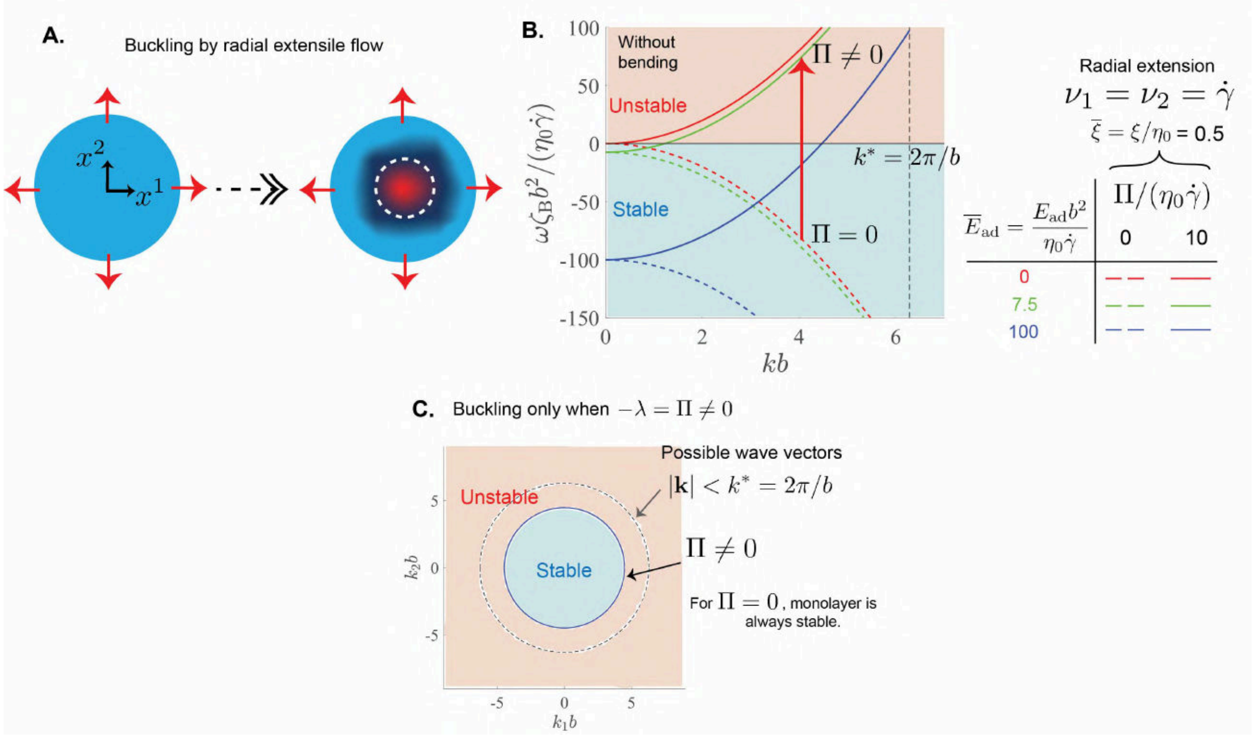


**Figure 3.11:** Left: A schematic of outward radial flow arising from flocks of bacteria moving away from a single point. Right: Dispersion curves for extensile flow showing growth rate as a function of wave vector along the radial direction. Bottom: Stability diagram in the $k_1 - k_2$ plane with the onset of instability demarcated by the dashed lines, for the case of $\xi/\eta_0 = 0.5$. The dashed black circle indicates the maximum possible wave vector, $k^* = 2\pi/b$, where $b$ is the bacterial length.

For a given adhesion strength and a base pressure, one may also alternatively obtain the maximum extensile rate below which buckling occurs as

$$\dot{\gamma}_{\max} = \frac{\Pi(\rho_0, Pe) - \frac{E_{\text{ad}}b^2}{4\pi^2}}{(4\xi + 3\eta_0)}. \tag{3.112}$$

This concludes our analysis of flow or motility induced buckling mechanisms leading to out-of-plane growth.

# 4. Molecular simulations to test buckling mechanisms of colonies

In what follows, we test the buckling mechanisms using molecular simulations of 2D polydisperse spherocylinder systems described in Chapter II. Acknowledging the existence of various types of in-plane flow induced buckling mechanisms, molecular simulations are best suited for testing the case of uniform in-plane shear-flow induced buckling (Sec. 3.2), since shearing can be implemented using well known Lees-Edwards boundary conditions [85], which are compatible with periodic boundary conditions. Further, shearing simulations also lead to an accurate description of the constitutive behaviors (power-law fluid), which can be used to test the scaling relation (3.76) obtained in Sec. 3.2.

## 4.1 Constitutive behavior of 2D polydisperse spherocylinder systems

We begin by obtaining the constitutive stress-strain rate behavior of fully-2D polydisperse spherocylinder systems with polydispersity as that of the *P. aeruginosa* bacterial colonies, where particles are not allowed to move out-of-plane. To that end, we apply an in-plane simple shear flow $\mathbf{v} = \dot{\gamma} x^2 \mathbf{e}_1$ by resizing the simulation box containing spherocylinders with Lees-Edwards boundary conditions [85] for various shearing rates $\dot{\gamma}$. The stress tensor is calculated with the Irving-Kirkwood formula (2.26), which then yields the shear viscosity given by

$$\eta^{\text{eff}} = \sigma_{12}/\dot{\gamma}. \tag{3.113}$$

The shear viscosity as a function of $\dot{\gamma}$ across three different densities is shown in Fig. 3.12. We observe that the dense spheroyclinders behave as a shear-thinning, power law fluid with an effective viscosity $\eta^{\text{eff}} = \sigma_{12}/\dot{\gamma} \sim \dot{\gamma}^{-0.5}$, consistent with dense colloidal suspensions [56–58]. Note that for large shear strains, the spherocylinders align along the extensional axis of shear and the system stays no longer isotropic. We only use and calculate the shear stress during the isotropic phase at lower strain rates.

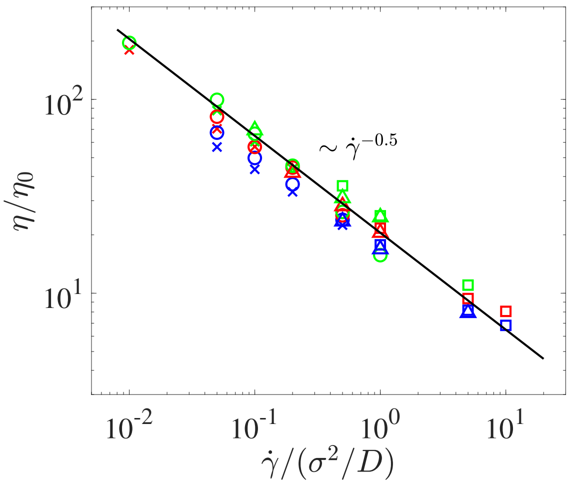


**Figure 3.12:** Shear viscosities for three different fixed area fractions, where green, red, and blue symbols correspond to $\phi = 0.81$, $\phi = 0.78$, and $\phi = 0.76$, respectively. Black line is a fit to obtain shear-rate dependent viscosity. We observe shear-thinning power law behavior with exponent of $-0.5$, similar to the case of hard colloidal systems under negligible hydrodynamic interactions [56–58].

## 4.2 The case of shear flow for passive spherocylinder systems

This power law fluid behavior suggests that the critical onset of shear flow induced instability (3.76) is given by

$$\frac{E_{\text{ad}} b^2}{\eta_0 \dot{\gamma}^{0.5}} = \text{const.} \tag{3.114}$$

Note that equation (3.114) explicitly indicates the nature of power-law fluid in mediating the instability with the presence of an exponent 0.5. Therefore, checking whether the condition (3.114) holds in molecular simulations provides a stringent test of the flow-induced buckling mechanisms.

To test the shear flow induced buckling, we return to our shearing molecular simulations, but now allow the spherocylinder particles to buckle out-of-plane, as shown in Fig. 3.13. The spherocylinder systems also include attractive interactions with the bottom substrate modeled by Morse wall potential [60, 61], which for a range of parameters operates effectively as a Hookean spring potential $U = k(z - r_0)^2/2$ with stiffness $k = 2D_0\alpha^2$. Here, $z$ and $r_0$ indicate the vertical and equilibrium resting length with respect to the substrate, respectively. A narrow potential well is fixed (corresponding to a value of $\alpha = 10^{-4}$ in the HOOMD code corresponding to the Morse wall potential [60, 61]) at a distance of $r_0 = \sigma/2$. The depth of the well $D_0$ is varied in the simulations to modulate adhesion strength between the spherocylinder and the substrate.

Equation (3.114) shows a competition between shear stress and substrate adhesion. We therefore conduct shearing simulations across four different substrate adhesions and three different densities, and check for buckling events of particles from 2D to 3D. The buckling event is defined as the instance when a particle rises 1 particle diameter above the monolayer, consistent with the limit of attractive adhesion interactions with the substrate. Figure 3.13 shows that for a given adhesion strength, monolayers are stable for lower shear rates, while buckling events occur at larger strain rates consistent with the condition (3.76). Furthermore, across all of the simulations where the monolayers are unstable, we observe all of the buckling events occur at the level of individual particles. This is consistent with our theory, which predicts that the fastest growth of deformation occurs at a wave-vector corresponding to the largest wave vector in the system, *i.e.,* smallest length scale in the system—an individual bacterial size. This is further consistent with our experiments on *P. aeruginosa* colonies, which show individual bacteria popping out into the third dimension in a spatially heterogeneous manner, as opposed to rafts of bacteria delaminating from the monolayer.

The results from molecular simulations indicating a stability map for various adhesion strengths and shearing rates across three different densities is shown in Fig. 3.14, where circles and crosses

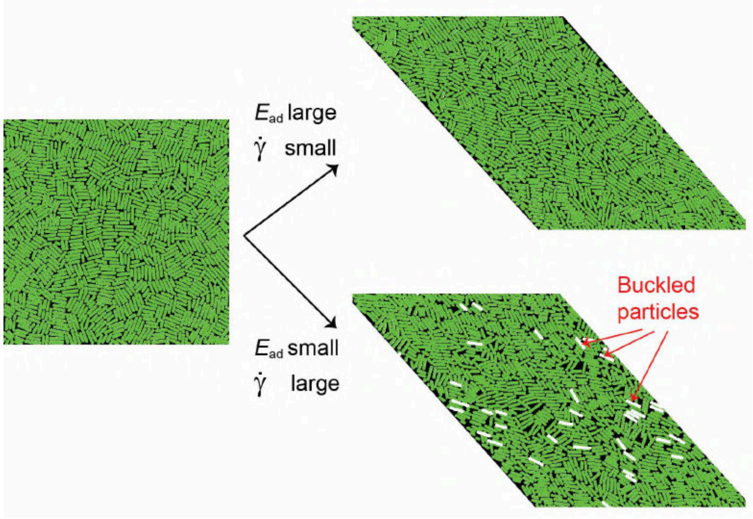


**Figure 3.13:** Shearing molecular simulations containing 2D polydisperse spherocylinders to test the shear flow induced buckling instability criterion. Snapshots of the simulations of polydisperse spherocylinders imposed with homogeneous shear flow. The particles remain stable in the monolayer for large cell-substrate adhesion $E_{ad}$ and small shear rates $\dot{\gamma}$. For small $E_{ad}$ and large $\dot{\gamma}$, we observe particles overcome adhesive interactions with the substrate leading to buckling events out of plane at the level of individual particles. Particles that buckled are shown in white.

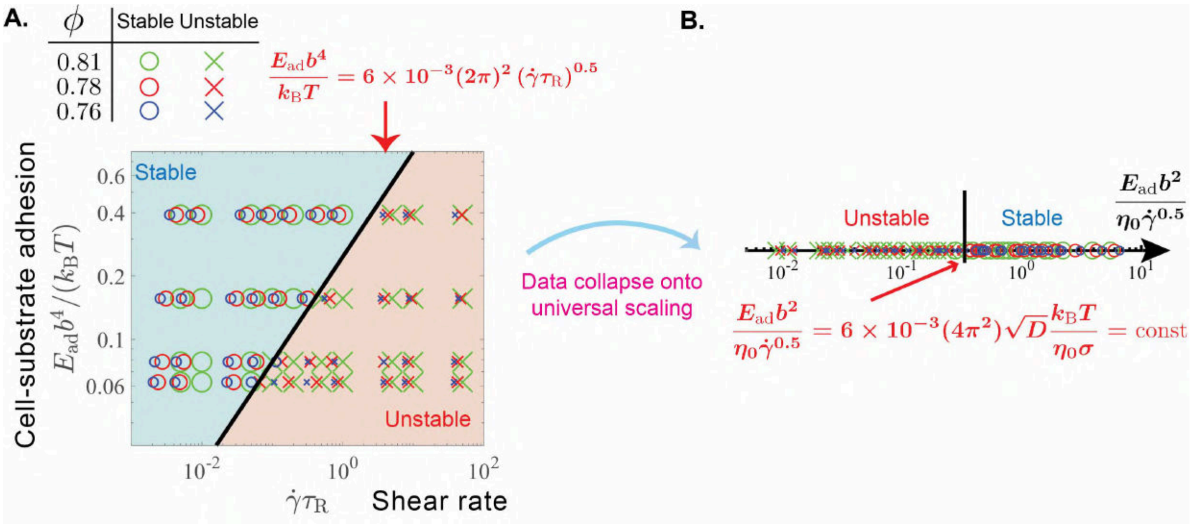


**Figure 3.14:** (A) Results from molecular simulations of monolayers for various various cell-substrate adhesion and imposed homogeneous shear rates. The circles and crosses indicate stable and unstable regions of the monolayers, respectively. The solid black curve indicates the dividing line between stable and unstable regions and is remarkably consistent with the theoretical expression. (B) Collapse of all data onto a single universal scaling relation as predicted by the theory for power-law fluids. This concretely demonstrates that shear stresses $\pi^{\alpha\beta}$ arising from in-plane shearing flows lead to buckling of particles into the third dimension.

indicate stable and unstable systems, respectively.[3] Remarkably, the data show excellent agreement for critical buckling given by the relation $E_{\rm ad} \sim \eta_0 \dot{\gamma}^{0.5}$. Furthermore, Fig. 3.14 also shows that all data collapse to single point when scaled by (3.114), thus confirming the mechanism of shear flow induced buckling instability. Taken together, these simulations and corresponding observations provide evidence for the existence of flow/motility induced buckling instabilities in bacterial colonies leading to growth into the third dimension.

## *4.3 The case of localized shear at an interface for passive spherocylinder systems*

The analytical scaling relations for the instabilities and the molecular simulations in Fig. 3.14 correspond to uniform shear flows. To demonstrate that our proposed buckling mechanisms are applicable even in cases with localized shear flows, we perform molecular simulations corresponding to an increasingly complex case where two adjacent flocks are driven uniformly in opposite directions (see Fig. 3.15A and also SI Movie S12). Figure 3.15A shows a snapshot of the 2D spherocylinder system with particles subjected to equal and opposite body forces in the top and bottom parts of the system, thereby creating an interface with localized shear velocity gradients. The shear flow induced buckling mechanism then dictates that buckling events should occur predominantly at the interface separating the two flocks. Using the same criteria for observing buckling events corresponding to instances where particles displace vertically at least by their diameter, Fig. 3.15B shows the probability of buckling events along the $x^2$-direction. Figure 3.15B indeed shows that almost all of the buckling events are localized to the interfaces, thus consistent with our theory for buckling. These results further support the applicability of our flow-induced instability mechanisms.

[3]Note that the horizontal axis is normalized by a density-dependent shear viscosity $\eta_0(\phi)$ to enable direct comparison of the three area fractions tested.

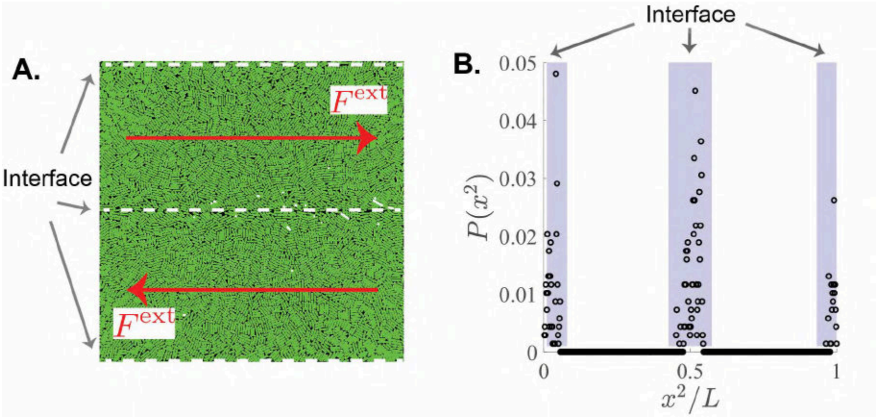


**Figure 3.15:** Monolayers show buckling events in regions of localized shear flows. (A) Snapshot of MD simulations of polydisperse, non-motile spherocylinders with an external body force, where particles on the upper half ($x^2 > 0$) and lower half ($x^2 < 0$) of the simulation box are driven by an equal and opposite body force $F^{\mathrm{ext}}$ and $-F^{\mathrm{ext}}$, respectively, thus creating two interfaces at $x^2 = 0$ and $x^2 = \pm L_{x^2}/2$, where $L_{x^2}$ is the length of the simulation box. (B) Probability of buckling along the $x^2$ direction across the entire duration of the simulation where probabilities have been slab averaged over the $x^1$ dimension. The peaks in the probability distribution (in blue shades) show that buckling occurs at interfaces of localized shear stresses.

# 5. Role of topological defects in buckling

Recent works on motile mammalian tissues [86, 87] have focused on topological defects and their role in "extrusion" or buckling out of a monolayer, by considering the tissue to be an active nematic. For motile bacterial colonies of *P. aeruginosa*, we observe no strong indication of buckling events occurring at sites of defects (see SI Movies S19-S20). There are two large differences between 2D active mammalian tissues and bacterial colonies that may contribute to this observation.

First, bacterial motility speeds ($\sim \mathcal{O}(10\mu\mathrm{m/min})$) are much larger than that of mammalian cells in [86, 87] ($\sim \mathcal{O}(10\mu\mathrm{m/hr})$). As shown in a snapshot in Fig. 3.16A of active spherocylinder simulations, bacterial swarms are highly dynamic with no clear long-range, stable nematic phase or defect formation (see SI Movie S19 for full video). Instead, we observe short, transient lifetime of defects that get disrupted by new configurations in active bacterial swarms, similar to an amorphous liquid that undergoes constant and rapid changes in structure.

Secondly, the aspect ratio of bacterial body is small ($\ell/\sigma \sim 3-4$) with significant polydispersity. At these aspect ratios, equilibrium phase diagrams show that monodisperse spherocylinders exist either in isotropic or smectic phases [88–90]. In contrast, polarized, migrating mammalian cells have strong coupling between the actin cytoskeleton and focal adhesions with the substrate. This has been suggested to provide individual cells anisotropic drag coefficients and make cells difficult to reorient rapidly, which may help produce long-lasting nematic ordering and defects [87]. We observe that adding polydispersity in our MD simulations disrupts the smectic phases and results in a micro-crystalline smectic structure. Furthermore, adding activity to MD simulations yield a flowing polycrystal (i.e., small domains of flocks), and not an active nematic; this behavior is also observed in swarming *P. aeruginosa* colonies. In this case, individual cells and crystals can reorient readily and transient polar flocks are disrupted more easily, thus making defects unimportant in studies of *P. aeruginosa*. We also performed MD simulations of larger aspect ratio ($\ell/\sigma = 10$), as shown in Fig. 3.16B and observe, interstingly, that in these cases stable defects form, and are consistent with defects present in motile microtubules [91] and other biopolymers. It is of interest

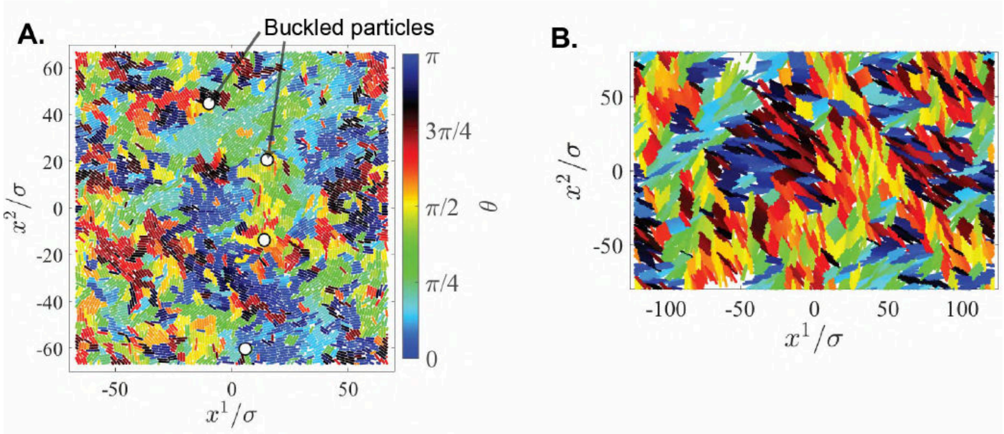


**Figure 3.16:** (A) Instantaneous snapshot of MD simulations of active polydisperse spherocylinders, where the color indicates the orientation of the particle relative to a fixed reference frame. The white circles are the particles that buckled out-of-plane at this time step. We observe microdomains that undergo constant and rapid changes in structure, with no clear long-range nematic order. (B) Instantaneous snapshot of MD simulations of active polydisperse spherocylinders with large aspect ratio, $\ell/\sigma = 10$. Colors again indicate instantaneous orientation of the particle as in (A), where semi-stable defects are observed with these large aspect ratio active particles.

to consider motile bacteria with larger aspect ratios, such as Myxobacteria swarms [92], where the coupling between topological defects arising in active nematics and motility induced in-plane flows may play a significant role in the out-of-plane growth. We leave the analysis of the aspect ratio and its role in bacterial colony growth to future work.

Chapter IV

# CONNECTIONS TO SIMULATIONS AND EXPERIMENTS

Previously, we provided a detailed study of the dynamical state diagram for 2D monolayers at different densities and activities demarcating the boundary between active liquid and glassy states. We also studied various flow/motility induced buckling mechanisms, by considering special cases involving uniform linear and non-linear squeeze flows. We also tested the buckling mechanism for uniform shear flows in molecular simulations, and demonstrated its applicability to an increasingly complex case of flows with localized shear stresses or velocity gradients. However, real bacterial swarms contain a variety of spatially heterogeneous in-plane flow fields, in addition to homogeneous linear flows. We now study the applicability of our motility induced buckling mechanisms in real bacterial swarms.

The inherent activity of the bacteria produces natural swarms, where there exist spatially and temporally-varying shear, tensile and compressive stresses, and corresponding velocity gradients. Therefore, it is not easily possible to isolate different mechanisms by which bacteria buckle out of plane just by visual inspection, requiring a new metric to correlate the flow fields to buckling events. One way to find such a correlation is to calculate the strain-rate tensor at each fluid element, defined by

$$\mathbf{E} = (\nabla \mathbf{v} + (\nabla \mathbf{v})^T)/2, \tag{4.1}$$

where $\mathbf{v}$ is the velocity of the fluid element. The 2D strain-rate tensor contains two eigenvalues $\nu_{\min}$ and $\nu_{\max}$, where negative and positive eigenvalues indicate compression and extension, respectively, in a direction informed by the corresponding eigenvectors. Assuming that buckling is correlated by an appearance of a bacterium onto the second layer[1], one can study the correlation between the eigenvalues and the associated buckling events.

The eigenvalues of the strain-rate tensor corresponding to the buckling events can be represented in a plot as shown in Fig. 4.1, with the smaller value $\nu_{\min}$ on the horizontal axis, and the larger value $\nu_{\max}$ on the vertical axis. This metric for buckling shows points only within the half-space $[\pi/4, 5\pi/4]$, and information about the orientation of the flow (i.e., eigenvectors) is not included. The eigenvalue diagram in Fig. 4.1 can be partitioned into three major distinct zones, each marking a different motility-induced buckling mechanism: (I) Incompressible shear flow ($\nu_{\min}+\nu_{\max} \approx 0$), in pink; (II) Compression and shear flow ($\nu_{\min}+\nu_{\max} < 0$), in green; (III) Extensile flow ($\nu_{\min}+\nu_{\max} > 0$), in blue. All of the buckling mechanisms for incompressible flows considered in Sec. III.3.1-Sec. III.3.4 including uniform shear flows fall under the category of Zone I. Zone II includes all of the flow cases under compression, including radial extension considered in Sec. III.3.5. Finally, Zone III describes scenarios of buckling under extensile flows. It is here that one can clearly identify buckling events under radial extensile flows (Sec. III.3.5), which are allowed only for significant non-vanishing base pressures induced by activity, *i.e.,* $\Pi(Pe) > 0$.

[1]We define buckling as the moment a bacterium's z-position rises 1 cell diameter above the monolayer.

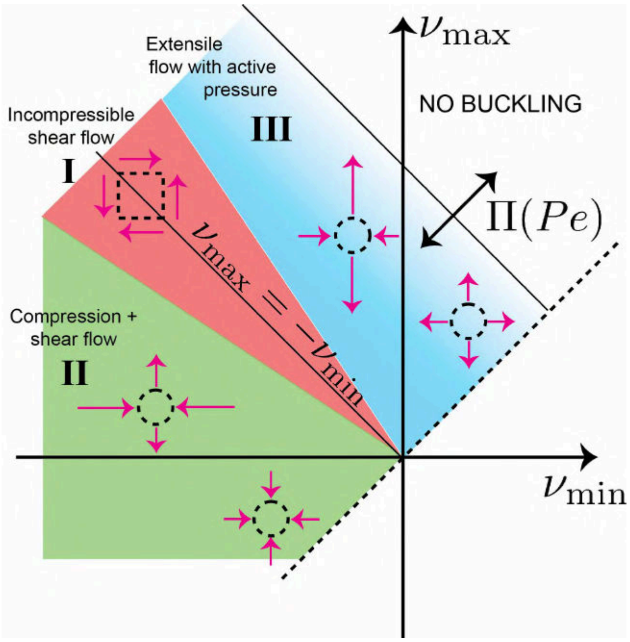


**Figure 4.1:** An eigenvalue-based metric to characterize the flow fields and identify the mechanisms behind buckling events. Eigenvalue portrait shows the different characteristic in-plane flows that can trigger buckling corresponding to distinct zones including incompressible shear flow (zone I), compression and shear flow (zone II), and extensile flows (zone III). Any region where $\nu_{\mathrm{max}} + \nu_{\mathrm{min}} \neq 0$ is a compressible flow.

In what follows, we test the utility of the metric in Fig. 4.1 in molecular simulations of spherocylinder systems, specifically for buckling events corresponding to uniform shear and interfacial flows. We then use it to study the distinct buckling mechanisms in active spherocylinder and *P. aeruginosa* bacterial swarms. Before we begin testing and utilizing the metric, we provide a brief description of how we evaluate the velocity fields at every spatial point in both molecular simulations and the experiments on bacterial colonies.

In MD simulations, we know the precise configurations of all particles at every timestep. Therefore, we bin particles based on their spatial location, and compute a local velocity vector to construct a continuum flow field across the entire colony. The simulation box is divided into square bins of edge lengths $7\sigma$, each containing $N_{\mathrm{b}} \approx 10$ spherocylinders. The instantaneous velocity in each bin is obtained averaged over all particles in the bin

$$\mathbf{v}_{\mathrm{inst}}(x^1, x^2, t) = \frac{1}{N_{\mathrm{b}}} \sum_{i=1}^{N_{\mathrm{b}}} \mathbf{v}_i(x^1, x^2, t), \tag{4.2}$$

where $\mathbf{v}_i(x^1, x^2, t)$ is the velocity of particle $i$ in the bin and $N_{\mathrm{b}}$ is the number of particles in the bin. The velocity in each bin is further coarse-grained in time as

$$\mathbf{v}(x^1, x^2, t) = \frac{1}{\Delta t} \int_{-\Delta t/2}^{\Delta t/2} \mathbf{v}_{\mathrm{inst}}(x^1, x^2, t + t')\ dt', \tag{4.3}$$

where $\Delta t$ is the coarse-graining time (taken to be $\Delta t = \tau_{\mathrm{R}}$). We varied the size of the bin and the coarse-graining time to verify that the velocity fields are insensitive to these chosen values. The rate-of-strain tensor and corresponding eigenvalues are then computed from the flow fields obtained

from (4.3). Out-of-plane transitions are identified whenever a particle's z-position increases more than 1 particle diameter above the monolayer.

For quantification of flow fields and buckling events in experiments on colonies, we obtain time lapse images taken by confocal microscopy on two different z-planes: the bottom (1st) layer at the plane of the bacteria monolayer, and an upper (2nd) layer about 0.5-1 $\mu$m above the monolayer. Buckling is observed directly by an appearance of a bacterium onto the upper imaging plane. We compute the flow field in the monolayer using two methods. In the first method, we obtained displacements of individual bacteria at single-cell resolution by using a particle-tracking algorithm SuperSegger [66]. Cells are binned into elements based on their spatial location, and an average of their velocities then produces a continuum flow field across the entire colony. The size of the square bin was determined such that $\approx 5$ bacteria were contained in each element. In the second method, we obtain average flow fields directly by using an open-source particle image velocimetry (PIV) script, PIVLab [93]. Here, displacements of particle fluorescence intensity is converted into a flow field at each element. Both methods produced quantitatively similar flow fields, and all experimental results presented here and in the main text are obtained by the PIV method.

# 1. Eigenvalue analysis of spherocylinders under uniform & interfacial shear

Let us consider the case of passive spherocylinders subjected to homogeneous shear flow as considered in Sec. III.4.2. In this case, the theory dictates that buckling is dominated by in-plane shearing flows (and therefore shear stresses) generated uniformly across the monolayer (Sec. III.3.2). Since we have uniform shear stress, we expect the eigenvalues of buckling events to correspond to zone (I) in Fig. 4.1, and to lie on the line $\nu_{\min} + \nu_{\max} \approx 0$. As expected, Fig. 4.2 shows perfect agreement with shear flow mediated buckling for a range of external strain rates. Note that the eigenvalues corresponding to buckling events scale in a proportional manner to the magnitude of the imposed strain. Further, Fig. 4.2 shows the population or histogram of buckled particles corresponding to distinct zones, again demonstrating that the buckling events corresponding to incompressible shear flow fall under zone I as expected. Note also that there do not exist any events in Zone I or Zone III in the case of shear flows.

We next test the utility of the metric devised in Fig. 4.1 on describing the buckling mechanisms found in MD simulations of localized shear flows shown in Figs. 3.15. Since there exist uniform shear velocity gradients localized to a boundary layer close to the interface separating the two flocks, the theory predicts that the buckling events should be localized to the interface. Furthermore, corresponding eigenvalues should again correspond to zone (I), and lie on the line $\nu_{\min} + \nu_{\max} \approx 0$. Fig. 4.3 (top) shows perfect agreement with shear flow mediated buckling for a range of external forcing. Figure. 4.3 (Bottom) further shows the population of buckled particles, and indicates that buckling events occur only in Zone I corresponding to incompressible shear flows.

# 2. Eigenvalue analysis of general active colonies

We now apply our metric to both molecular simulations of active spherocylinder swarms, and experiments on *P. aeruginosa* colonies to study the motility-induced buckling mechanisms leading to out-of-plane colony growth. Note that our MD simulations of 2D active spherocylinder systems exhibit swarming flows, consistent with experimental colonies in Fig. 1.2. Therefore, these simulations and corresponding buckling event eigenvalue diagrams are particularly useful in studying the role of activity and density in mediating the motility-induced buckling mechanisms. In particular, we will see that increasing the activity changes the mode of buckling from those mediated by shear

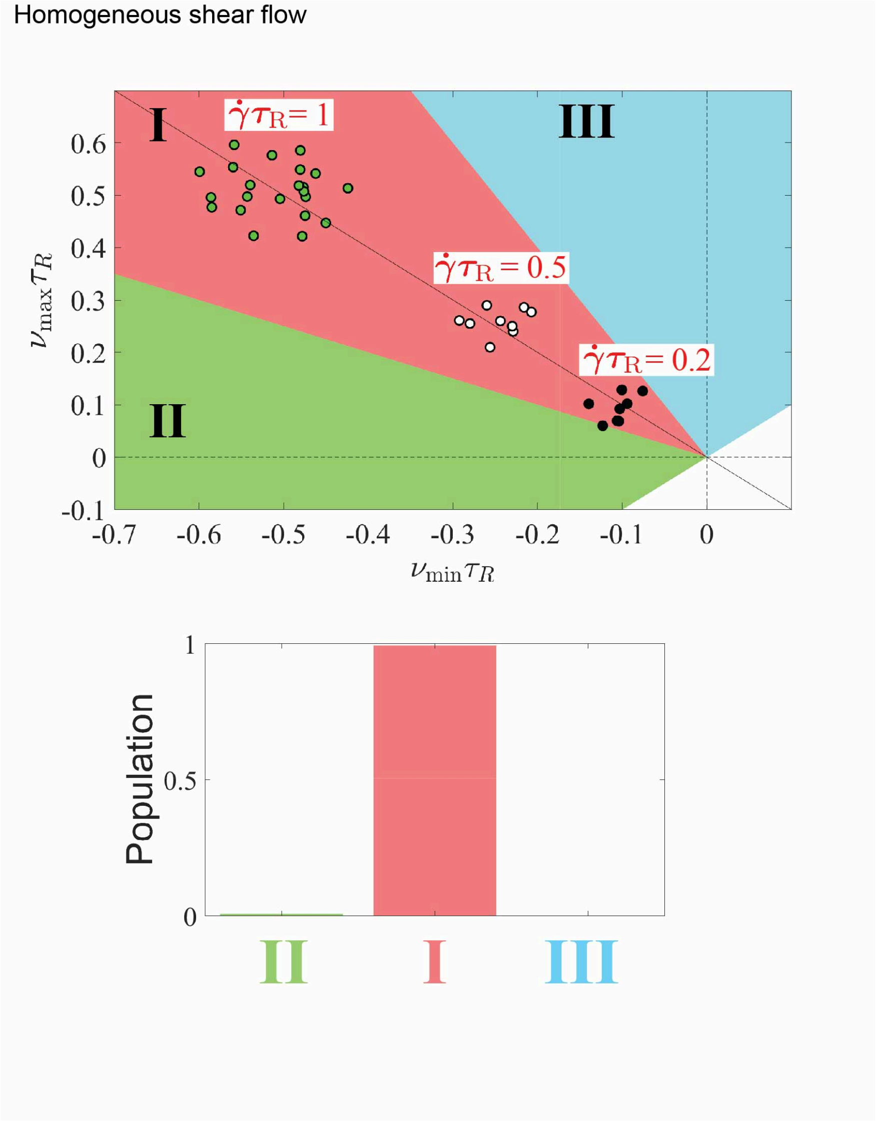


**Figure 4.2:** Eigenvalue scatter plot from MD simulations of simple shear flows in Fig. 3.13 (and Fig. 6A in the main text) for a fixed particle-substrate adhesion and different imposed shear rates, $\dot{\gamma}\tau_R = 1$ (green), 0.5 (white), and 0.2 (black). Bottom: Histogram showing the population distribution of the buckled particles corresponding to the three zones contained in the eigenvalue-portrait above, showing quantitatively that buckling mechanisms correspond entirely to Zone I.

stresses at low activity (zone I) to multiple mechanisms at high activity (all zones). Figures 4.4-4.6 summarize the results of experiments and MD simulations of active (or motile), polydisperse spherocylinders for various activities, for densities lesser than the onset density for glassy dynamics.

Figure 4.4A shows snapshots of molecular simulations, where the red arrows are the velocity field $\mathbf{v}(\mathbf{x})$, the color contour indicates $\nu_{min}$, and the white circular markers indicate cells that buckled at this time step (see SI Movies S14-S16). Smaller activities ($Pe = 5$ in Fig. 4.4A) produce buckling events corresponding to shear flows with rates that are in the vicinity of the unstable region idenfitied in Fig. 3.14. Careful examination of these events further reveals that buckling events occur frequently at interfaces between two opposing flows with localized shear stress, similar

to interface flows studied in Fig. 3.15. In this case, we expect incompressible shear flow mediated buckling corresponding to zone (I), as confirmed in Figs. 4.5 and 4.6. This shows that buckling events at low activity are triggered by a competition of the viscous-curvature coupling term ($\pi^{\alpha\beta} b_{\alpha\beta}$) and cell-substrate adhesion ($E_{\rm ad} h$) consistent with the instability relation in (3.76).

As activity increases, swarming patterns evolve more quickly in time and we obtain nonlinear and/or compressible flows, including squeeze and radial compression/extensile flows. This changes the out-of-plane growth from a simple shear flow induced buckling mechanism (zone I) to that of compression, shear and squeeze flow (zone II). Interestingly, we also observe buckling in extensile flow regions (zone III), which may be counter-intuitive based on a sole competition between adhesion $E_{\rm ad}$ versus viscous-curvature coupling $\pi^{\alpha\beta}$. These results indicate the presence of a nonzero in-plane active pressure $-\lambda = \Pi(Pe, \phi)$ and a significant role of tension-curvature coupling in (3.39), as previously analyzed for radial extensile flows leading to (3.111). In this case, we see that swarming colonies can buckle even in purely extensile regions, if the in-plane pressure is large enough to overcome the stabilizing effects of the extensile flows, as explained in Fig. 3.11. Ultimately, it is the competition between $E_{\rm ad}$ (always stabilizing), $\lambda$ (always destabilizing), and $\pi^{\alpha\beta}$ (either stabilizing

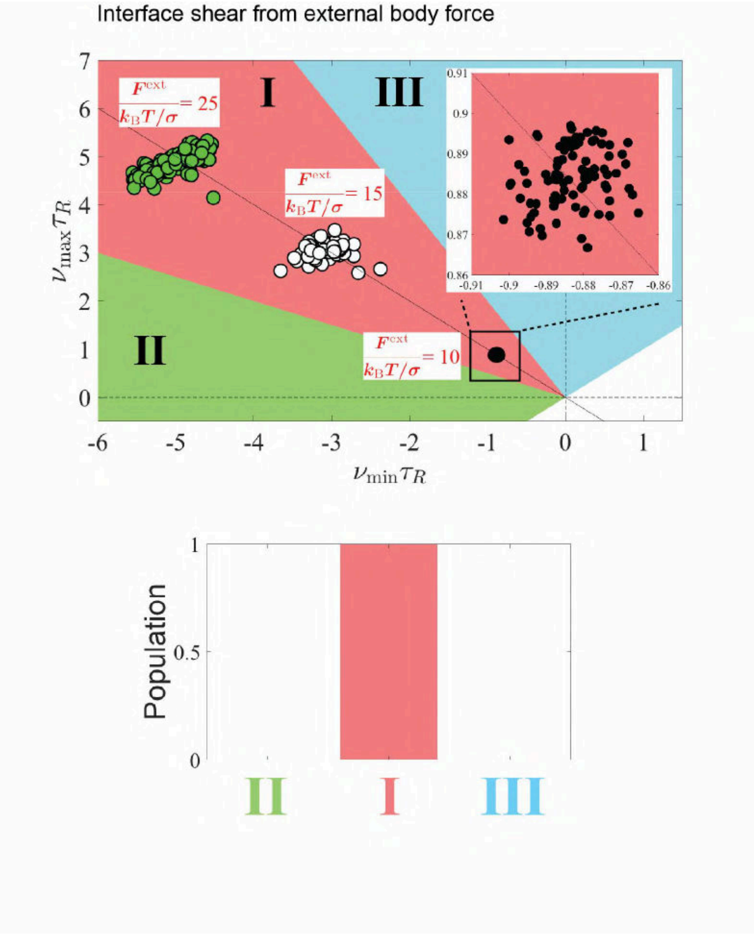


**Figure 4.3:** Eigenvalue scatter plot computed from MD simulations of localized interface shear flows in Fig. 3.15 and Fig. 6C-E in the main text for a fixed particle-substrate adhesion and different external body forces $F^{\rm ext}/(k_{\rm B}T/\sigma) = 25$ (green), 15 (white), and 10 (black). Inset is a magnified view of the data corresponding to the smallest external force. Bottom: Histogram showing the population distribution of the buckled particles corresponding to the three zones.

or destabilizing depending on flow profile). Indeed, eigenvalue plots and histograms for $Pe = 7$ show transitioning of buckling events from zone (I) to zones (II) and (III). For $Pe = 10$, the buckling events further spread uniformly across all zones to shear, squeeze, and radial compressible flows, as shown in Fig. 4.6. Therefore, if motility is strong compared to cell-substrate adhesion, we predict buckling events via a combination of mechanisms involving both viscous-curvature and tension-curvature coupling arising from shear, squeeze, and radial flows.

Figure 4.5B shows the analysis of buckling events in motile *P. aeruginosa* swarms at densities smaller than the onset density for glassy dynamics (see SI Movies S17-S18). Here, we observe the buckling events spread across all zones (see Fig. 4.6), indicating that swarming *P. aeruginosa* colonies exhibit all types of flow characteristics, similar to our simulations at intermediate activity $7 < Pe < 10$. In fact, for the twitching motility speed of $U_0 \sim 10\mu\text{m/min}$, reorientation time of $\tau_\text{R} \sim 1\text{min}$, and characteristic bacteria size of $\sigma \sim 1\mu\text{m}$, the activity of the bacteria corresponds to $Pe = U_0\tau_\text{R}/\sigma \sim 10$. *P. aeruginosa* are known to secrete extracellular polymeric substances that facilitate cell-cell adhesion [94–98]; this may partially stabilize monolayers under extensile flows and help explain the lower population in zone (III) compared to the MD simulations, which do not incorporate cell-cell adhesion. Although cell-substrate and cell-cell adhesion cannot be calculated easily in experiments, an activity of $Pe \approx 7 - 10$ gives results consistent with those of our simulations, where buckling is triggered by all mechanisms.

Taken together, Figs. 4.4-4.6 show that motility-induced buckling mechanisms mediate out-of-plane colony growth. In summary, at densities lower than the onset density, motile bacterial colonies exist in a swarming state and generate motility-induced flows resulting in viscous and compressive stresses. These stresses then induce out-of-plane deformations, subsequently leading to buckling and growth into the third dimension. Finally, at cell densities above the onset density, the colony enters into a kinetically-arrested glassy state that suppresses any in-plane flows, and the nature of buckling crosses over from flow-mediated buckling to a quasi-static growth and division-induced Euler-Bernoulli buckling [1–7]. Our dynamical state diagram in Fig. 2.19C thus provides a fundamental framework to understand and regulate the 3D transition of bacterial colonies.

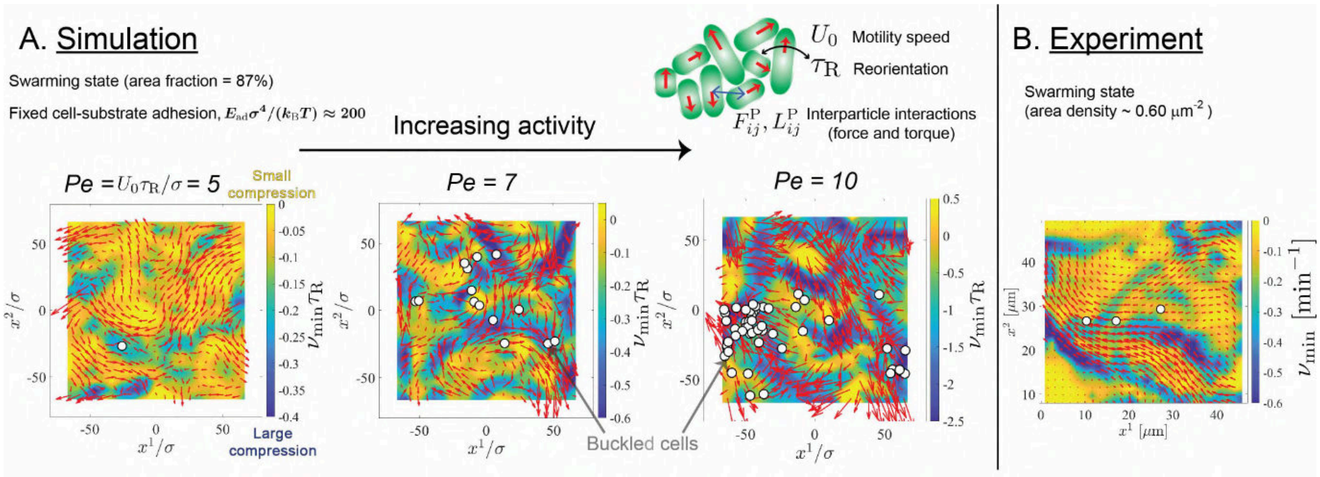


**Figure 4.4:** (A) MD simulations of motile, polydisperse spherocylinders in the swarming state, below the onset pressure for glassy dynamics, across three different activities ($Pe$) for fixed cell-substrate adhesion. Snapshots of the flow fields (red arrows) and $\nu_\text{min}$ (colormap) are shown within a region of the simulation. White circular markers indicate particles that have buckled at this time step. (B) Experiments of bacterial colonies in the swarming state, with a snapshot of flow fields (red arrows) and $\nu_\text{min}$ (colormap) within a region of the colony for cell density of $\sim 0.60\mu\text{m}^{-2}$.

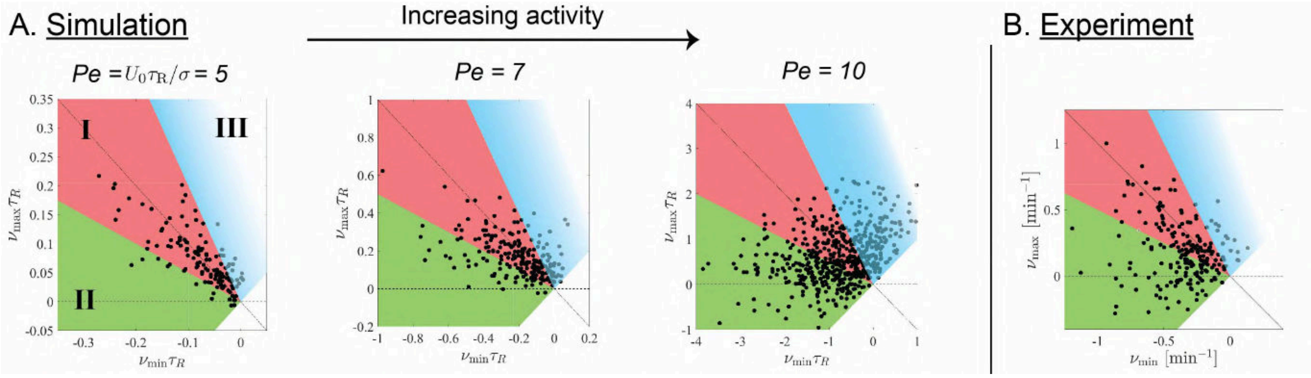


**Figure 4.5:** (A) Eigenvalue scatter plot corresponding to buckling of active spherocylinder simulations. Low $Pe$ shows that majority of buckling events occur by motility-induced incrompressible shear flows. Increasing $Pe$ shows that buckling occurs from a broad variety of mechanisms, including inward and outward incompressible squeeze flows, and radial compressional or extensile flows. Buckling in the blue shaded region (extensile flows with $\nu_{\min} + \nu_{\max} > 0$) indicates that motility-driven in-plane pressure $\Pi$ can generate instability by overcoming stabilizing flows. (B) Experiments of bacterial colonies in the swarming state, with the eigenvalue scatter plot across all cell densities tested in the swarming state (to the left of the glassy onset).

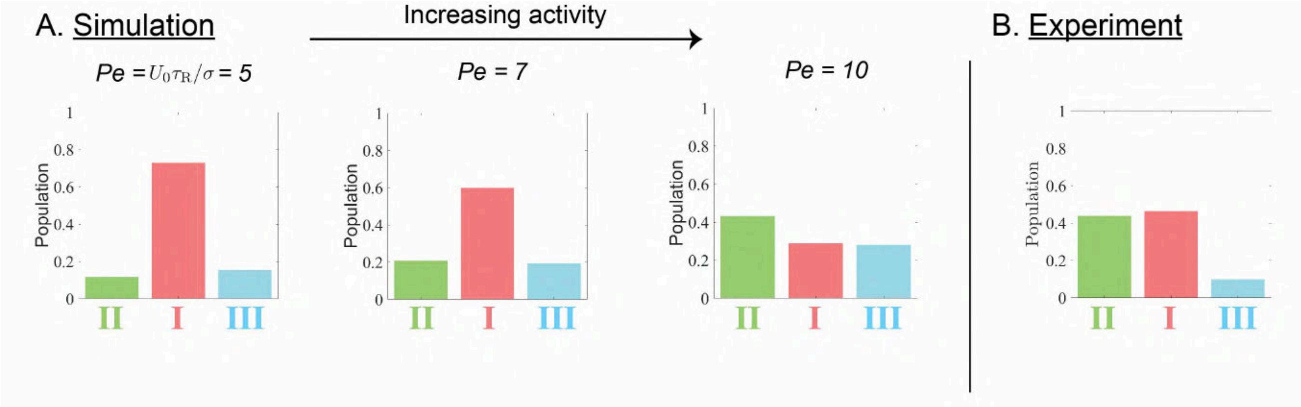


**Figure 4.6:** (A) Histogram of different flow zones that resulted in buckling, color-coded to match the panels in Fig. 4.5, again showing buckling occurs from shear stresses at low $Pe$ to mechanisms mediated by different characteristic in-plane flows at high $Pe$. (B) Experiments of bacterial colonies in the swarming state, with the histogram of buckling events corresponding to the different flow zones. The similarity between experiments and active spherocylinder simulations at $Pe = 10$ show that buckling in swarming *P. aeruginosa* colonies are mediated by a broad variety of flow induced stresses and active pressures.

## 3. Other experimental observations

In addition to 3D transitions, we have also observed a rich diversity of swarming behaviors in *P. aeruginosa* colonies, including patterns at the edges of colonies that resemble fingering instabilities [49, 50] (as shown in Fig. 4.7 and SI Movies S21-S22) . Further, when cells lyse during collective swarming flows, the cell wall ruptures and spills DNA into the surrounding fluid. We observe that these extracellular DNA (eDNA) gets entangled, stretched, and mixed within the motile colony. It has been known that extracellular DNA is critical for biofilm formation [99] and its degradation reduces swarming in *P. aeruginosa* colonies [49]. We experimentally observe that addition of DNA-degrading enzyme DNaseI suppresses swarming and subsequent buckling at leading edges, as shown in Fig. 4.7 and SI Movies S21-S22. By adding SYTOX Nucleic Acid Stain, we observe clear

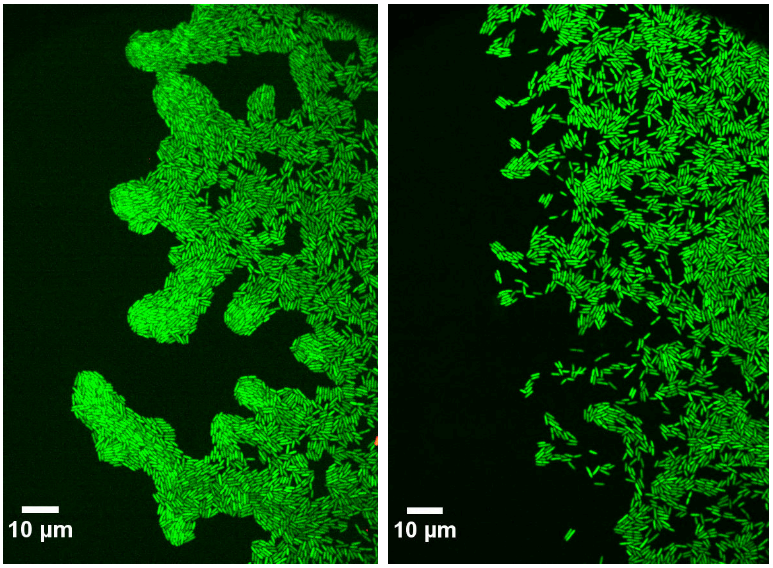


**Figure 4.7:** Confocal image of motile *P. aeruginosa* colonies with (left) and without (right) inclusion of DNaseI. Untreated colonies exhibit collective swarming motion, whereas DNaseI disrupts any collective motion. When a cell dies, the cell wall ruptures and spills DNA into the surrounding fluid. We observe that these extracellular DNA (eDNA) gets entangled, stretched, and mixed within the motile colony. Associated movies are shown in SI videos S21 and S22.

indications of DNA being cleaved in the suspension. Based on our observations, we believe that eDNA promotes collective swarming by increasing the strength of cell-cell adhesion and alignment. Indeed, we have found in our molecular simulations that alignment interactions are needed to generate swarms (e.g., active spherocylinders produce swarms whereas active spherical particles do not).

These observations further support our motility induced buckling mechanism at leading edges; any perturbation that destroys swarming motion prevents rate-dependent buckling. Such effects and other biochemical factors that impact the developmental program of bacterial colony growth require reevaluation of the dynamical state diagram (in Fig. 2.19C), and consequently the motility-induced buckling mechanisms.

## Chapter V

# SUPPLEMENTAL MOVIES

Here we list the Supplemental Movies associated with this manuscript. The movies can be viewed at https://ucsb.box.com/s/fkwe5s8k3qi5096i9dqr0wfyy8rvjx61. In all movies, the time stamp corresponds to hours:minutes:seconds, unless otherwise noted.

**S1.** Fluorescence microscopy timelapse of motile *P. aeruginosa* colony. The colony transitions from a single monolayer of cells at the beginning of the video to a multi-layered structure, which can be observed from the brighter intensity of the colony. The faint black line on the right is an artifact of stitching two image panels together.

**S2.** Fluorescence microscopy timelapse of motile *P. aeruginosa* colony, capturing the instance of buckling due to shear flow. The left and right videos correspond to confocal slices of the bottom and top layers, respectively. We observe a 2D-to-3D transition of bacteria at the site of large shear stress. The time stamp is min:sec.

**S3.** Fluorescence microscopy timelapse of motile *P. aeruginosa* colony, capturing the instance of buckling due to squeeze flow. We observe a 2D-to-3D transition of bacteria at the site of large compressive stresses due to two flocks colliding.

**S4.** Fluorescence microscopy timelapse of non-motile *P. aeruginosa* colony. We observe a 2D-to-3D transition of bacteria only within the deep interiors of large colonies due to quasi-static growth and division. The time stamp is min:sec.

**S5.** Fluorescence microscopy timelapse of non-motile *P. aeruginosa* colony. The colony's leading edge advances very slowly from cellular growth and division. Unlike motile bacteria, we observe a 2D-to-3D transition within the interior of the colony but not at the leading edge.

**S6.** Fluorescence microscopy timelapse of dense motile *P. aeruginosa* colony. The large cell density prevents any collective swarming within the colony. Similar to non-motile colonies, we observe buckling of individual bacteria within the interior of colonies due to division and growth.

**S7.** Fluorescence microscopy timelapse of dense motile *P. aeruginosa* colony exhibiting dynamic heterogeneity. Activated dynamics are apparent by observing the motion of individual bacteria. The large cell density prevents any collective swarming within the colony. Scale bar is $10\mu$m.

**S8.** Displacements of individual bacteria were tracked from a timelapse confocal images of dense motile *P. aeruginosa* colony. Colors indicate displacement magnitude of each bacterium from its initial position, where blue indicates zero displacement and red indicates displacement more than a body length, $2\mu$m. Activated dynamics are apparent by observing the motion of individual bacteria.

**S9.** MD simulations of a monolayer of active, bidisperse spheres in the glassy regime. Displacements of individual particles were tracked. Red and blue colors indicate large and small

displacements of a particle from its initial position. Activated dynamics are apparent by the heterogeneous relaxation of the material.

**S10.** MD simulations of a monolayer of passive, polydisperse spherocylinders subjected to homogeneous shear flow with shear rate, $\dot{\gamma}\tau_{\mathrm{R}} = 0.01$. At small shear rates, we observe no buckling of particles out of plane.

**S11.** MD simulations of a monolayer of passive, polydisperse spherocylinders subjected to homogeneous shear flow with shear rate, $\dot{\gamma}\tau_{\mathrm{R}} = 1$. At large shear rates, we observe buckling of individual particles out of plane (shown in red).

**S12.** MD simulations of a monolayer of passive, polydisperse spherocylinders subjected to opposing 1D body forces along the $\pm x^1$ directions. There is a shear stress generated at the interfaces, located at $x^2 = 0$ and $x^2 = \pm L/2$ where $L$ is the box size. Red particles are those that have buckled above 1 particle width $\sigma$.

**S13.** MD simulations of a monolayer of passive, polydisperse spherocylinders subjected to opposing 1D body forces along the $\pm x^1$ directions. There is a shear stress generated at the interfaces. The red arrows display the local velocity. The colors indicate the magnitude of the smaller eigenvalue, $\nu_{\mathrm{min}}$. White circles indicate instances when a particle buckles above 1 particle width $\sigma$.

**S14.** MD simulations of a monolayer of active, polydisperse spherocylinders for $Pe = U_0\tau_{\mathrm{R}}/\sigma = 5$ and cell-substrate adhesion $E_{\mathrm{ad}}\sigma^4/(k_{\mathrm{B}}T) = 200$. Red particles are those that have buckled above 1 particle width $\sigma$.

**S15.** MD simulations of a monolayer of active, polydisperse spherocylinders for $Pe = U_0\tau_{\mathrm{R}}/\sigma = 5$ and cell-substrate adhesion $E_{\mathrm{ad}}\sigma^4/(k_{\mathrm{B}}T) = 200$. The red arrows display the local velocity. The color map indicate the magnitude of the smaller eigenvalue, $\nu_{\mathrm{min}}\tau_{\mathrm{R}}$. White circles indicate instances when a particle buckles above 1 particle width $\sigma$.

**S16.** MD simulations of a monolayer of active, polydisperse spherocylinders for $Pe = U_0\tau_{\mathrm{R}}/\sigma = 7$ and cell-substrate adhesion $E_{\mathrm{ad}}\sigma^4/(k_{\mathrm{B}}T) = 200$. The red arrows display the local velocity. The color map indicate the magnitude of the smaller eigenvalue, $\nu_{\mathrm{min}}\tau_{\mathrm{R}}$. White circles indicate instances when a particle buckles above 1 particle width $\sigma$. Buckling events are more frequent at larger activities.

**S17.** Fluorescence microscopy timelapse of motile *P. aeruginosa* colony, same as SI Movie S2. The red arrows display the local velocity.

**S18.** Fluorescence microscopy timelapse of motile *P. aeruginosa* colony, same as SI Movie S2, capturing instances of buckling due to shear flow. The red arrows display the local velocity. The colors indicate the magnitude of the smaller eigenvalue, $\nu_{\mathrm{min}}$ [min$^{-1}$]. White circles indicate instances when a particle buckles into the second confocal slice.

**S19.** MD simulations of a monolayer of active, polydisperse spherocylinders for $Pe = U_0\tau_{\mathrm{R}}/\sigma = 5$ and cell-substrate adhesion $E_{\mathrm{ad}}\sigma^4/(k_{\mathrm{B}}T) = 200$. The color map indicates the orientation of the particle relative to a fixed reference frame. White circles indicate instances when a particle buckles above 1 particle width $\sigma$.

**S20.** Fluorescence microscopy timelapse of motile *P. aeruginosa* colony, overlayed with a color indicating the orientation of the bacterium relative to a fixed reference frame.

**S21.** Wild type colonies exhibit swarming expansion, where we observe collective flocking of bacteria. Green colors are the bacteria (expressing GFP from a plasmid), and red colors are the DNA dye SYTOX Orange Nucleic Acid Stain. When a cell dies and lyses open, DNA spills into the surrounding. We notice that extracellular DNA gets entangled, stretched, and mixed within the motile colony.

**S22.** DNase-treated colonies exhibit swarming expansion that is different from untreated colonies. In DNase-treated colonies, there is no persistent flocking of groups of bacteria. As a result, there are no significant in-plane shear stresses generated within the colony, and we observe no active buckling. Green colors are the bacteria (expressing GFP from a plasmid), and red colors are the DNA dye SYTOX Orange Nucleic Acid Stain. When a cell dies and lyses open, DNA spills into the surrounding. We notice that extracellular DNA gets quickly lysed due to DNase activity.

# References

1. Yan, J. *et al.* Mechanical instability and interfacial energy drive biofilm morphogenesis. *eLife* **8,** e43920 (2019).
2. Beroz, F. *et al.* Verticalization of bacterial biofilms. *Nature Physics* **14,** 954 (2018).
3. You, Z., Pearce, D. J., Sengupta, A. & Giomi, L. Mono-to-multilayer transition in growing bacterial colonies. *arXiv:1811.08875* (2018).
4. Dell'Arciprete, D. *et al.* A growing bacterial colony in two dimensions as an active nematic. *Nature Communications* **9,** 4190 (2018).
5. Grant Matthew, A. A., Wacław, B., Allen Rosalind, J. & Cicuta, P. The role of mechanical forces in the planar-to-bulk transition in growing Escherichia coli microcolonies. *Journal of The Royal Society Interface* **11,** 20140400 (2014).
6. Boyer, D. *et al.* Buckling instability in ordered bacterial colonies. *Physical Biology* **8,** 026008 (2011).
7. Farrell, F. D. C., Hallatschek, O., Marenduzzo, D. & Waclaw, B. Mechanically driven growth of quasi-two-dimensional microbial colonies. *Physical Review Letters* **111,** 168101 (2013).
8. Berthier, L. Trend: Dynamic heterogeneity in amorphous materials. *Physics* **4,** 42 (2011).
9. Weeks, E. R., Crocker, J. C., Levitt, A. C., Schofield, A. & Weitz, D. A. Three-dimensional direct imaging of structural relaxation near the colloidal glass transition. *Science* **287,** 627–631 (2000).
10. Keys, A. S., Hedges, L. O., Garrahan, J. P., Glotzer, S. C. & Chandler, D. Excitations are localized and relaxation is hierarchical in glass-forming liquids. *Physical Review X* **1,** 021013 (2011).
11. Kob, W., Donati, C., Plimpton, S. J., Poole, P. H. & Glotzer, S. C. Dynamical heterogeneities in a supercooled Lennard-Jones liquid. *Physical Review Letters* **79,** 2827 (1997).
12. Dauchot, O., Marty, G. & Biroli, G. Dynamical heterogeneity close to the jamming transition in a sheared granular material. *Physical Review Letters* **95,** 265701 (2005).
13. Berthier, L. & Biroli, G. Theoretical perspective on the glass transition and amorphous materials. *Reviews of Modern Physics* **83,** 587–645 (2011).
14. Chandler, D. & Garrahan, J. P. Dynamics on the way to forming glass: Bubbles in space-time. *Annual Review of Physical Chemistry* **61,** 191–217 (2010).
15. Binder, K. & Kob, W. *Glassy materials and disordered solids: An introduction to their statistical mechanics* (World scientific, 2011).
16. Berthier, L., Biroli, G., Bouchaud, J.-P., Cipelletti, L. & van Saarloos, W. *Dynamical heterogeneities in glasses, colloids, and granular media* (Oxford University Press, 2011).
17. Biroli, G. & Garrahan, J. P. Perspective: The glass transition. *The Journal of Chemical Physics* **138,** 12A301 (2013).

18. Donati, C. *et al.* Stringlike cooperative motion in a supercooled liquid. *Physical Review Letters* **80,** 2338–2341 (1998).

19. Glotzer, S. C. Spatially heterogeneous dynamics in liquids: insights from simulation. *Journal of Non-Crystalline Solids* **274,** 342–355 (2000).

20. Particle dynamics and the development of string-like motion in a simulated monoatomic supercooled liquid. *The Journal of Chemical Physics* **120,** 4415–4427 (2004).

21. Candelier, R. *et al.* Spatiotemporal hierarchy of relaxation events, dynamical heterogeneities, and structural reorganization in a supercooled liquid. *Physical Review Letters* **105,** 135702 (2010).

22. Garrahan, J. P. & Chandler, D. Geometrical explanation and scaling of dynamical heterogeneities in glass forming systems. *Physical Review Letters* **89,** 035704. ISSN: 0031-9007 (July 2002).

23. Elmatad, Y. S., Chandler, D. & Garrahan, J. P. Corresponding states of structural glass formers. *The Journal of Physical Chemistry B* **113,** 5563–5567 (2009).

24. Elmatad, Y. S., Chandler, D. & Garrahan, J. P. Corresponding states of structural glass formers. II. *The Journal of Physical Chemistry B* **114,** 17113–17119 (2010).

25. Katira, S., Garrahan, J. P. & Mandadapu, K. K. Theory for glassy behavior of supercooled liquid mixtures. *arXiv:1903.08557* (2019).

26. Keys, A. S., Garrahan, J. P. & Chandler, D. Calorimetric glass transition explained by hierarchical dynamic facilitation. *Proceedings of the National Academy of Sciences* **110,** 4482–4487 (2013).

27. Isobe, M., Keys, A. S., Chandler, D. & Garrahan, J. P. Applicability of dynamic facilitation theory to binary hard disk systems. *Physical Review Letters* **117,** 145701 (2016).

28. Garrahan, J. P. & Chandler, D. Coarse-grained microscopic model of glass formers. *Proceedings of the National Academy of Sciences* **100,** 9710 (2003).

29. Jäckle, J. & Eisinger, S. A hierarchically constrained kinetic Ising model. *Zeitschrift für Physik B Condensed Matter* **84,** 115–124 (1991).

30. Sollich, P. & Evans, M. R. Glassy time-scale divergence and anomalous coarsening in a kinetically constrained spin chain. *Physical Review Letters* **83,** 3238–3241 (1999).

31. Sollich, P. & Evans, M. R. Glassy dynamics in the asymmetrically constrained kinetic Ising chain. *Physical Review E* **68,** 031504 (2003).

32. Ritort, F. & Sollich, P. Glassy dynamics of kinetically constrained models. *Advances in Physics* **52,** 219–342 (2003).

33. Aldous, D. & Diaconis, P. The asymmetric one-dimensional constrained Ising model: Rigorous results. *Journal of Statistical Physics* **107,** 945–975 (2002).

34. Chleboun, P., Faggionato, A. & Martinelli, F. The influence of dimension on the relaxation process of East-like models: Rigorous results. *EPL (Europhysics Letters)* **107,** 36002 (2014).

35. Tailleur, J. & Cates, M. E. Statistical mechanics of interacting run-and-tumble bacteria. *Physical Review Letters* **100,** 218103 (2008).

36. Marchetti, M. C. *et al.* Hydrodynamics of soft active matter. *Reviews of Modern Physics* **85,** 1143–1189 (2013).

37. Cates, M. E. & Tailleur, J. When are active Brownian particles and run-and-tumble particles equivalent? Consequences for motility-induced phase separation. *Europhys Lett* **101,** 20010 (2013).

38. Ramaswamy, S. The mechanics and statistics of active matter. *Annual Review of Condense Matter Physics* **1,** 323–345 (2010).

39. Lauga, E. & Powers, T. R. The hydrodynamics of swimming microorganisms. *Reports on Progress in Physics* **72,** 096601 (2009).

40. Takatori, S. C., Yan, W. & Brady, J. F. Swim pressure: stress generation in active matter. *Physical Review Letters* **113,** 028103 (2014).

41. Yang, X., Manning, M. L. & Marchetti, M. C. Aggregation and segregation of confined active particles. *Soft Matter* **10,** 6477–6484 (2014).

42. Solon, A. P. *et al.* Pressure and phase equilibria in interacting active Brownian spheres. *Physical Review Letters* **114,** 198301 (2015).

43. Ezhilan, B., Alonso-Matilla, R. & Saintillan, D. On the distribution and swim pressure of run-and-tumble particles in confinement. *Journal of Fluid Mechanics* **781,** R4 (2015).

44. Yan, W. & Brady, J. F. The swim force as a body force. *Soft Matter* **11,** 6235–6244 (2015).

45. Epstein, J. M., Klymko, K. & Mandadapu, K. K. Statistical mechanics of transport processes in active fluids. II. Equations of hydrodynamics for active Brownian particles. *The Journal of Chemical Physics* **150,** 164111 (2019).

46. Nandi, S. K. *et al.* A random first-order transition theory for an active glass. *Proceedings of the National Academy of Sciences* **115,** 7688 (2018).

47. Kearns, D. B. A field guide to bacterial swarming motility. *Nature Reviews Microbiology* **8,** 634 (2010).

48. Rashid, M. H. & Kornberg, A. Inorganic polyphosphate is needed for swimming, swarming, and twitching motilities of *Pseudomonas aeruginosa. Proceedings of the National Academy of Sciences* **97,** 4885–4890 (2000).

49. Gloag, E. S. *et al.* Self-organization of bacterial biofilms is facilitated by extracellular DNA. *Proceedings of the National Academy of Sciences* **110,** 11541 (2013).

50. Verstraeten, N. *et al.* Living on a surface: swarming and biofilm formation. *Trends in microbiology* **16,** 496–506 (2008).

51. Lovely, P. S. & Dahlquist, F. W. Statistical measures of bacterial motility and chemotaxis. *Journal of Theoretical Biology* **50,** 477–496 (1975).

52. Heyes, D. & Melrose, J. Brownian dynamics simulations of model hard-sphere suspensions. *Journal of non-newtonian fluid mechanics* **46,** 1–28 (1993).

53. Berthier, L., Flenner, E. & Szamel, G. How active forces influence nonequilibrium glass transitions. *New Journal of Physics* **19,** 125006 (2017).

54. Ni, R., Stuart, M. A. C. & Dijkstra, M. Pushing the glass transition towards random close packing using self-propelled hard spheres. *Nature Communications* **4,** 2704 (2013).
55. Berthier, L. & Kurchan, J. Non-equilibrium glass transitions in driven and active matter. *Nature Physics* **9,** 310–314 (2013).
56. Isa, L., Besseling, R. & Poon, W. C. K. Shear zones and wall slip in the capillary flow of concentrated colloidal suspensions. *Physical Review Letters* **98,** 198305 (2007).
57. Petekidis, G., Vlassopoulos, D. & Pusey, P. N. Yielding and flow of sheared colloidal glasses. *Journal of Physics: Condensed Matter* **16,** S3955–S3963 (2004).
58. Lin, J. & Wyart, M. Microscopic processes controlling the Herschel-Bulkley exponent. *Physical Review E* **97,** 012603 (2018).
59. Weeks, J. D., Chandler, D. & Andersen, H. C. Role of repulsive forces in determining the equilibrium structure of simple liquids. *Journal of Chemical Physics* **54,** 5237–5247 (1971).
60. Glaser, J. *et al.* Strong scaling of general-purpose molecular dynamics simulations on GPUs. *Computer Physics Communications* **192,** 97–107 (2015).
61. Anderson, J. A., Lorenz, C. D. & Travesset, A. General purpose molecular dynamics simulations fully implemented on graphics processing units. *Journal of Computational Physics* **227,** 5342–5359 (2008).
62. Nguyen, T. D., Phillips, C. L., Anderson, J. A. & Glotzer, S. C. Rigid body constraints realized in massively-parallel molecular dynamics on graphics processing units. *Computer Physics Communications* **182,** 2307–2313 (2011).
63. Mishra, C. K., Hima Nagamanasa, K., Ganapathy, R., Sood, A. K. & Gokhale, S. Dynamical facilitation governs glassy dynamics in suspensions of colloidal ellipsoids. *Proceedings of the National Academy of Sciences of the United States of America* **111,** 15362–15367 (2014).
64. Zheng, Z., Wang, F. & Han, Y. Glass transitions in quasi-two-dimensional suspensions of colloidal ellipsoids. *Physical Review Letters* **107,** 065702 (2011).
65. Stenhammar, J., Marenduzzo, D., Allen, R. J. & Cates, M. E. Phase behaviour of active Brownian particles: the role of dimensionality. *Soft Matter* **10,** 1489–1499 (2014).
66. Stylianidou, S., Brennan, C., Nissen, S. B., Kuwada, N. J. & Wiggins, P. A. SuperSegger: robust image segmentation, analysis and lineage tracking of bacterial cells. *Molecular microbiology* **102,** 690–700 (2016).
67. Donev, A. *Jammed packings of hard particles* PhD thesis (2006).
68. Takatori, S. C. & Brady, J. F. Towards a thermodynamics of active matter. *Physical Review E* **91,** 032117 (2015).
69. Wensink, H. H. *et al.* Meso-scale turbulence in living fluids. *Proceedings of the National Academy of Sciences* **109,** 14308 (2012).
70. Dunkel, J. *et al.* Fluid dynamics of bacterial turbulence. *Physical Review Letters* **110,** 228102 (2013).

71. Grošelj, D., Jenko, F. & Frey, E. How turbulence regulates biodiversity in systems with cyclic competition. *Physical Review E* **91,** 033009 (2015).

72. Evans, E. A. & Skalak, R. *Mechanics and thermodynamics of biomembranes* (CRC Press, Boca Raton, Fl., 1980).

73. Arroyo, M. & DeSimone, A. Relaxation dynamics of fluid membranes. *Physical Review E* **79,** 031915 (2009).

74. Sahu, A., Sauer, R. A. & Mandadapu, K. K. Irreversible thermodynamics of curved lipid membranes. *Physical Review E* **96,** 042409 (2017).

75. Rangamani, P., Agrawal, A., Mandadapu, K. K., Oster, G. & Steigmann, D. J. Interaction between surface shape and intra-surface viscous flow on lipid membranes. *Biomechanics and modeling in mechanobiology* **12,** 833–845 (2013).

76. Sahu, A., Glisman, A., Tchoufag, J. & Mandadapu, K. K. Geometry and dynamics of lipid membranes. *arXiv:1910.10693* (2019).

77. Sauer, R. A., Duong, T. X., Mandadapu, K. K. & Steigmann, D. J. A stabilized finite element formulation for liquid shells and its application to lipid bilayers. *Journal of computational physics* **330,** 436–466 (2017).

78. Omar, Y. A., Sahu, A., Sauer, R. A. & Mandadapu, K. K. Non-axisymmetric shapes of biological membranes from locally induced curvature. *bioRxiv,* 688127 (2019).

79. Sahu, A., Omar, Y. A., Sauer, R. A. & Mandadapu, K. K. Arbitrary Lagrangian–Eulerian finite element method for curved and deforming surfaces: I. General theory and application to fluid interfaces. *Journal of Computational Physics,* 109253 (2020).

80. Naghdi, P. M. *The theory of shells and plates* 425–640 (Springer Berlin Heidelberg, 1973).

81. Struik, D. J. *Lectures on classical differential geometry* (Courier Corporation, 1961).

82. Kreyszig, E. *Introduction to differential geometry and Riemannian geometry* (University of Toronto Press, 1968).

83. Bird, R. B., Stewart, W. E. & Lightfoot, E. N. *Transport phenomena* (John Wiley & Sons, 2007).

84. Leal, L. G. *Advanced transport phenomena: fluid mechanics and convective transport processes* (Cambridge University Press, 2007).

85. Evans, D. J. & Morriss, G. *Statistical mechanics of nonequilibrium liquids* (Cambridge University Press, 2008).

86. Saw, T. B. *et al.* Topological defects in epithelia govern cell death and extrusion. *Nature* **544,** 212 (2017).

87. Kawaguchi, K., Kageyama, R. & Sano, M. Topological defects control collective dynamics in neural progenitor cell cultures. *Nature* **545,** 327 (2017).

88. Bolhuis, P. & Frenkel, D. Tracing the phase boundaries of hard spherocylinders. *The Journal of Chemical Physics* **106,** 666–687 (1997).

89. Bates, M. A. & Frenkel, D. Phase behavior of two-dimensional hard rod fluids. *The Journal of Chemical Physics* **112,** 10034–10041 (2000).

90. Bautista-Carbajal, G. & Odriozola, G. Phase diagram of two-dimensional hard ellipses. *The Journal of Chemical Physics* **140,** 204502 (2014).

91. DeCamp, S. J., Redner, G. S., Baskaran, A., Hagan, M. F. & Dogic, Z. Orientational order of motile defects in active nematics. *Nature materials* **14,** 1110 (2015).

92. Copenhagen, K., Alert, R., Wingreen, N. S. & Shaevitz, J. W. Topological defects induce layer formation in Myxococcus xanthus colonies. *arXiv:2001.03804* (2020).

93. Thielicke, W. & Stamhuis, E. PIVlab–towards user-friendly, affordable and accurate digital particle image velocimetry in MATLAB. *Journal of Open Research Software* **2** (2014).

94. Lyczak, J. B., Cannon, C. L. & Pier, G. B. Establishment of Pseudomonas aeruginosa infection: lessons from a versatile opportunist. *Microbes and Infection* **2,** 1051–1060 (2000).

95. Gellatly, S. L. & Hancock, R. E. W. Pseudomonas aeruginosa : new insights into pathogenesis and host defenses. *Pathogens and Disease* **67,** 159–173 (2013).

96. Faure, E., Kwong, K. & Nguyen, D. Pseudomonas aeruginosa in Chronic Lung Infections: How to Adapt Within the Host? *Frontiers in Immunology* **9** (2018).

97. López-Causapé, C., Rojo-Molinero, E., Maciá, M. D. & Oliver, A. The problems of antibiotic resistance in cystic fibrosis and solutions. *Expert Review of Respiratory Medicine* **9,** 73–88 (2015).

98. Bjarnsholt, T. The role of bacterial biofilms in chronic infections. *APMIS* **121,** 1–58 (2013).

99. Whitchurch, C. B., Tolker-Nielsen, T., Ragas, P. C. & Mattick, J. S. Extracellular DNA required for bacterial biofilm formation. *Science* **295,** 1487–1487 (2002).
